# Supplementary material for: An unavoidable set of D-reducible configurations
Source: arXiv:0905.0043 ancillary file (2009-05-04)

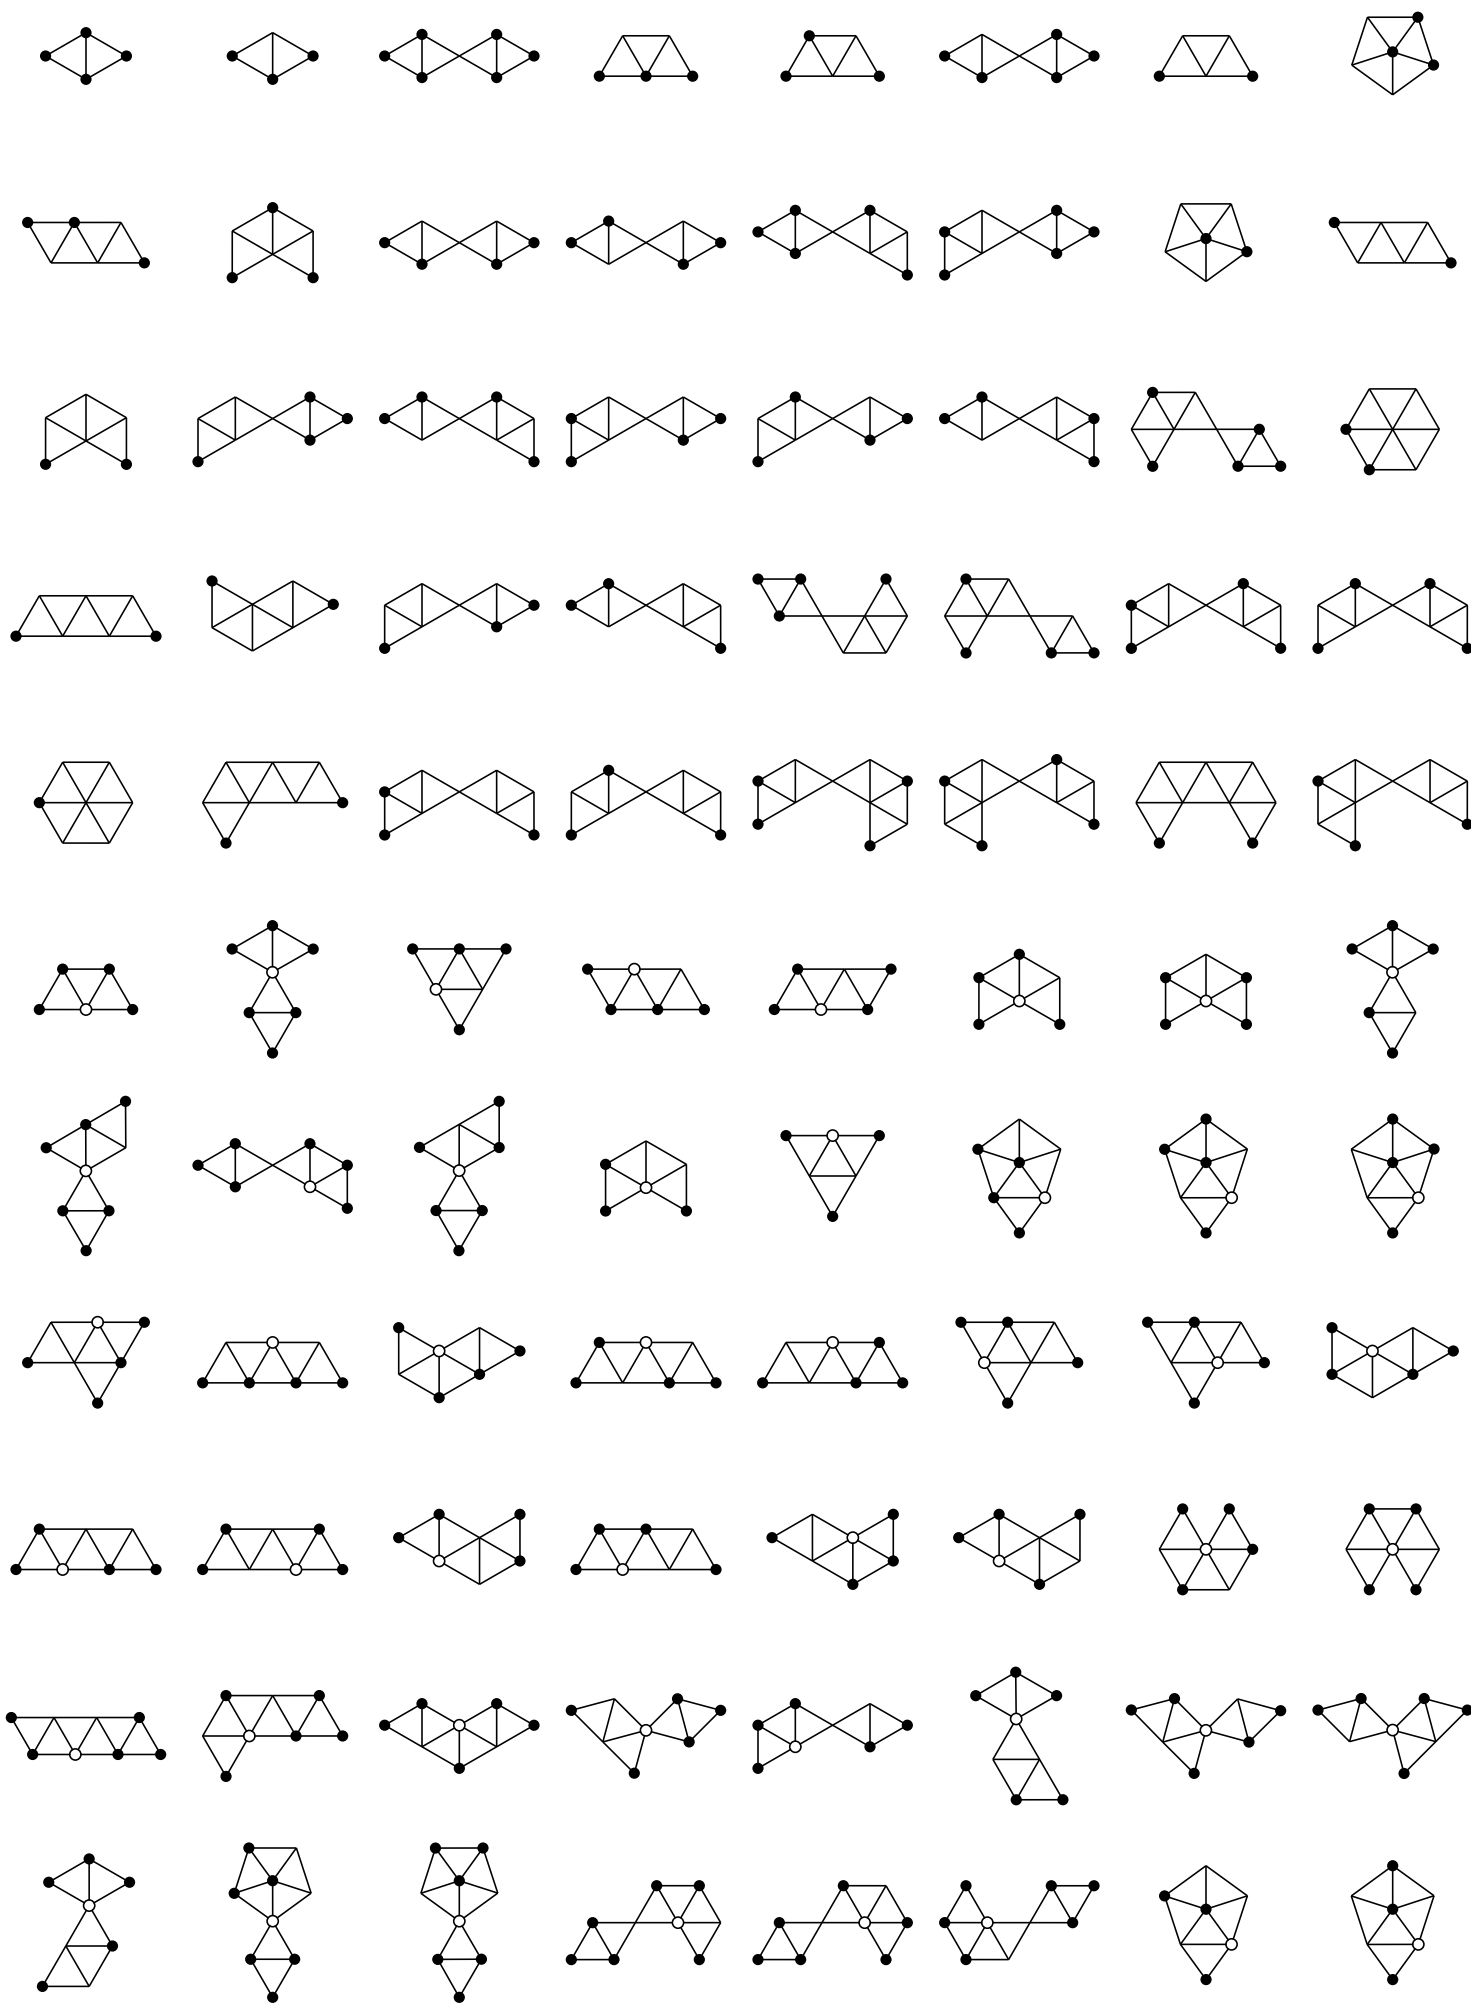

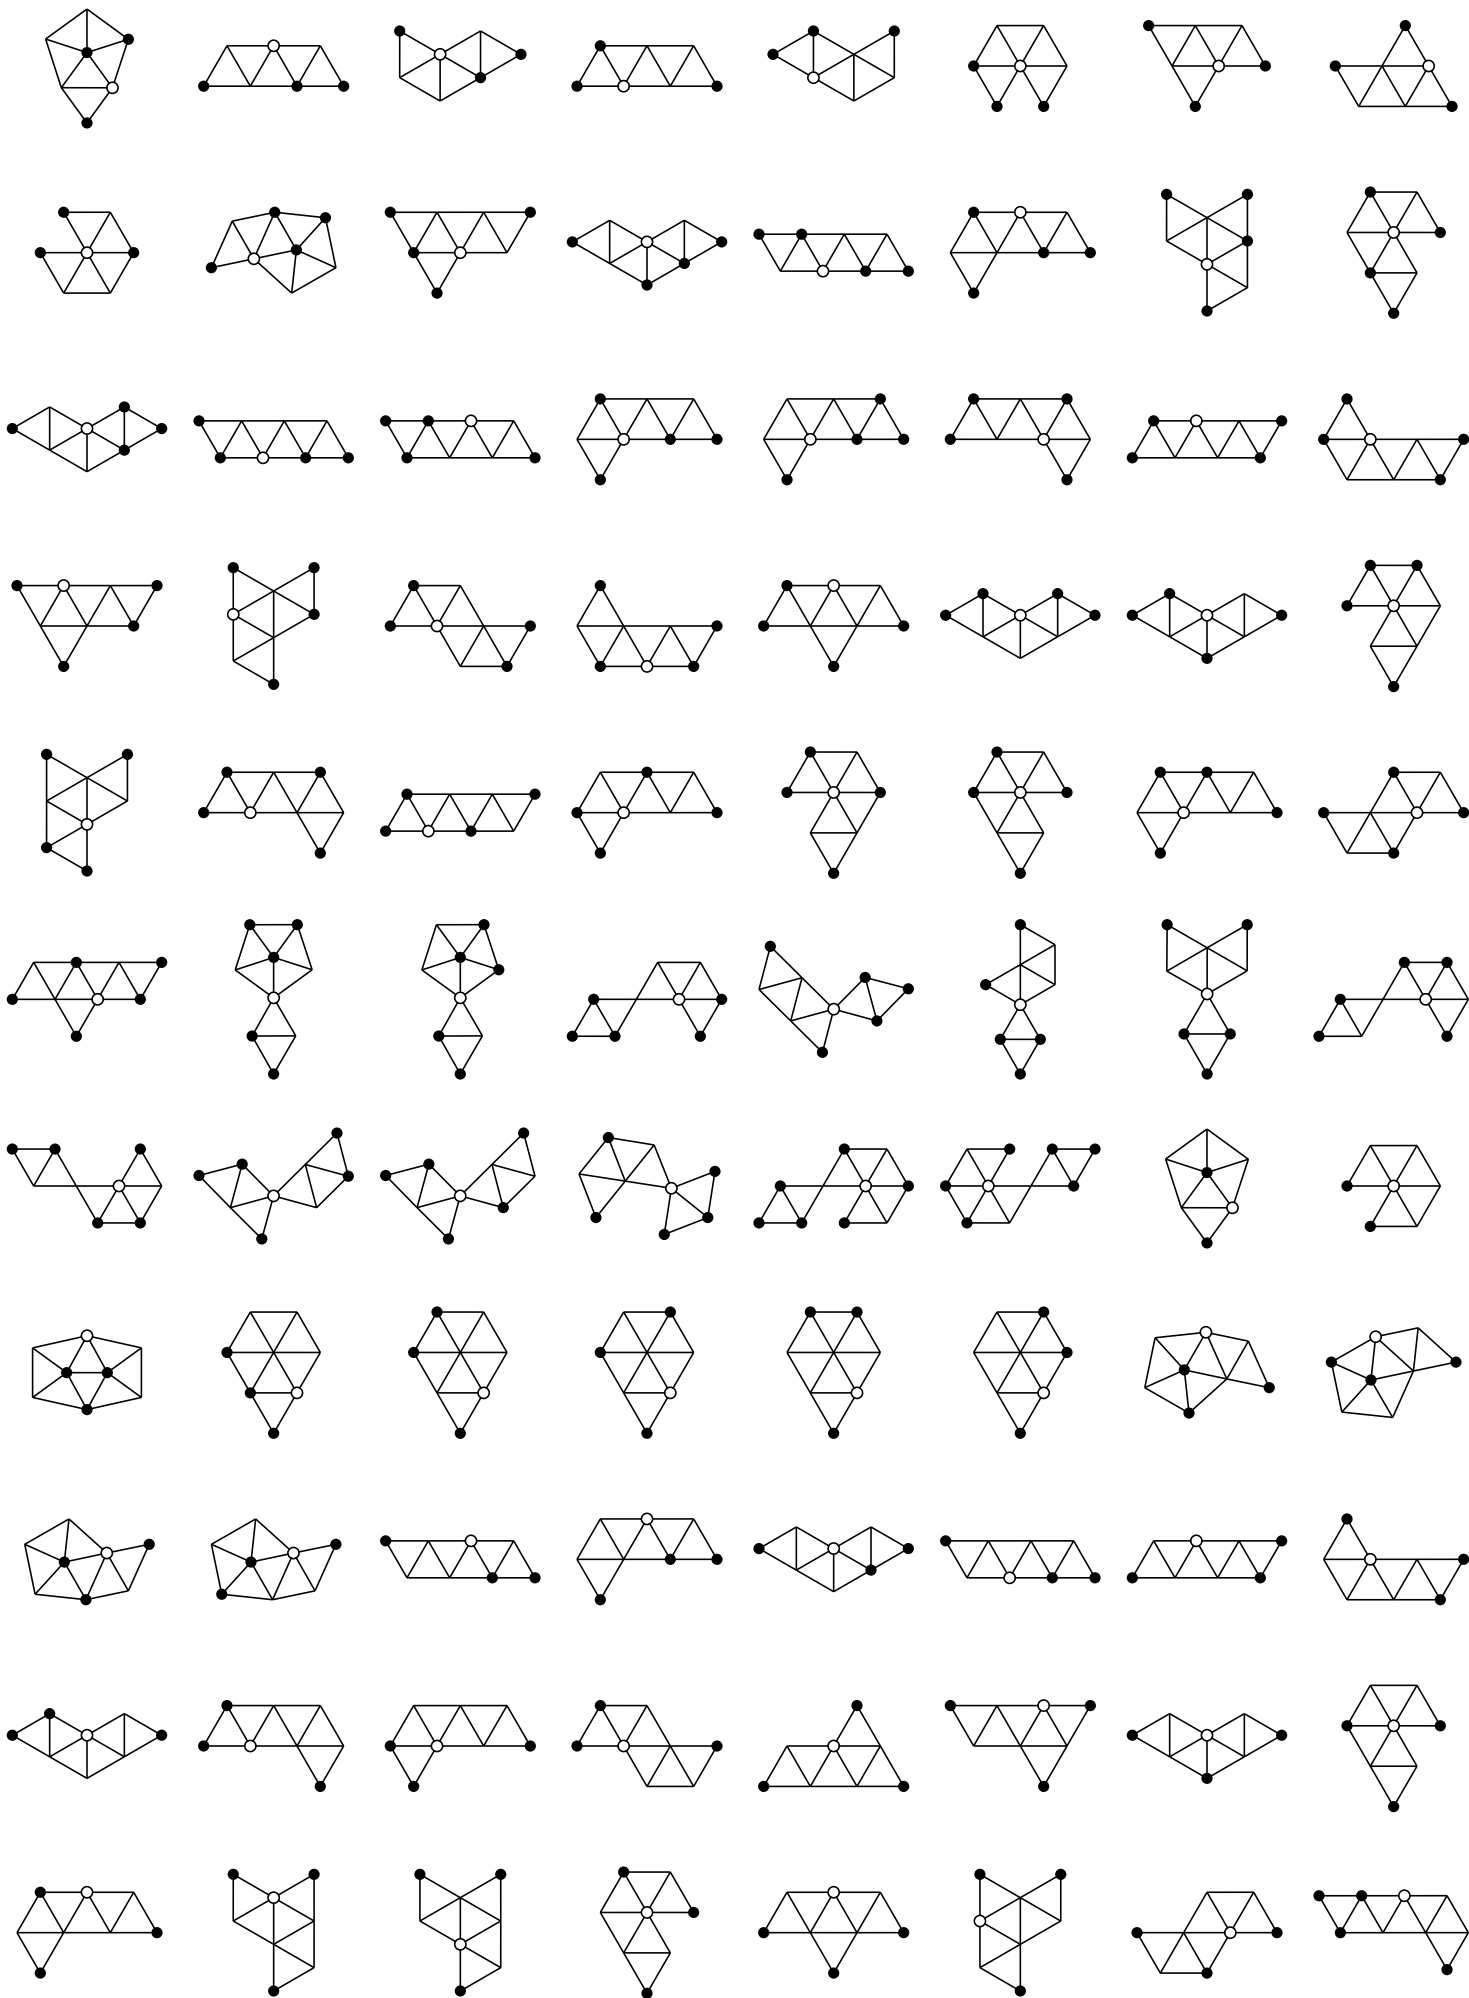

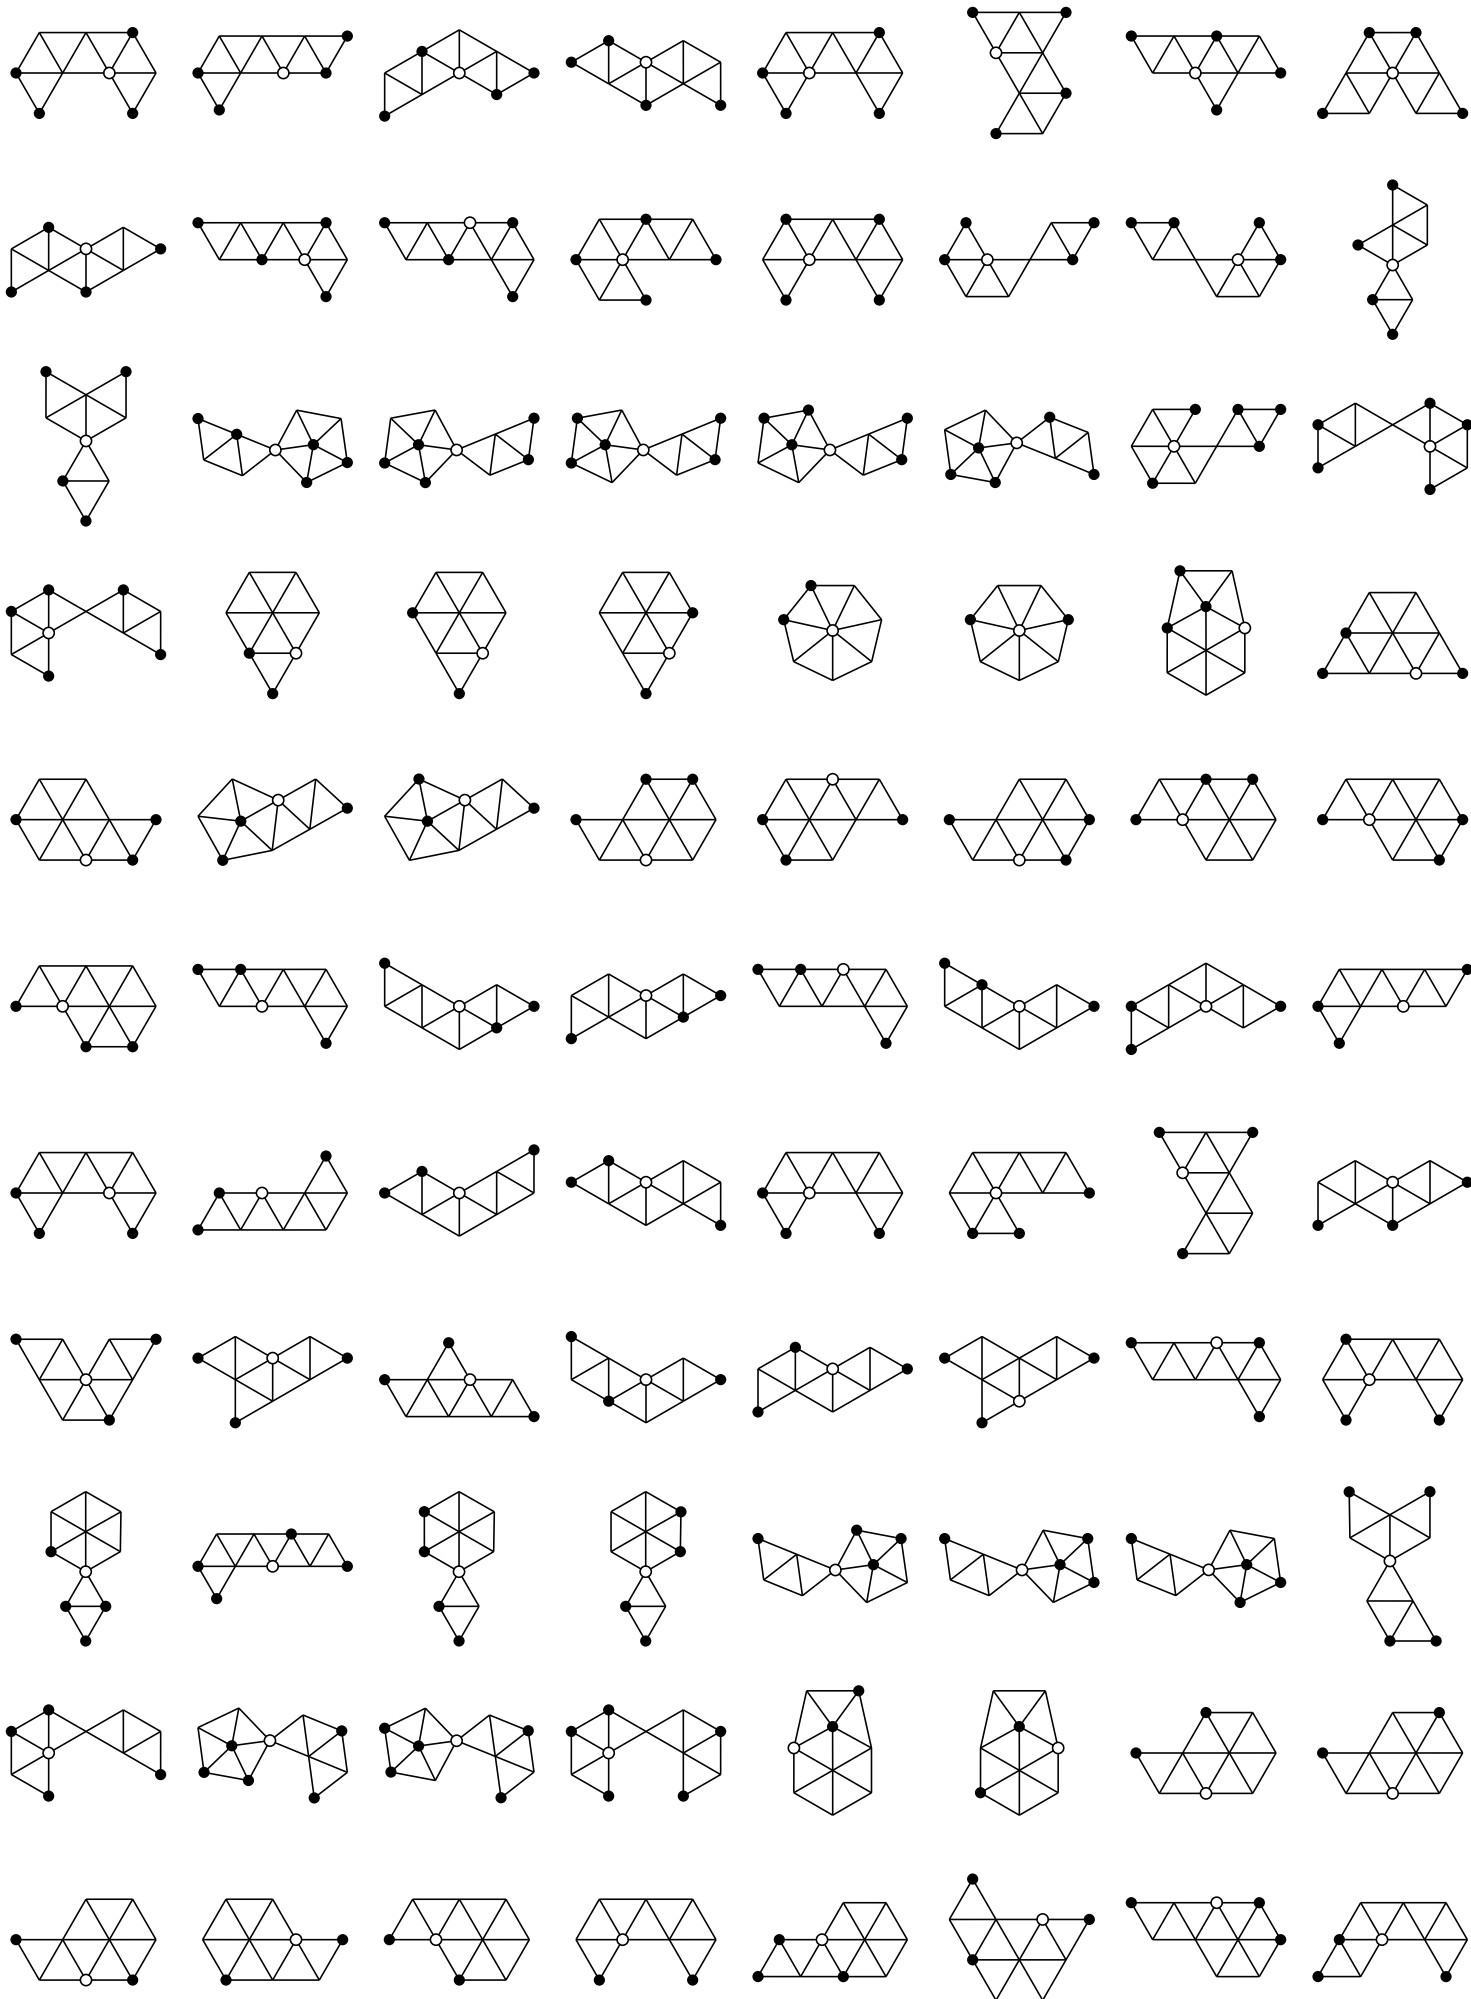

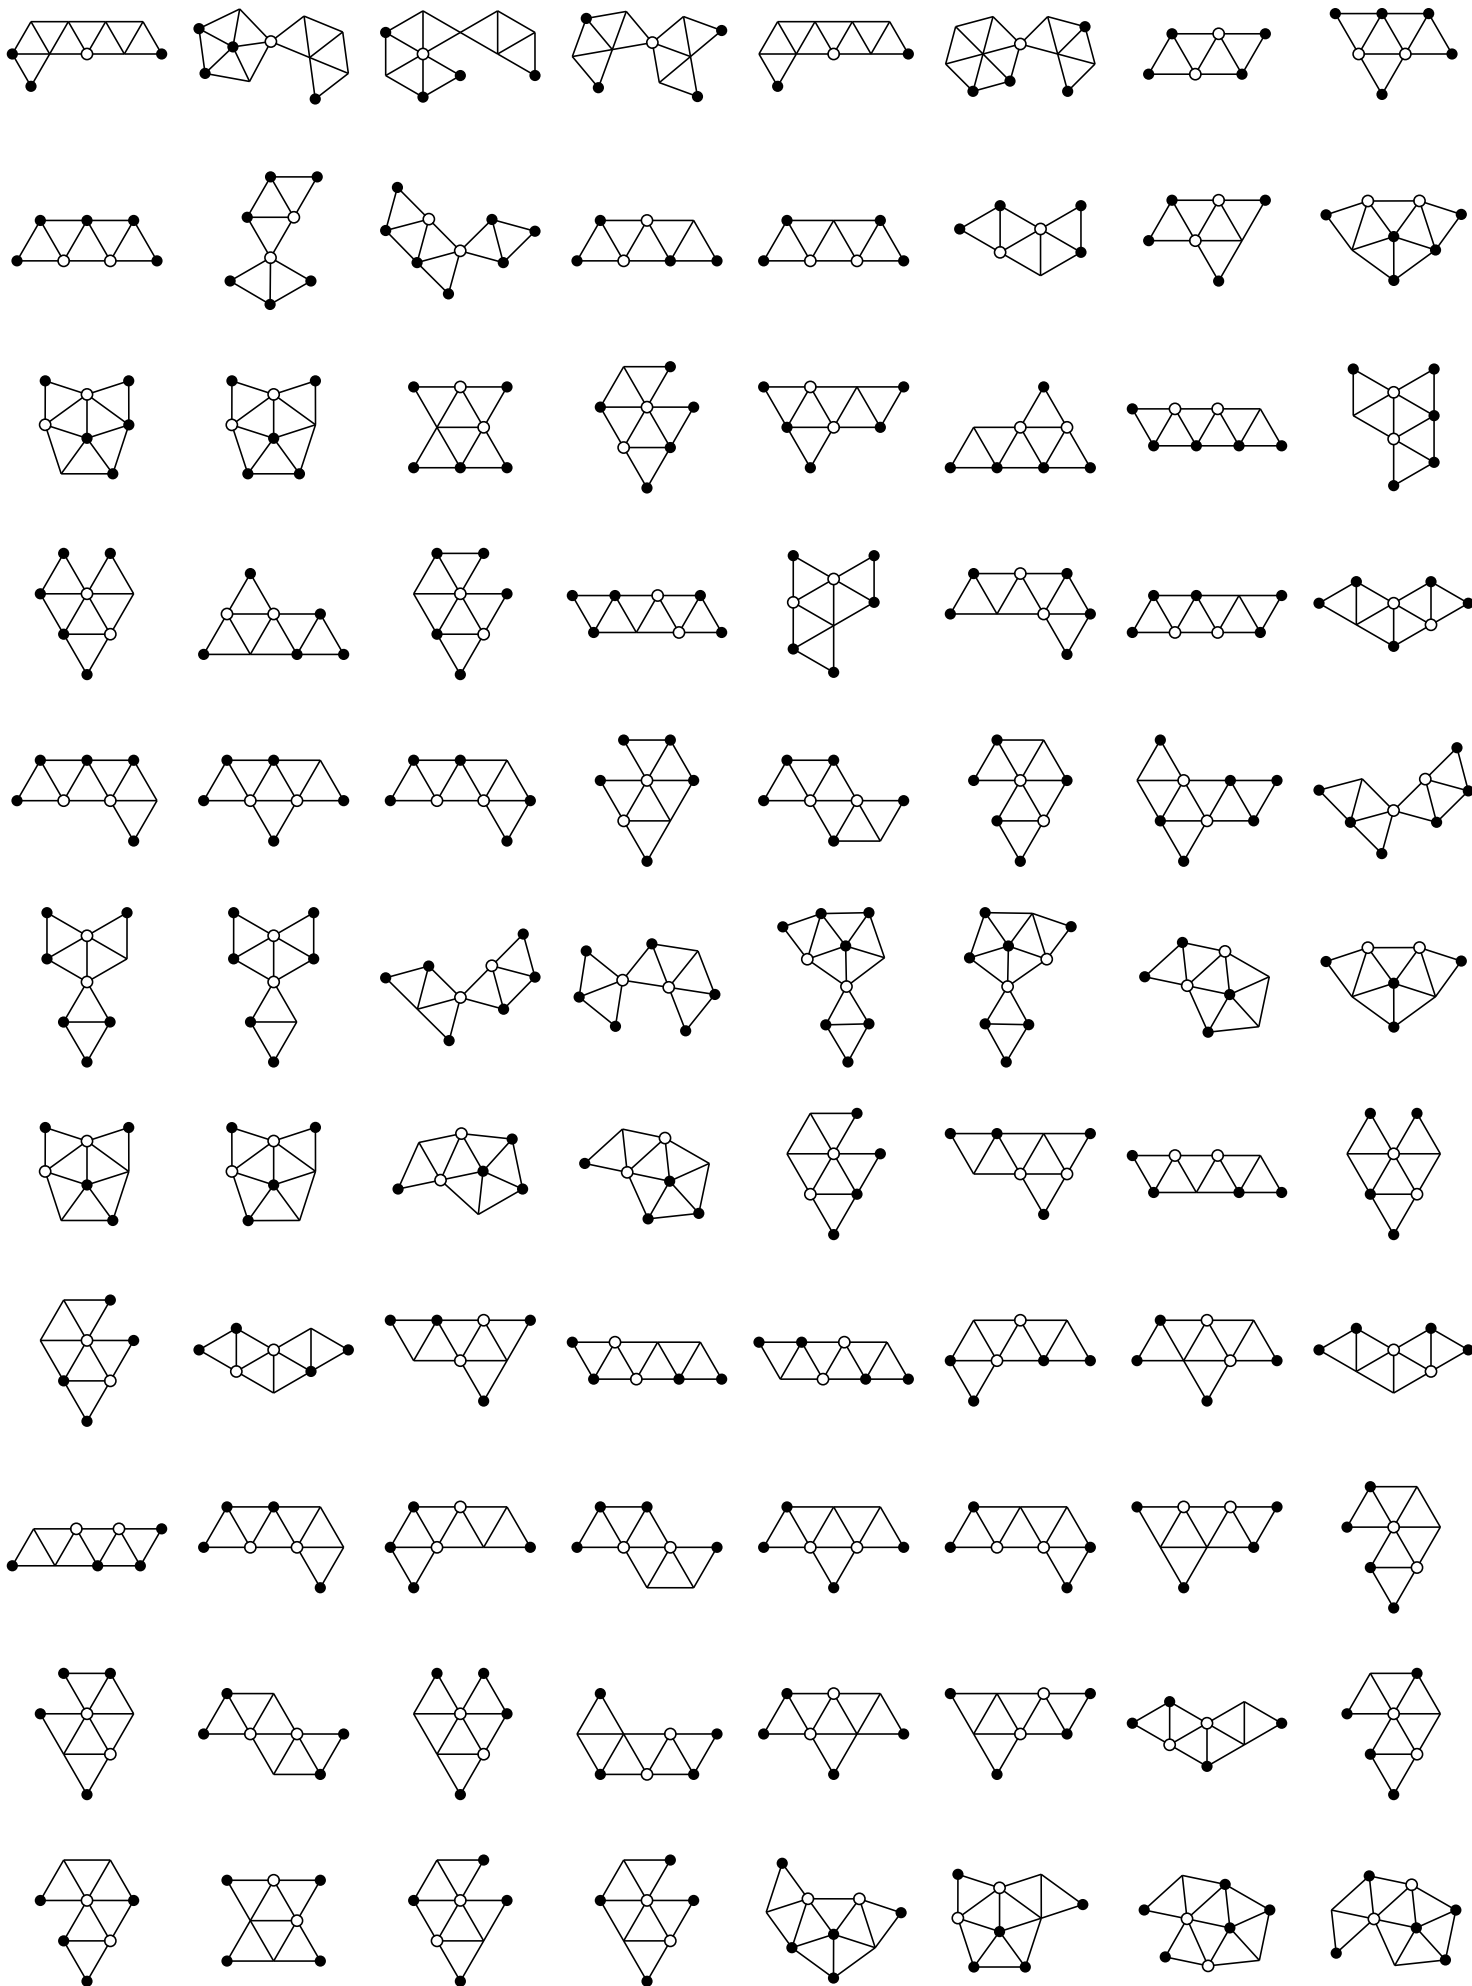

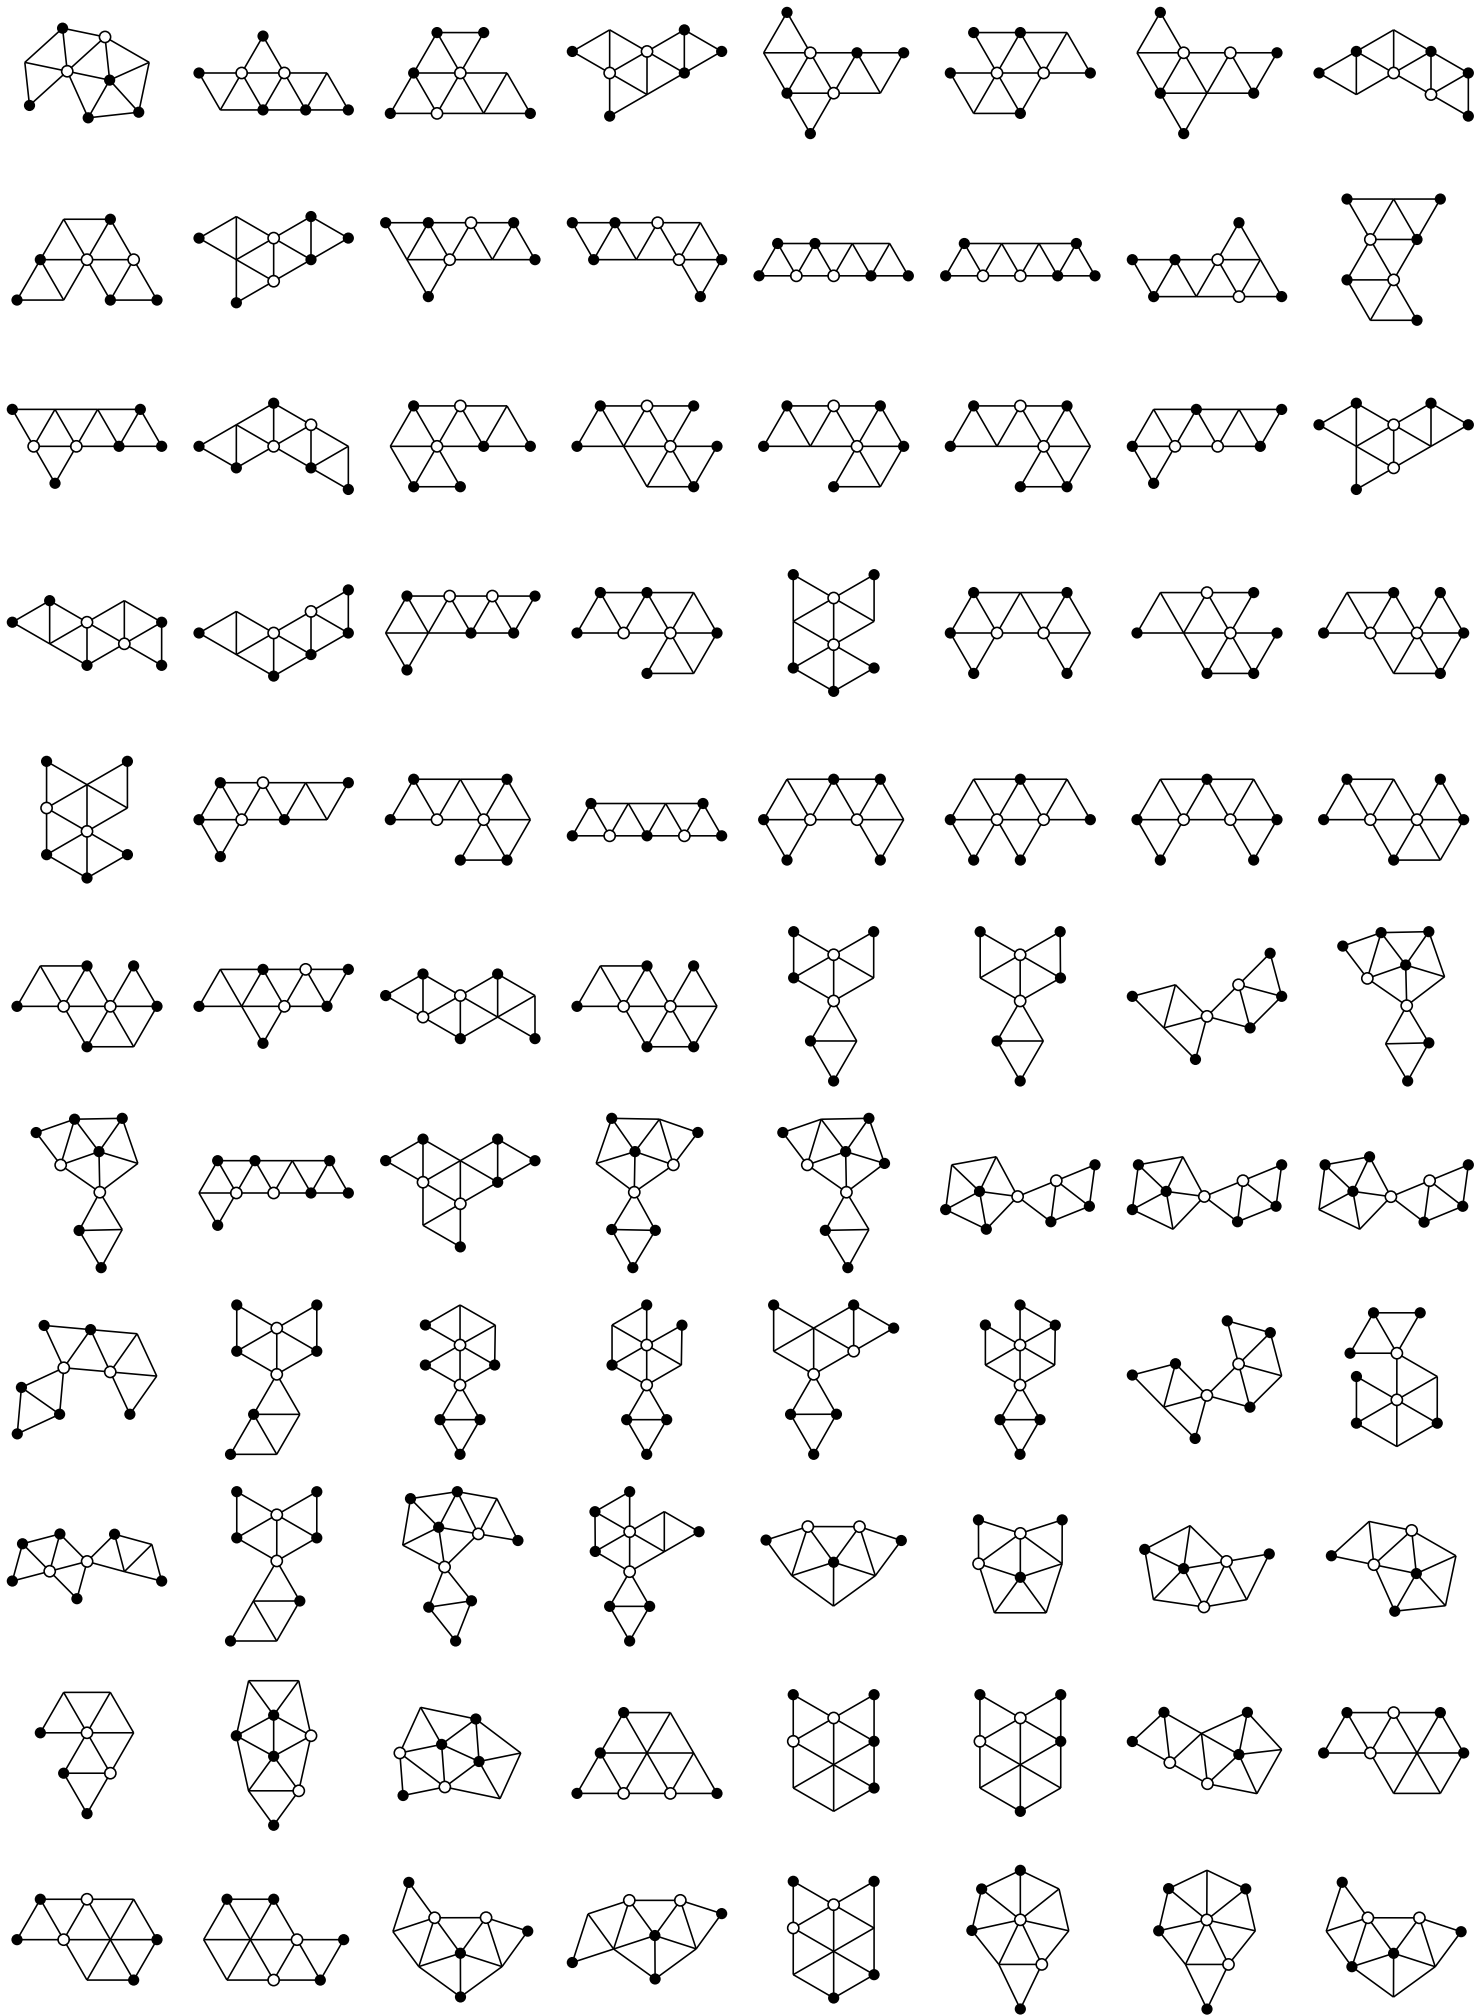

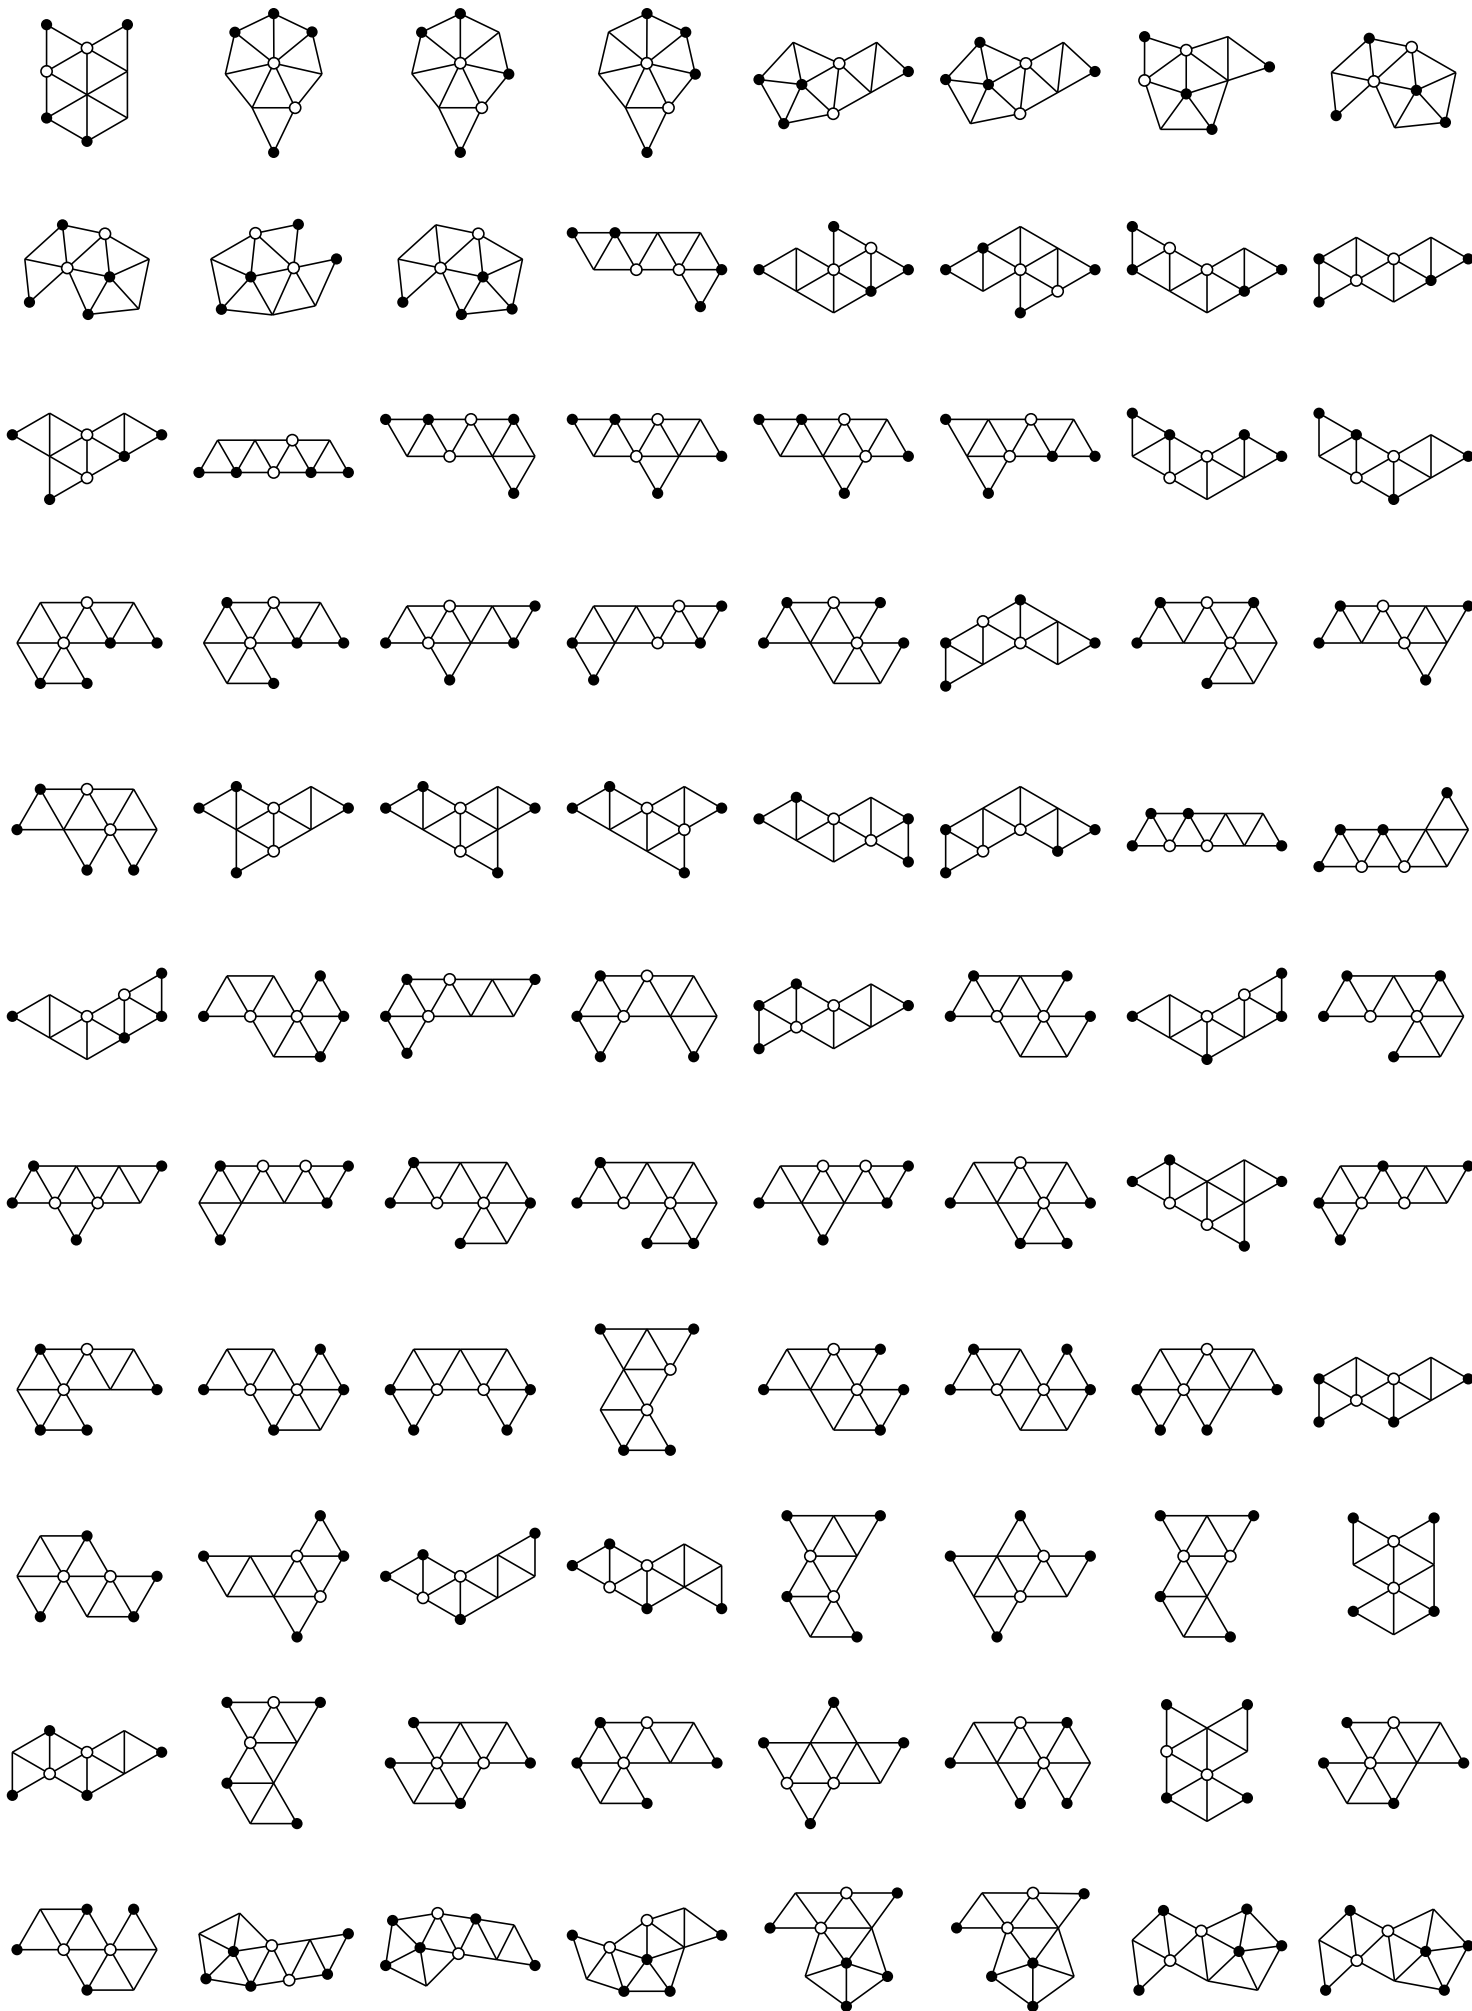

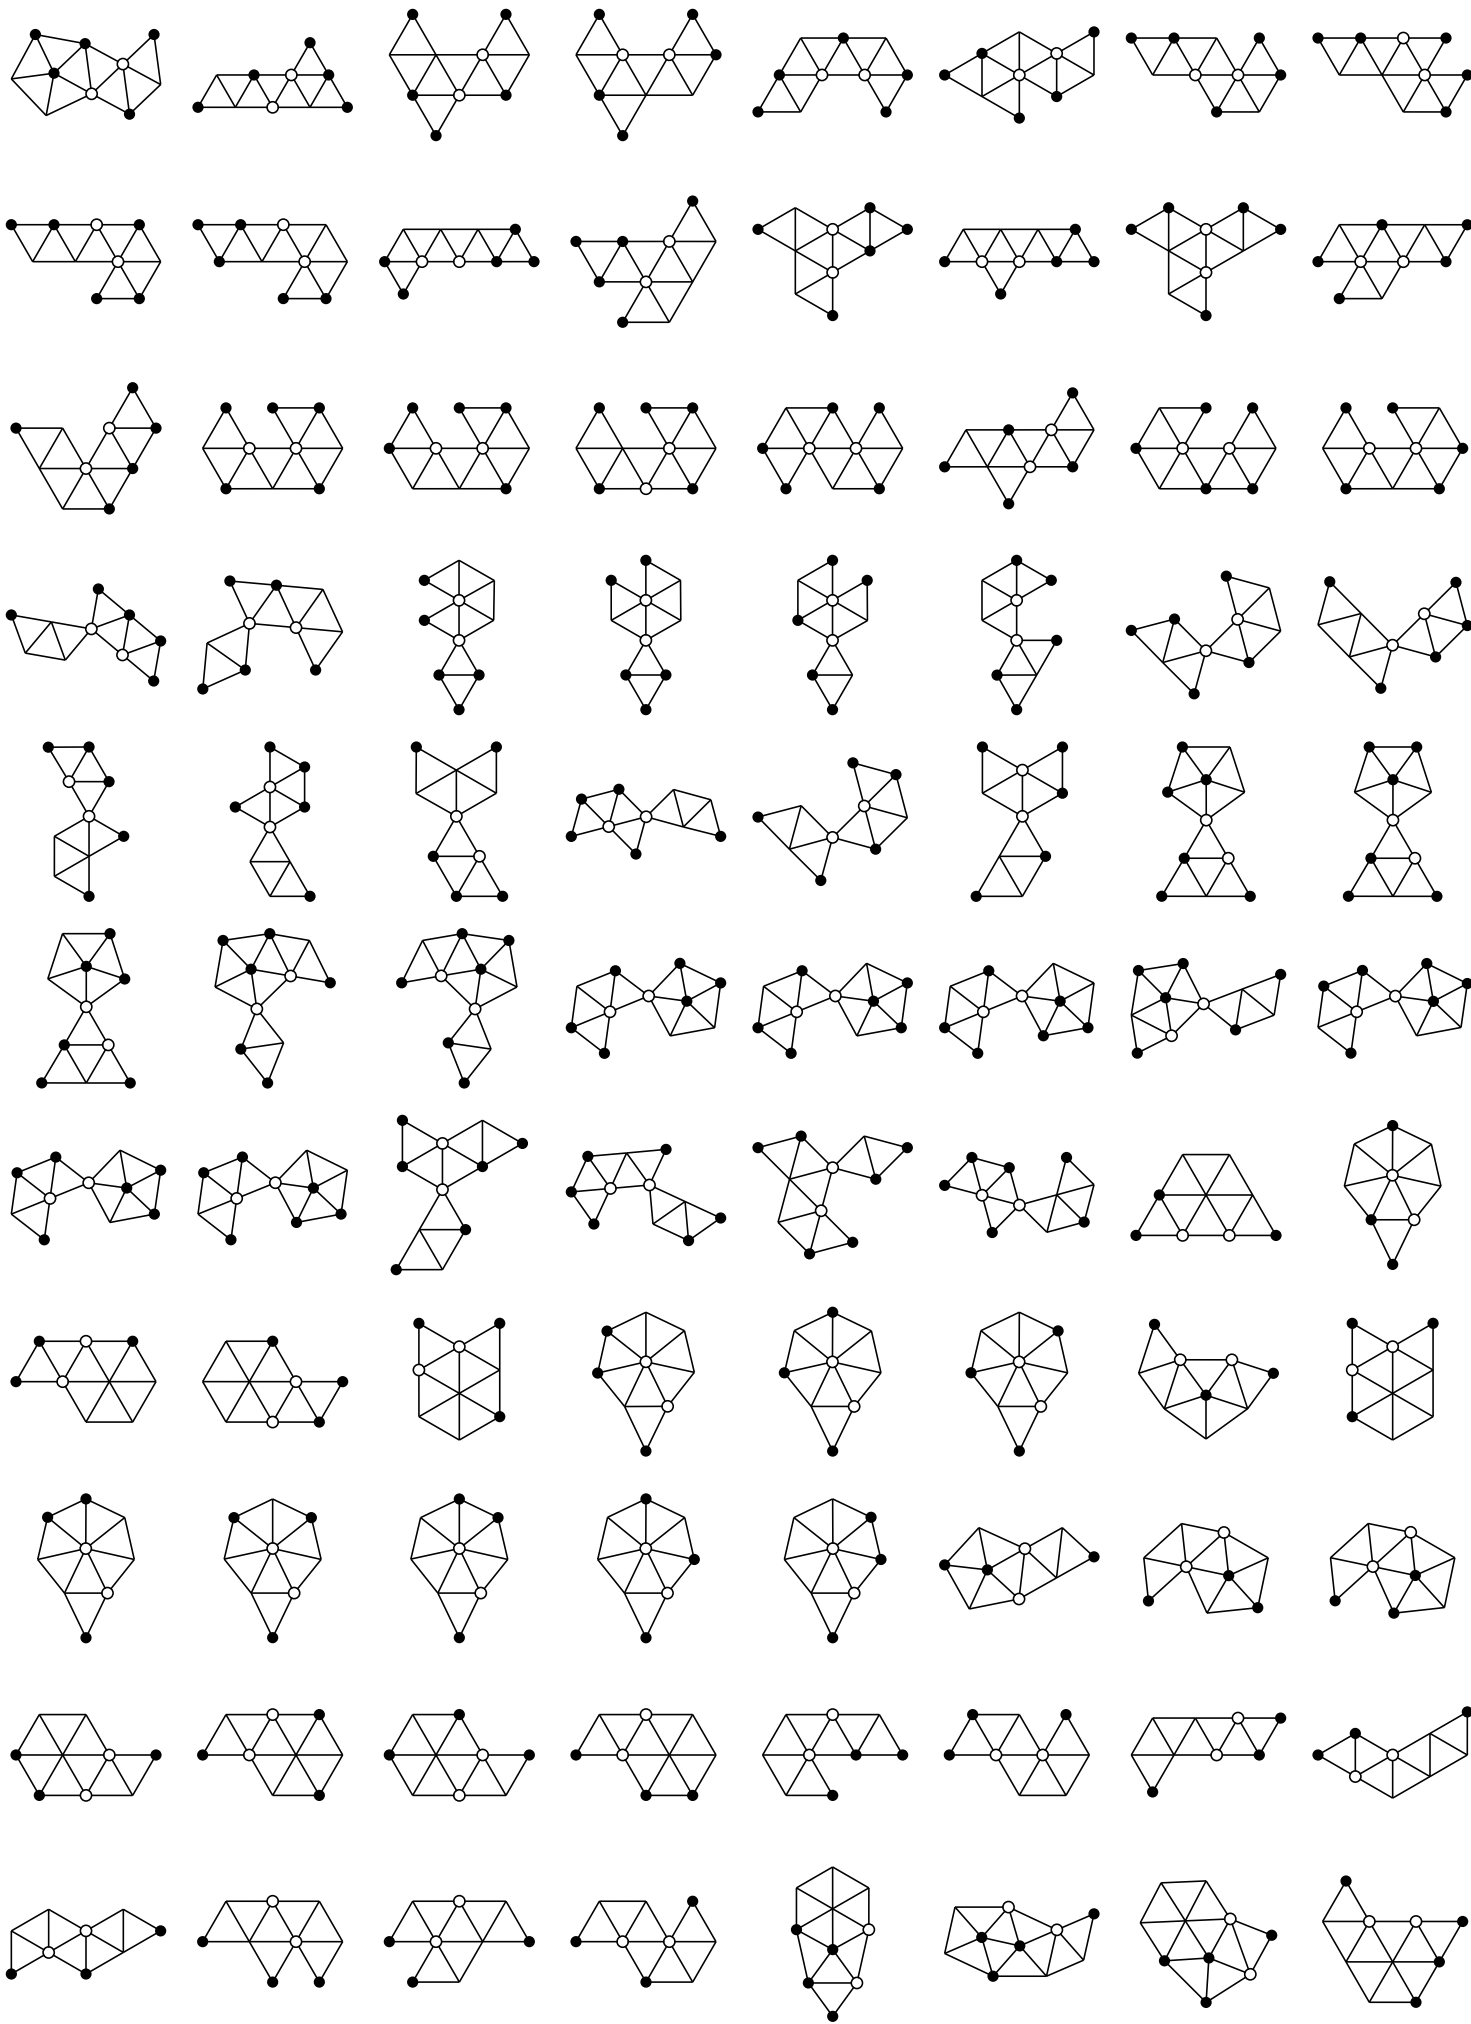

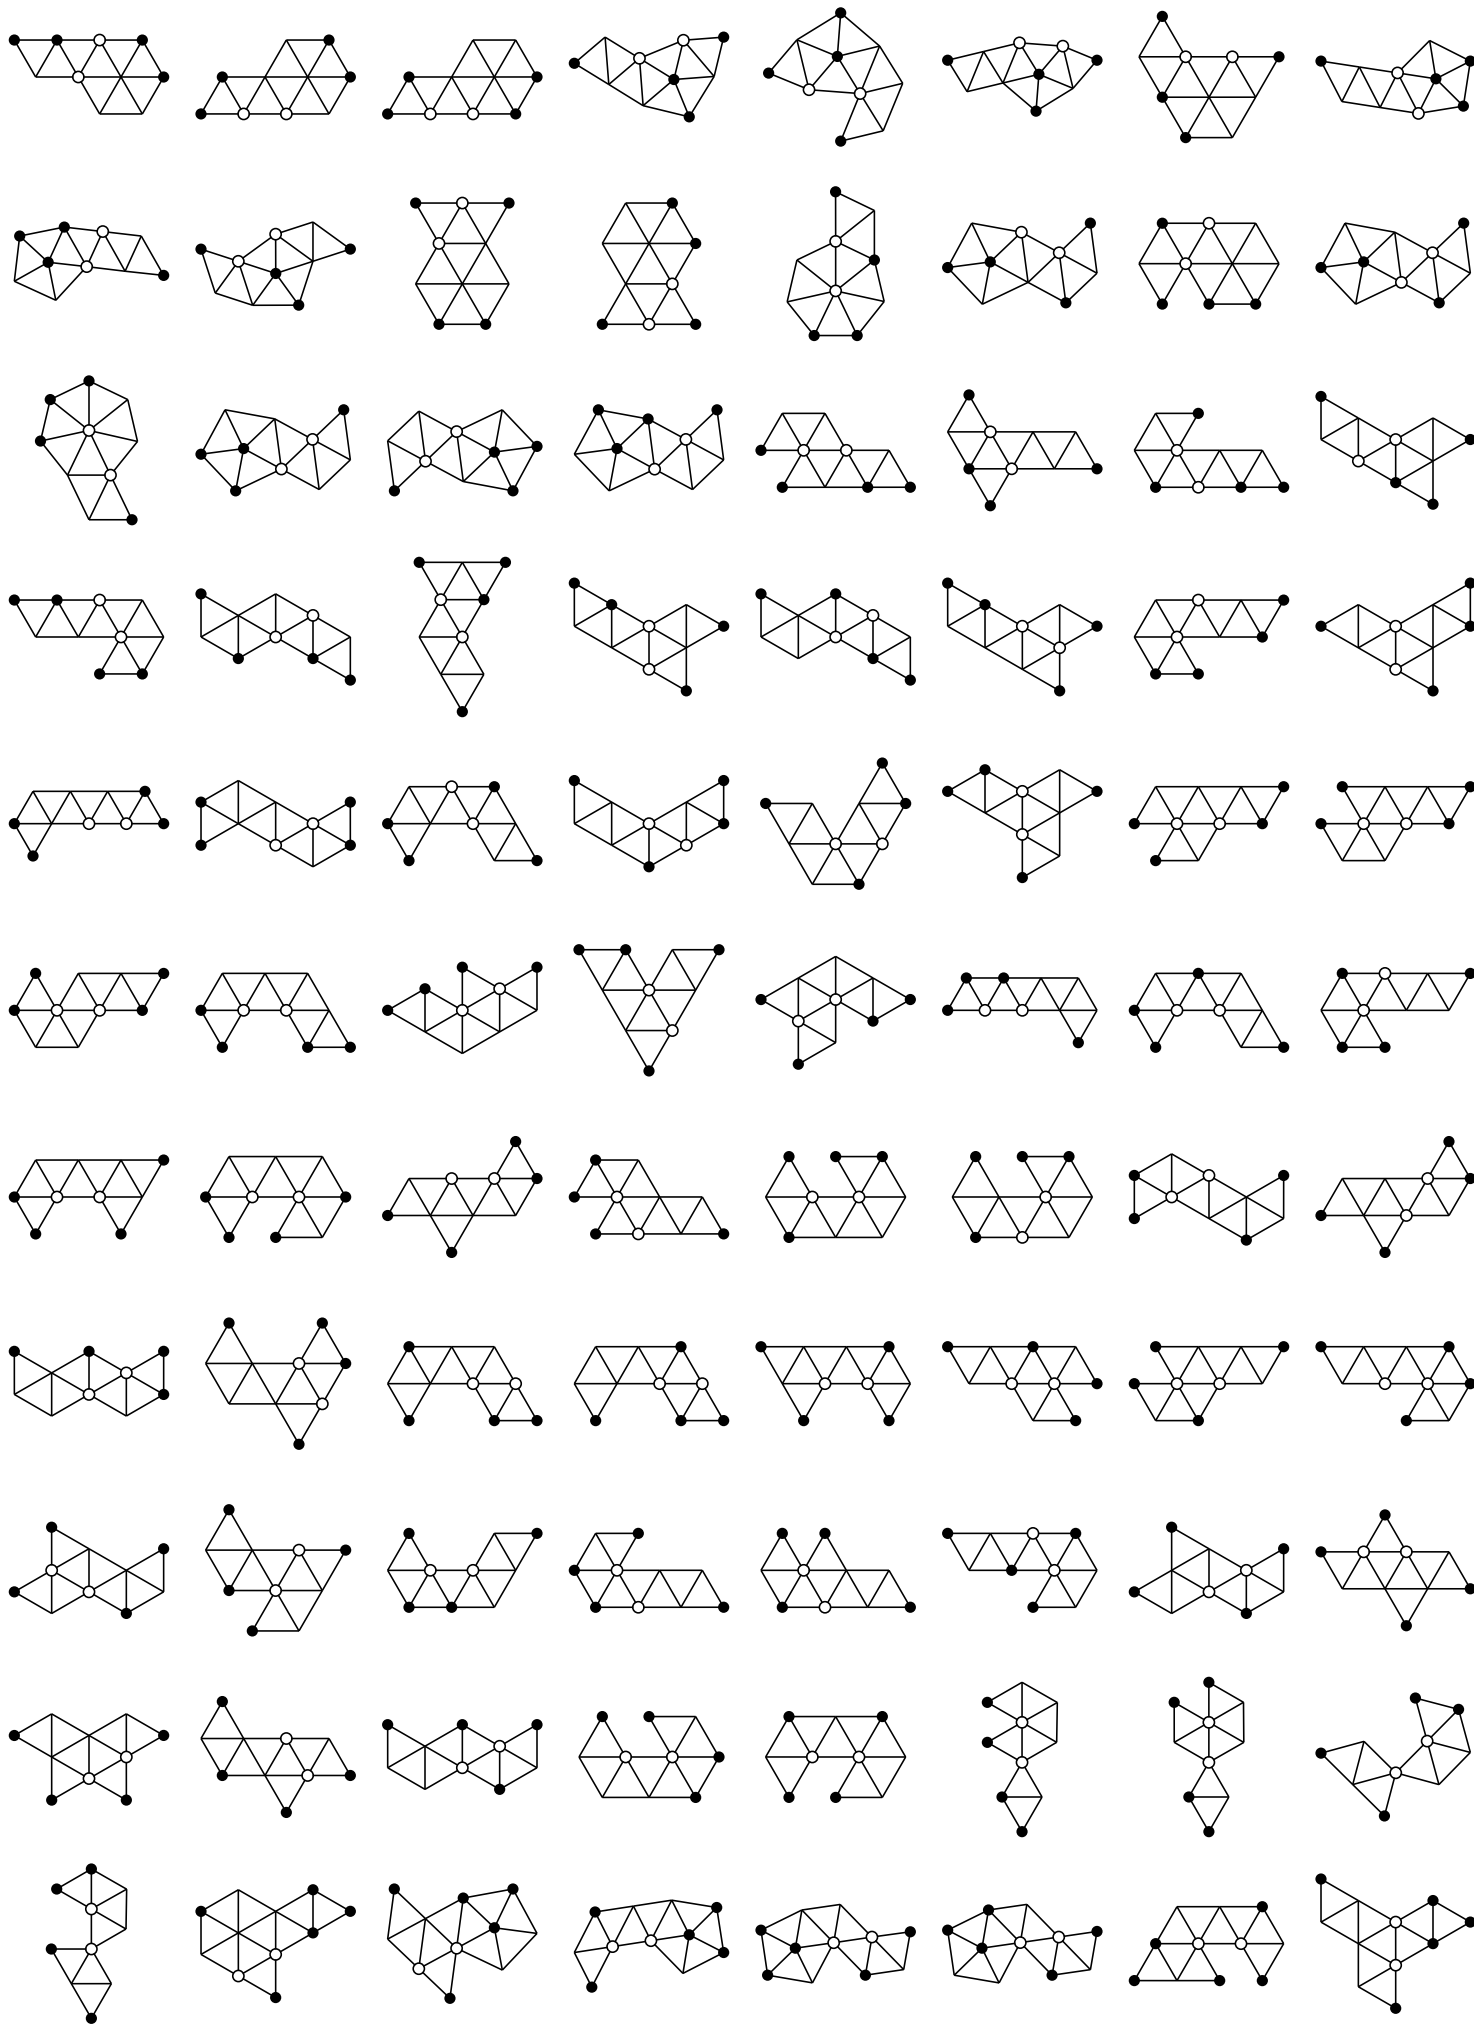



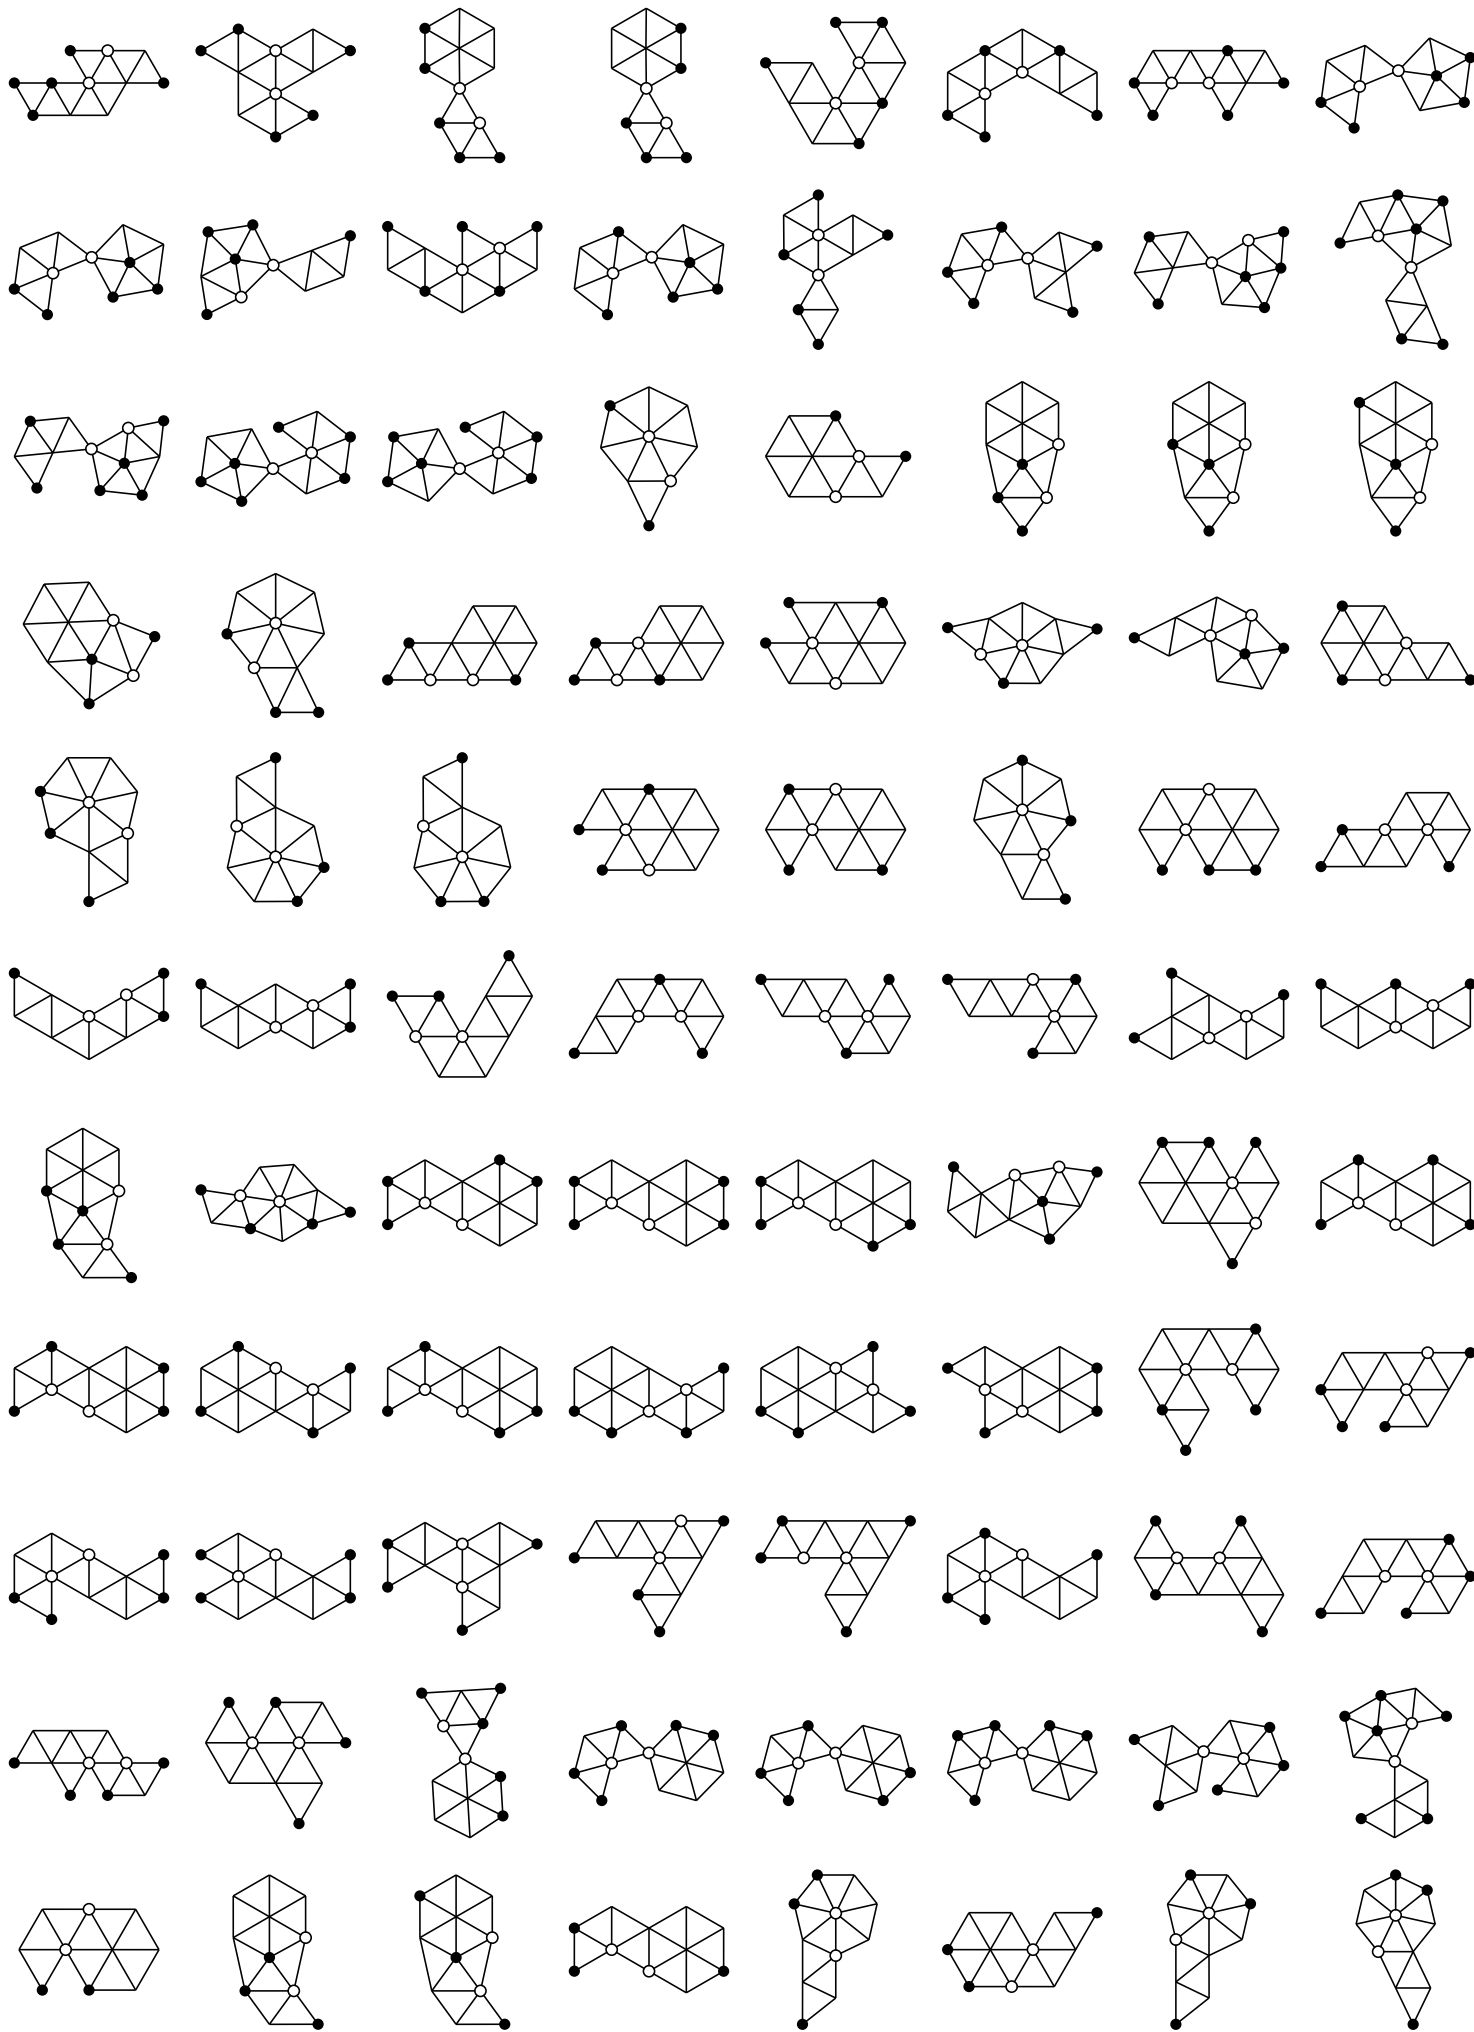

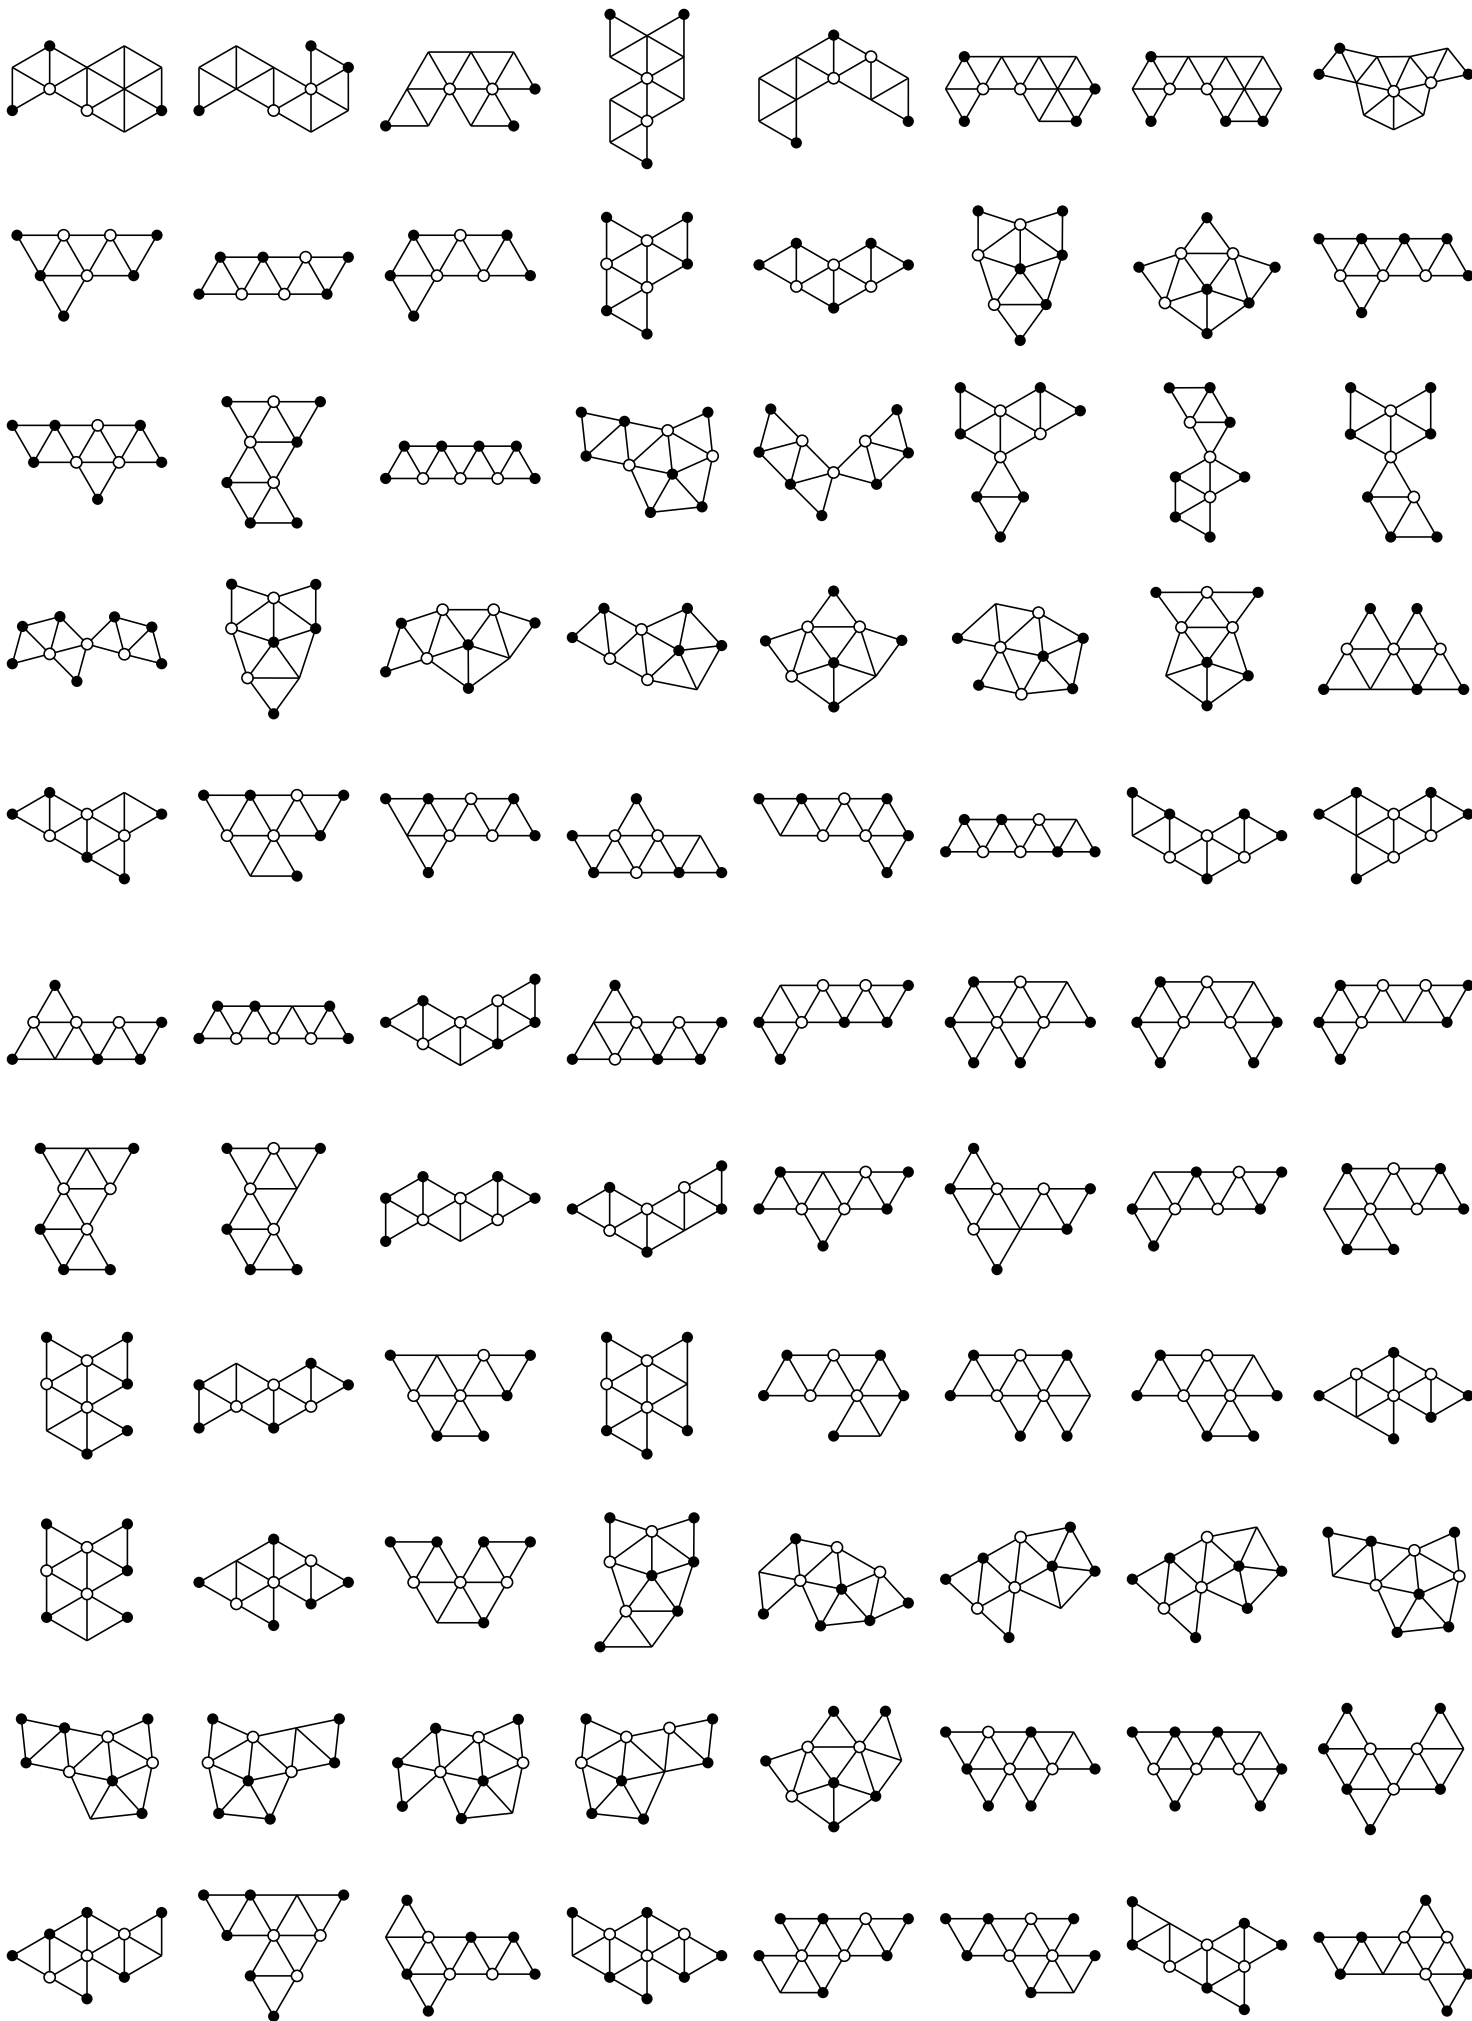

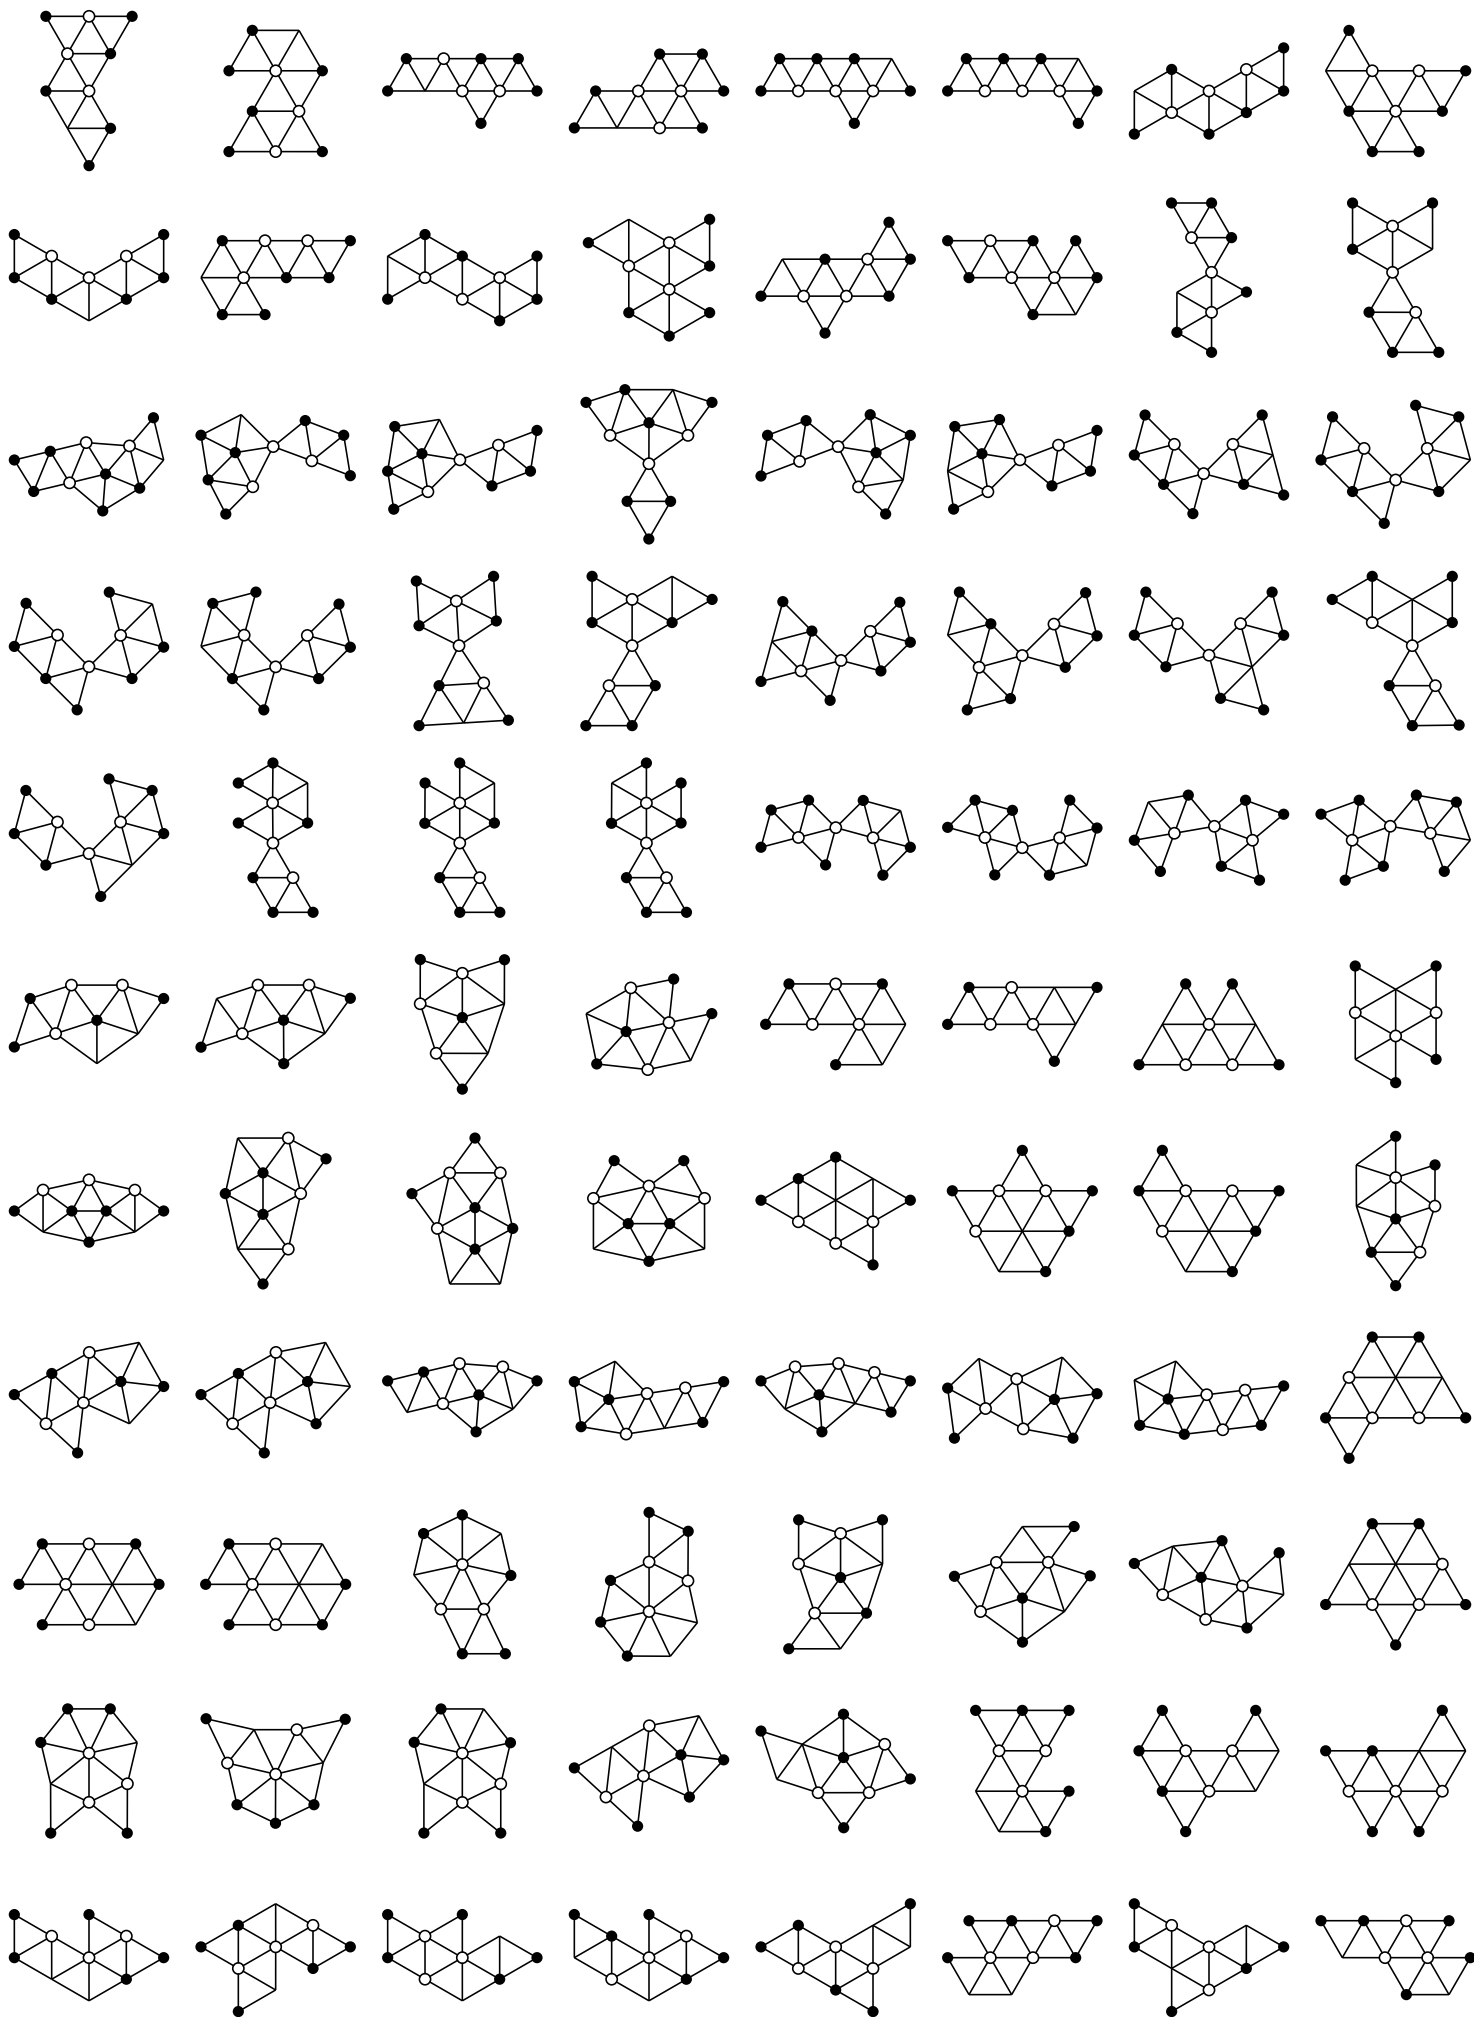

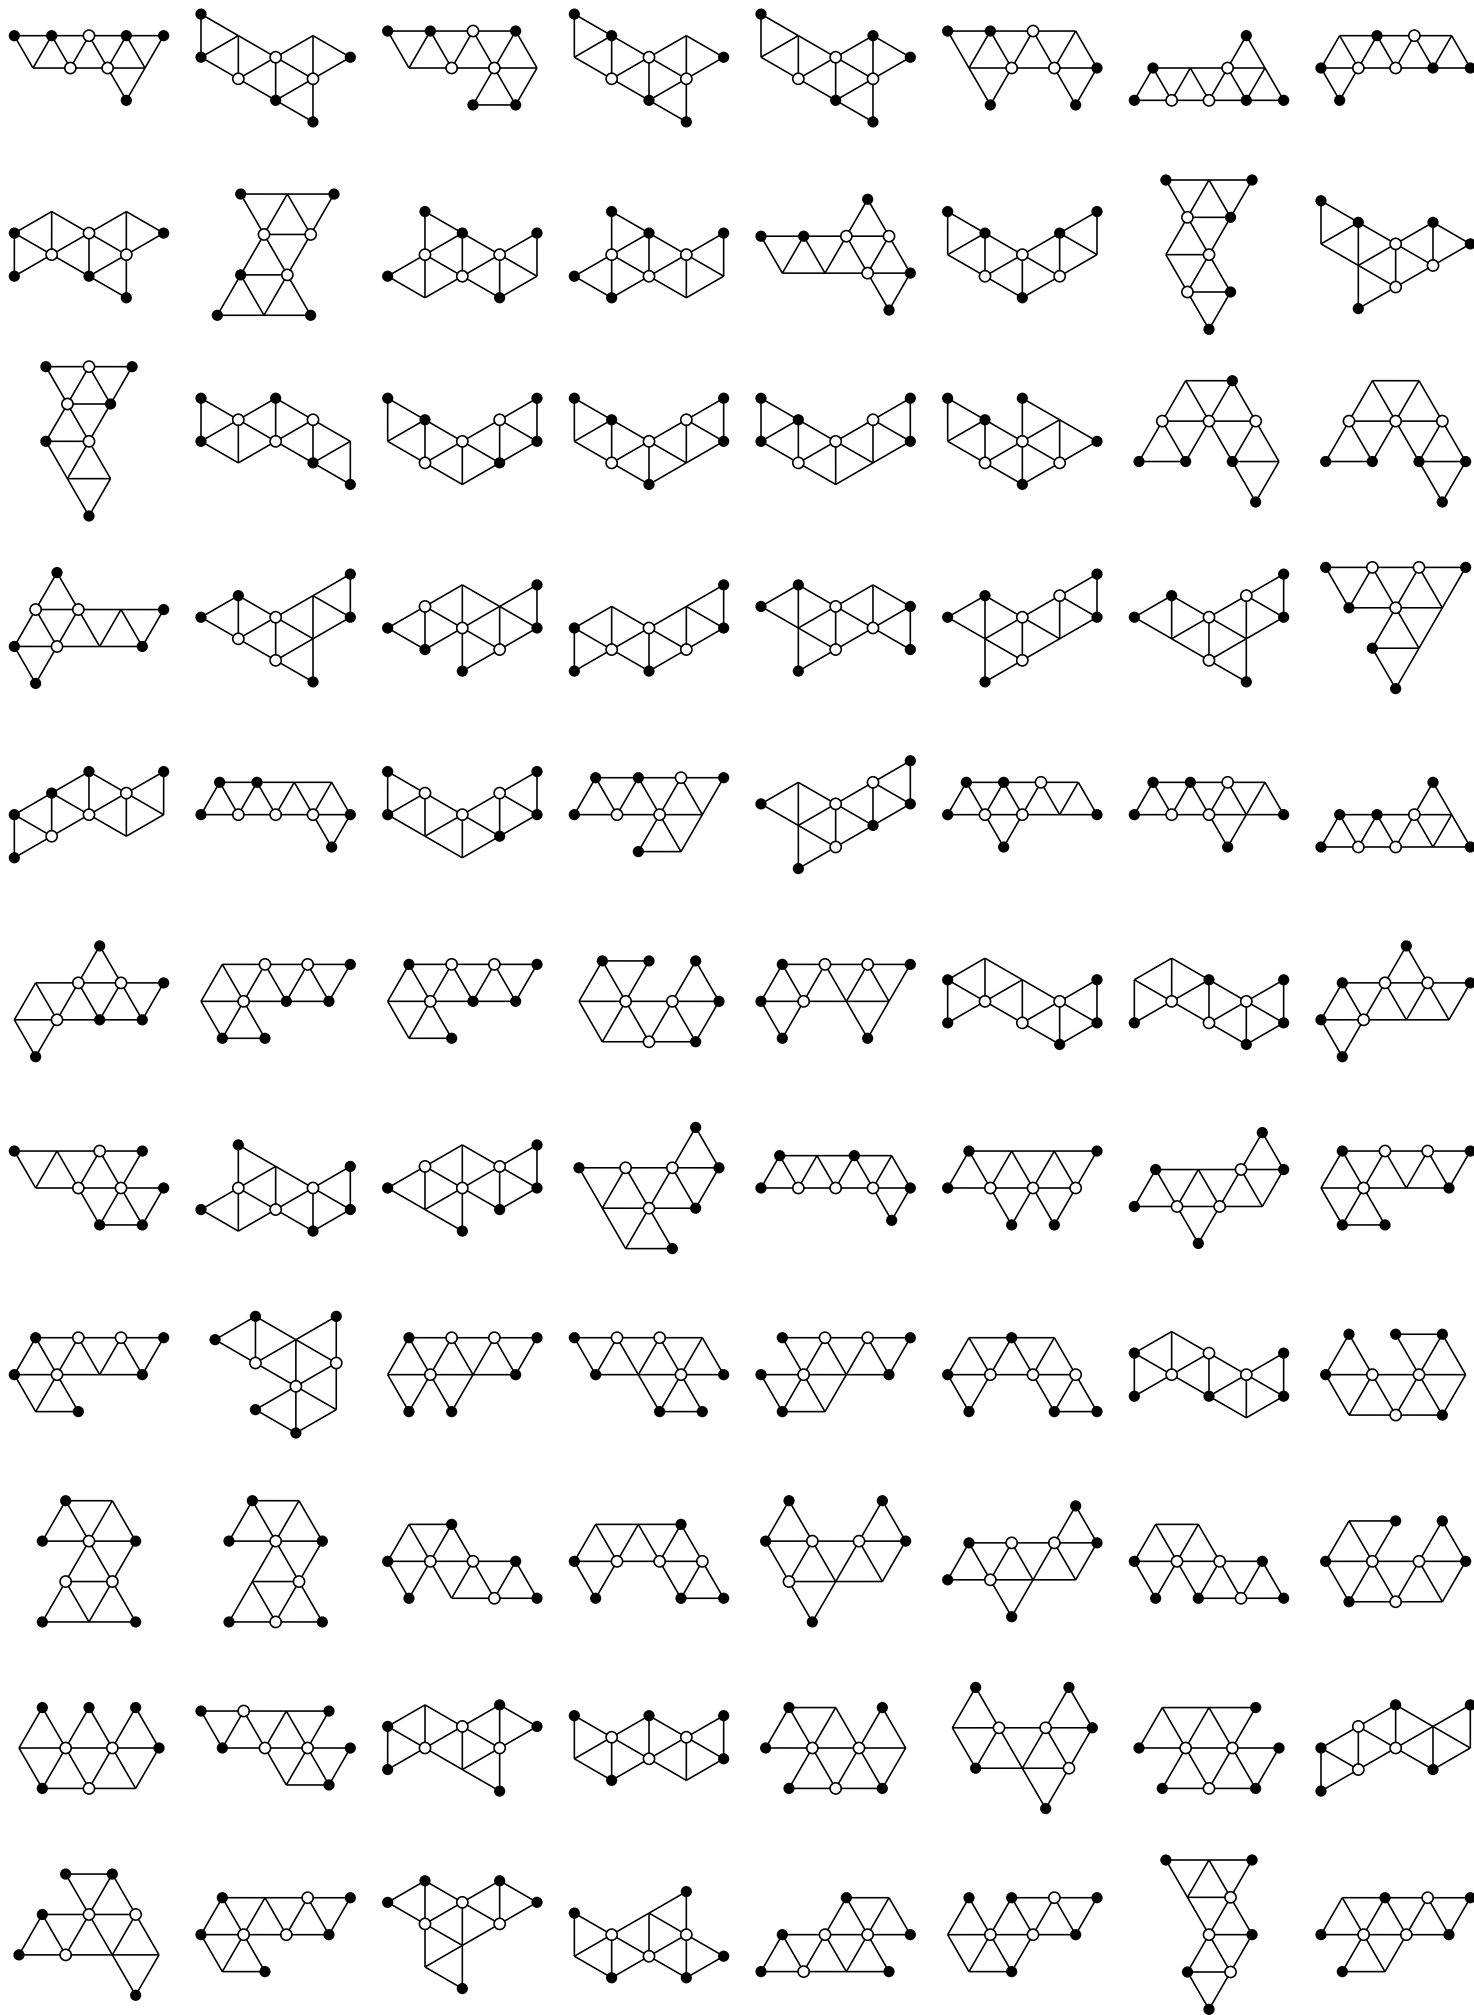

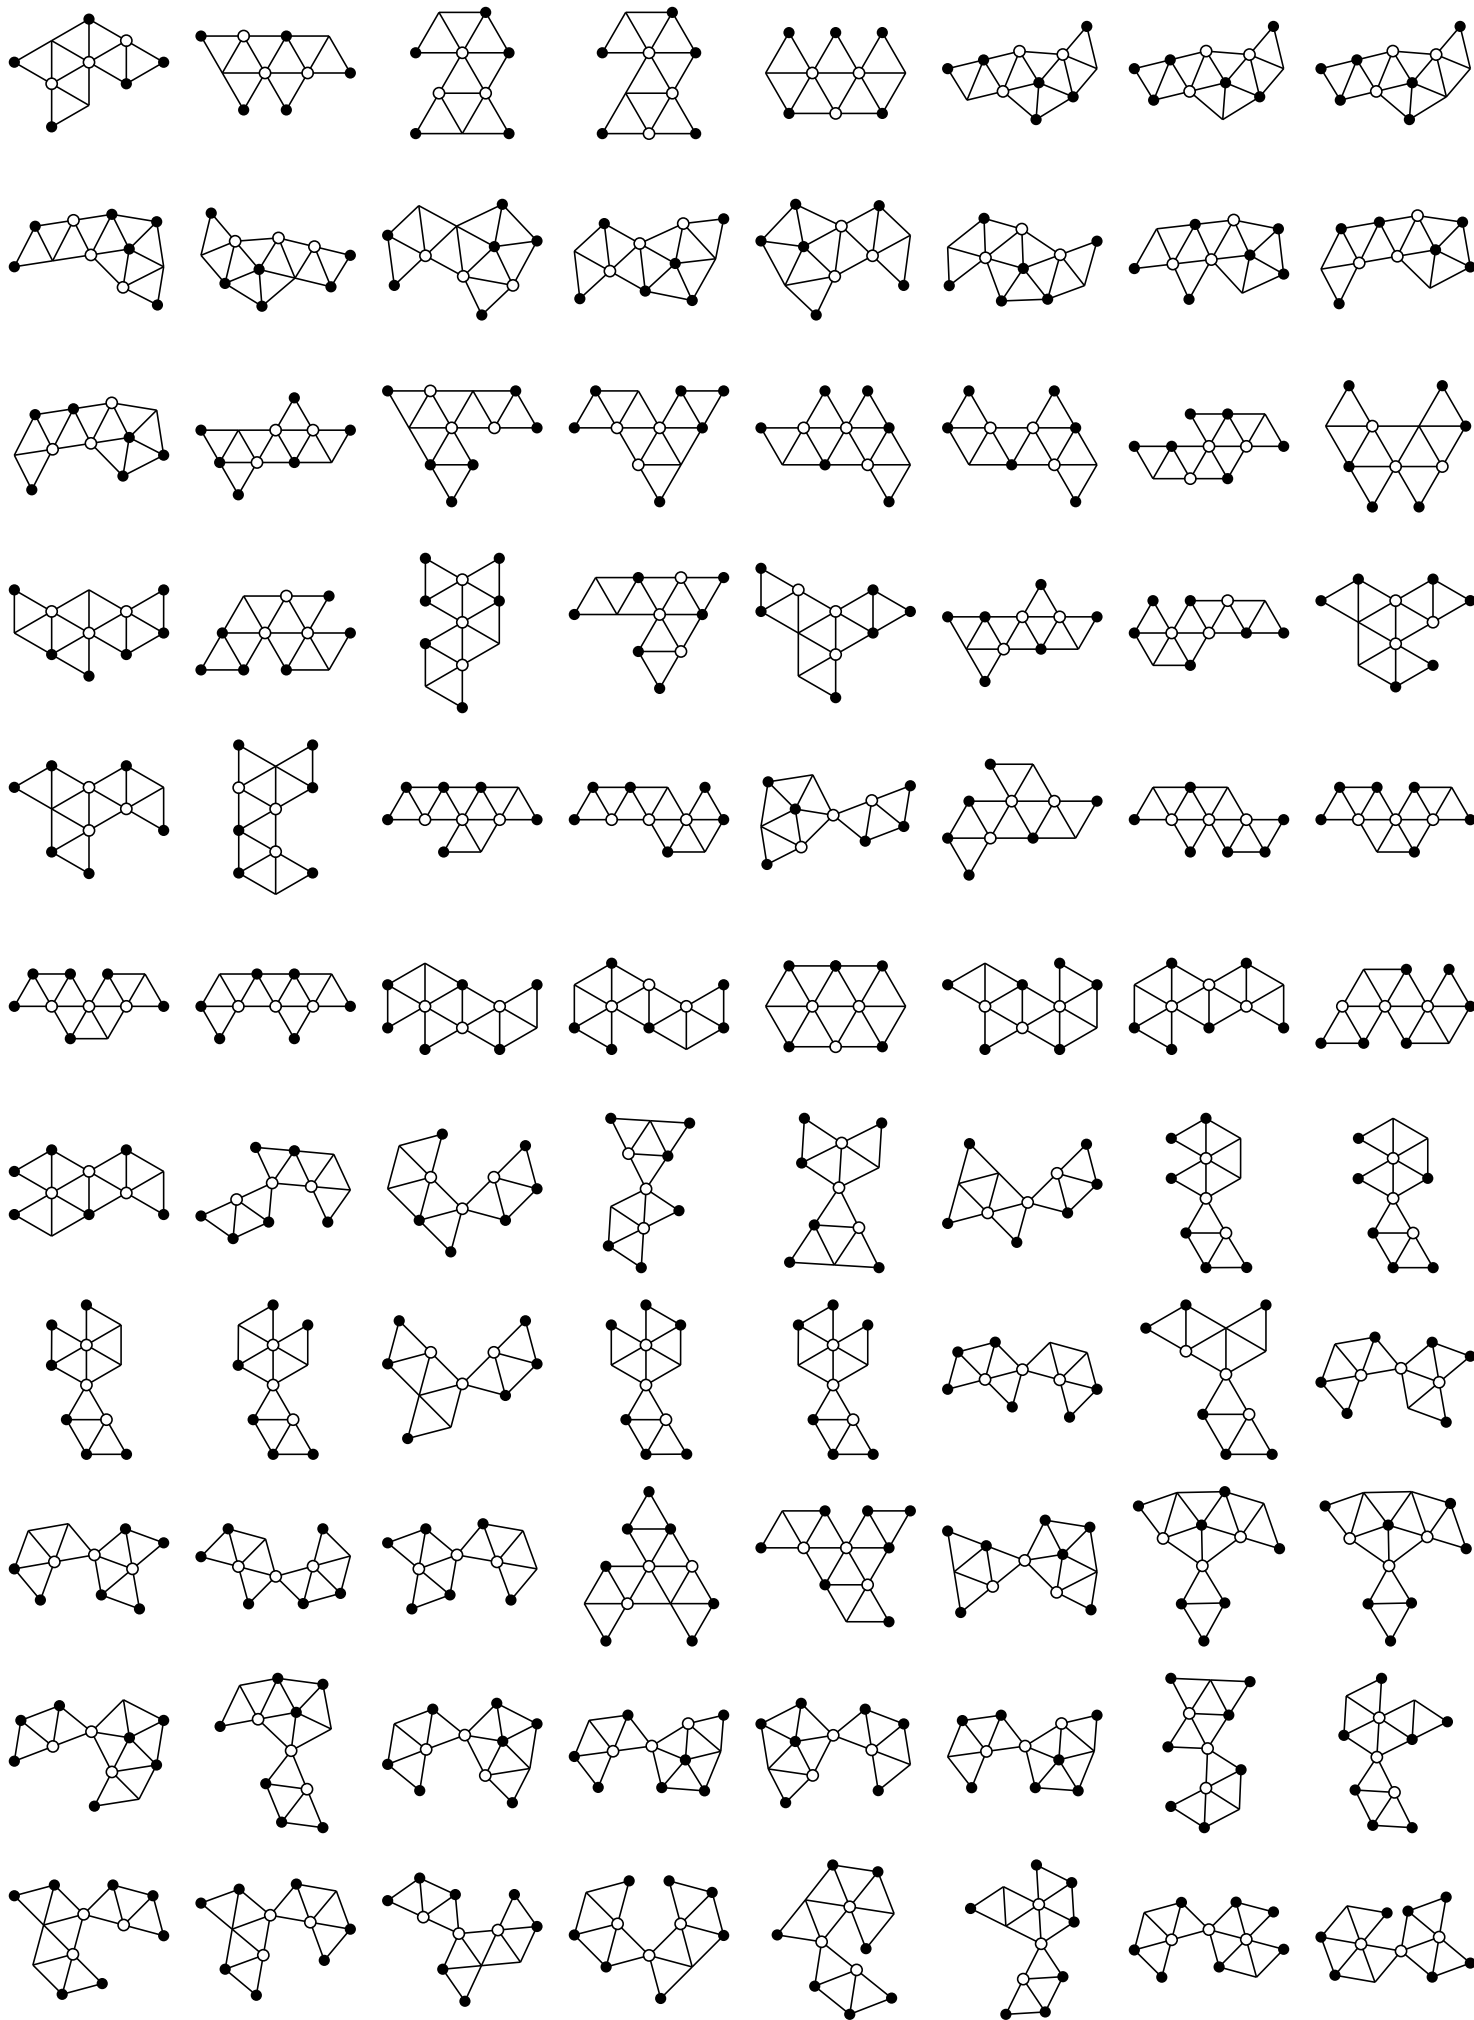

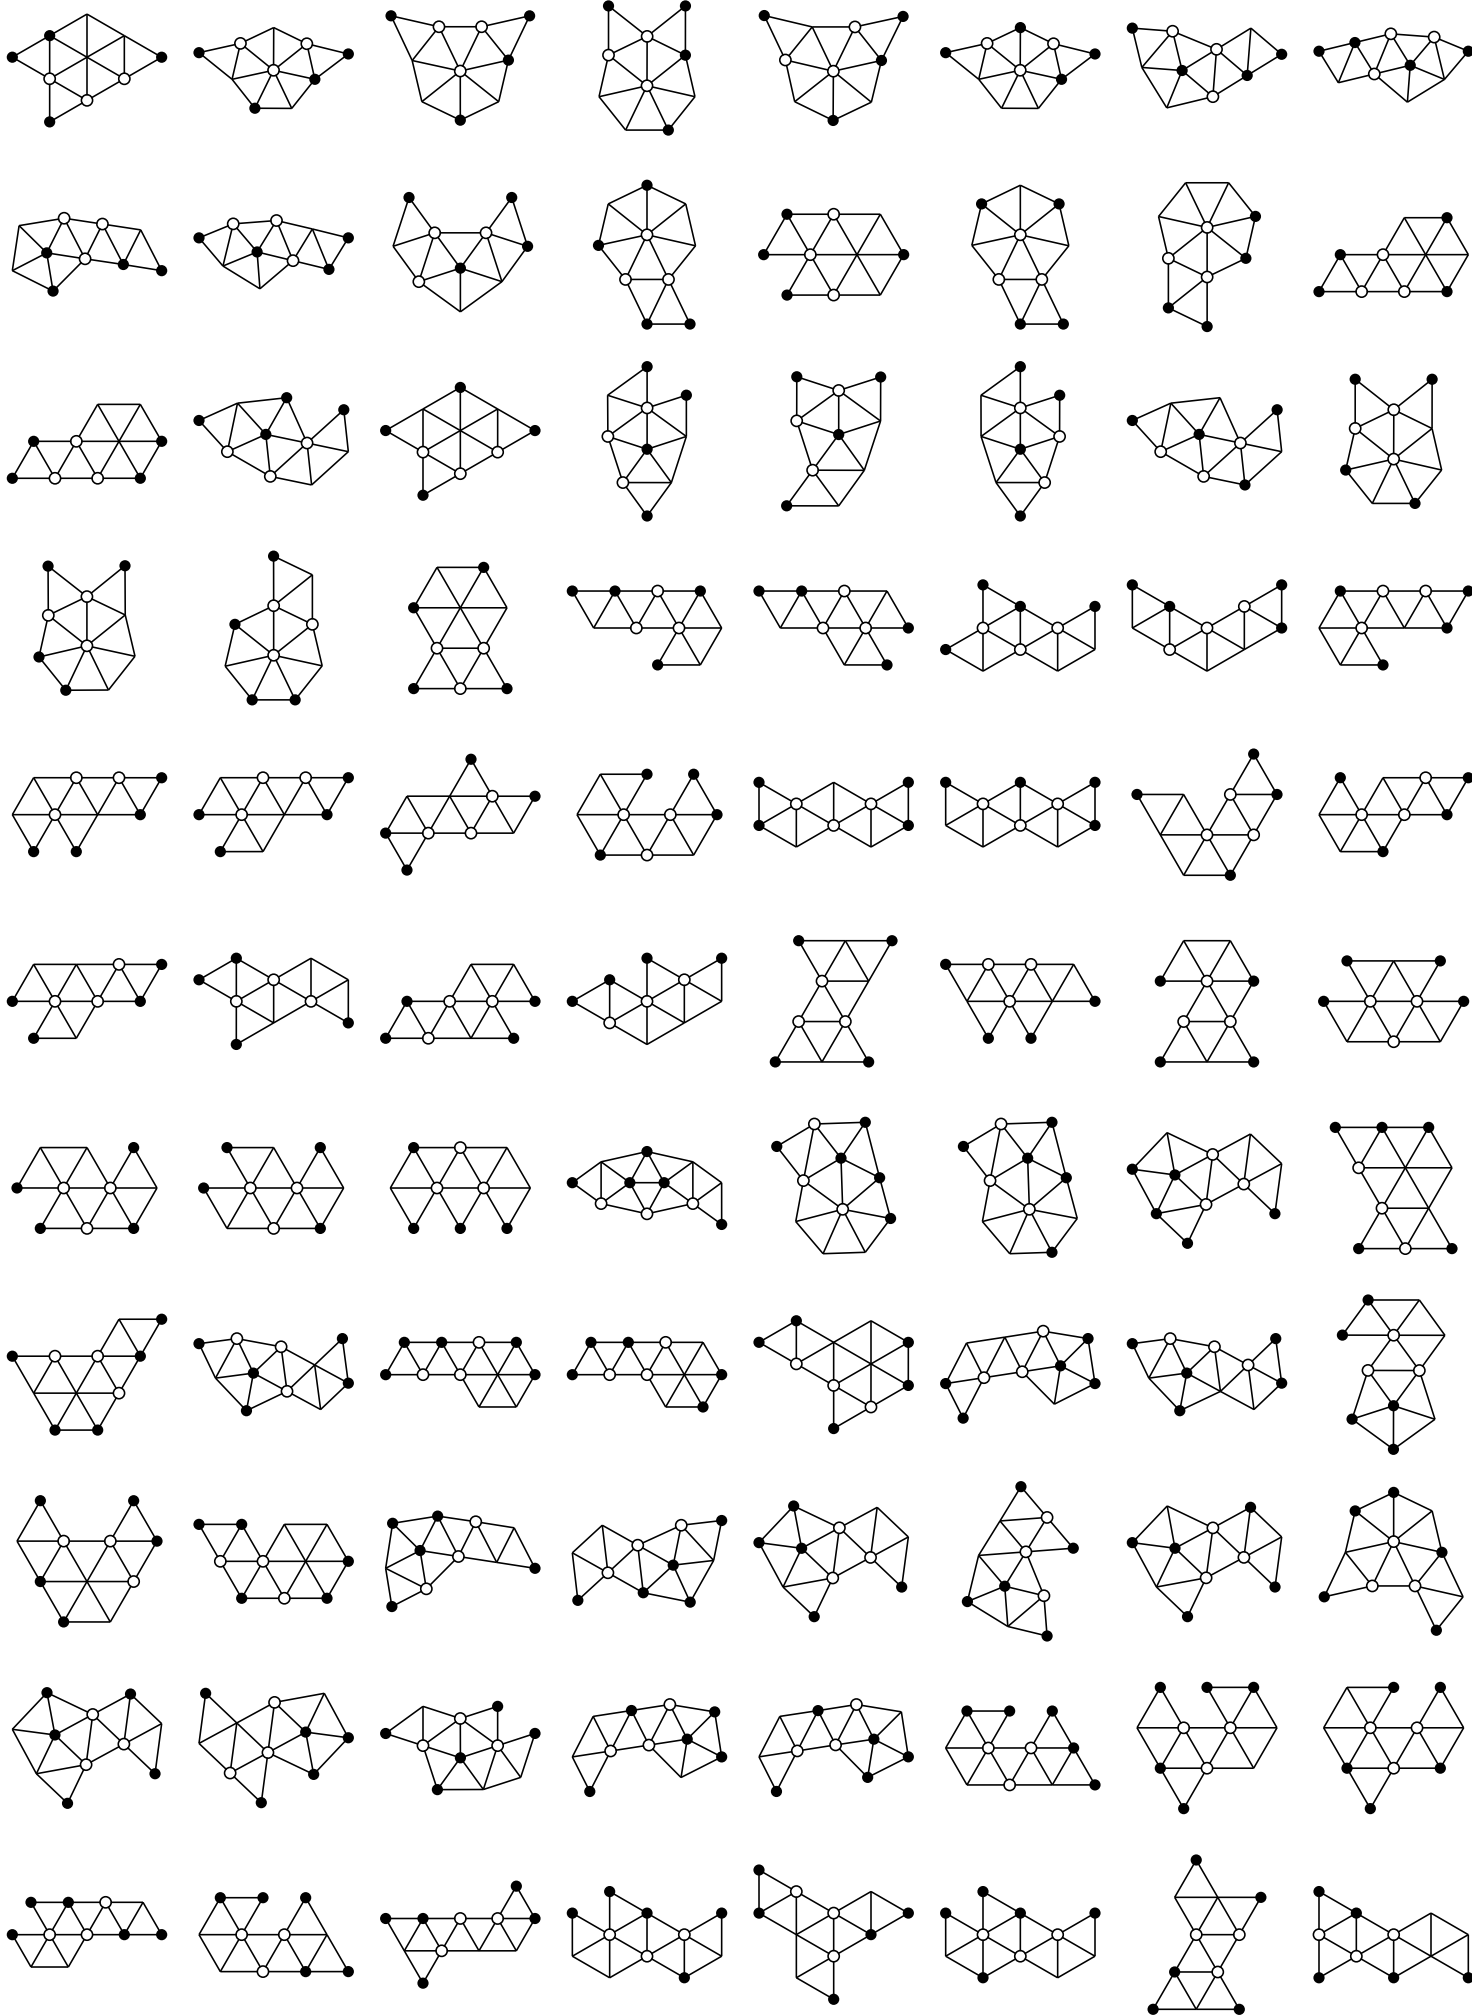

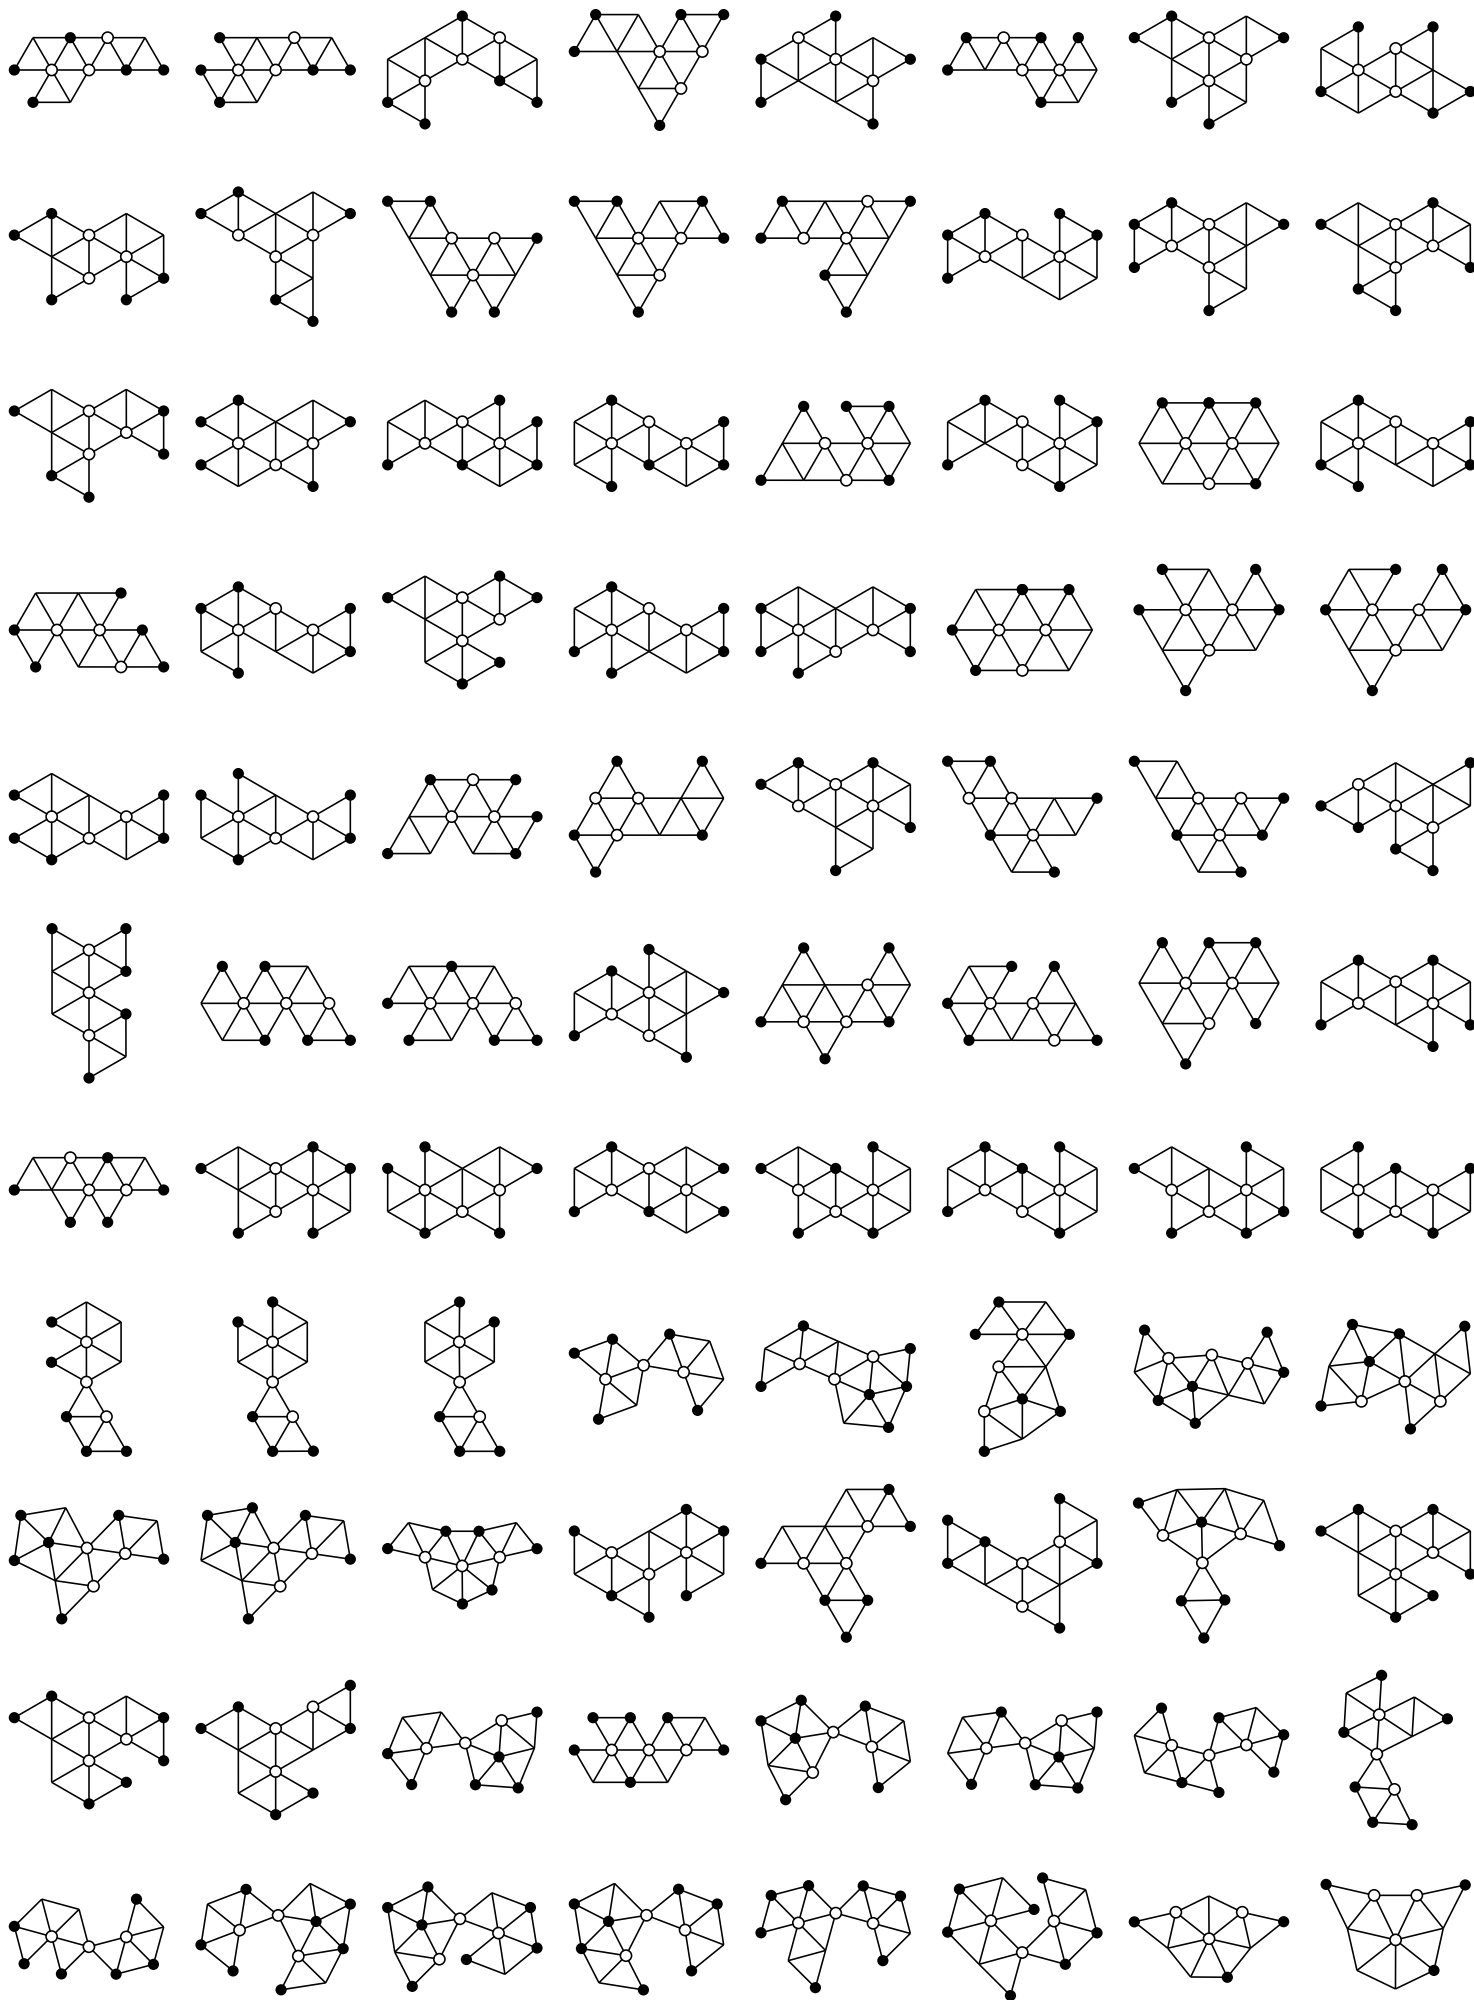

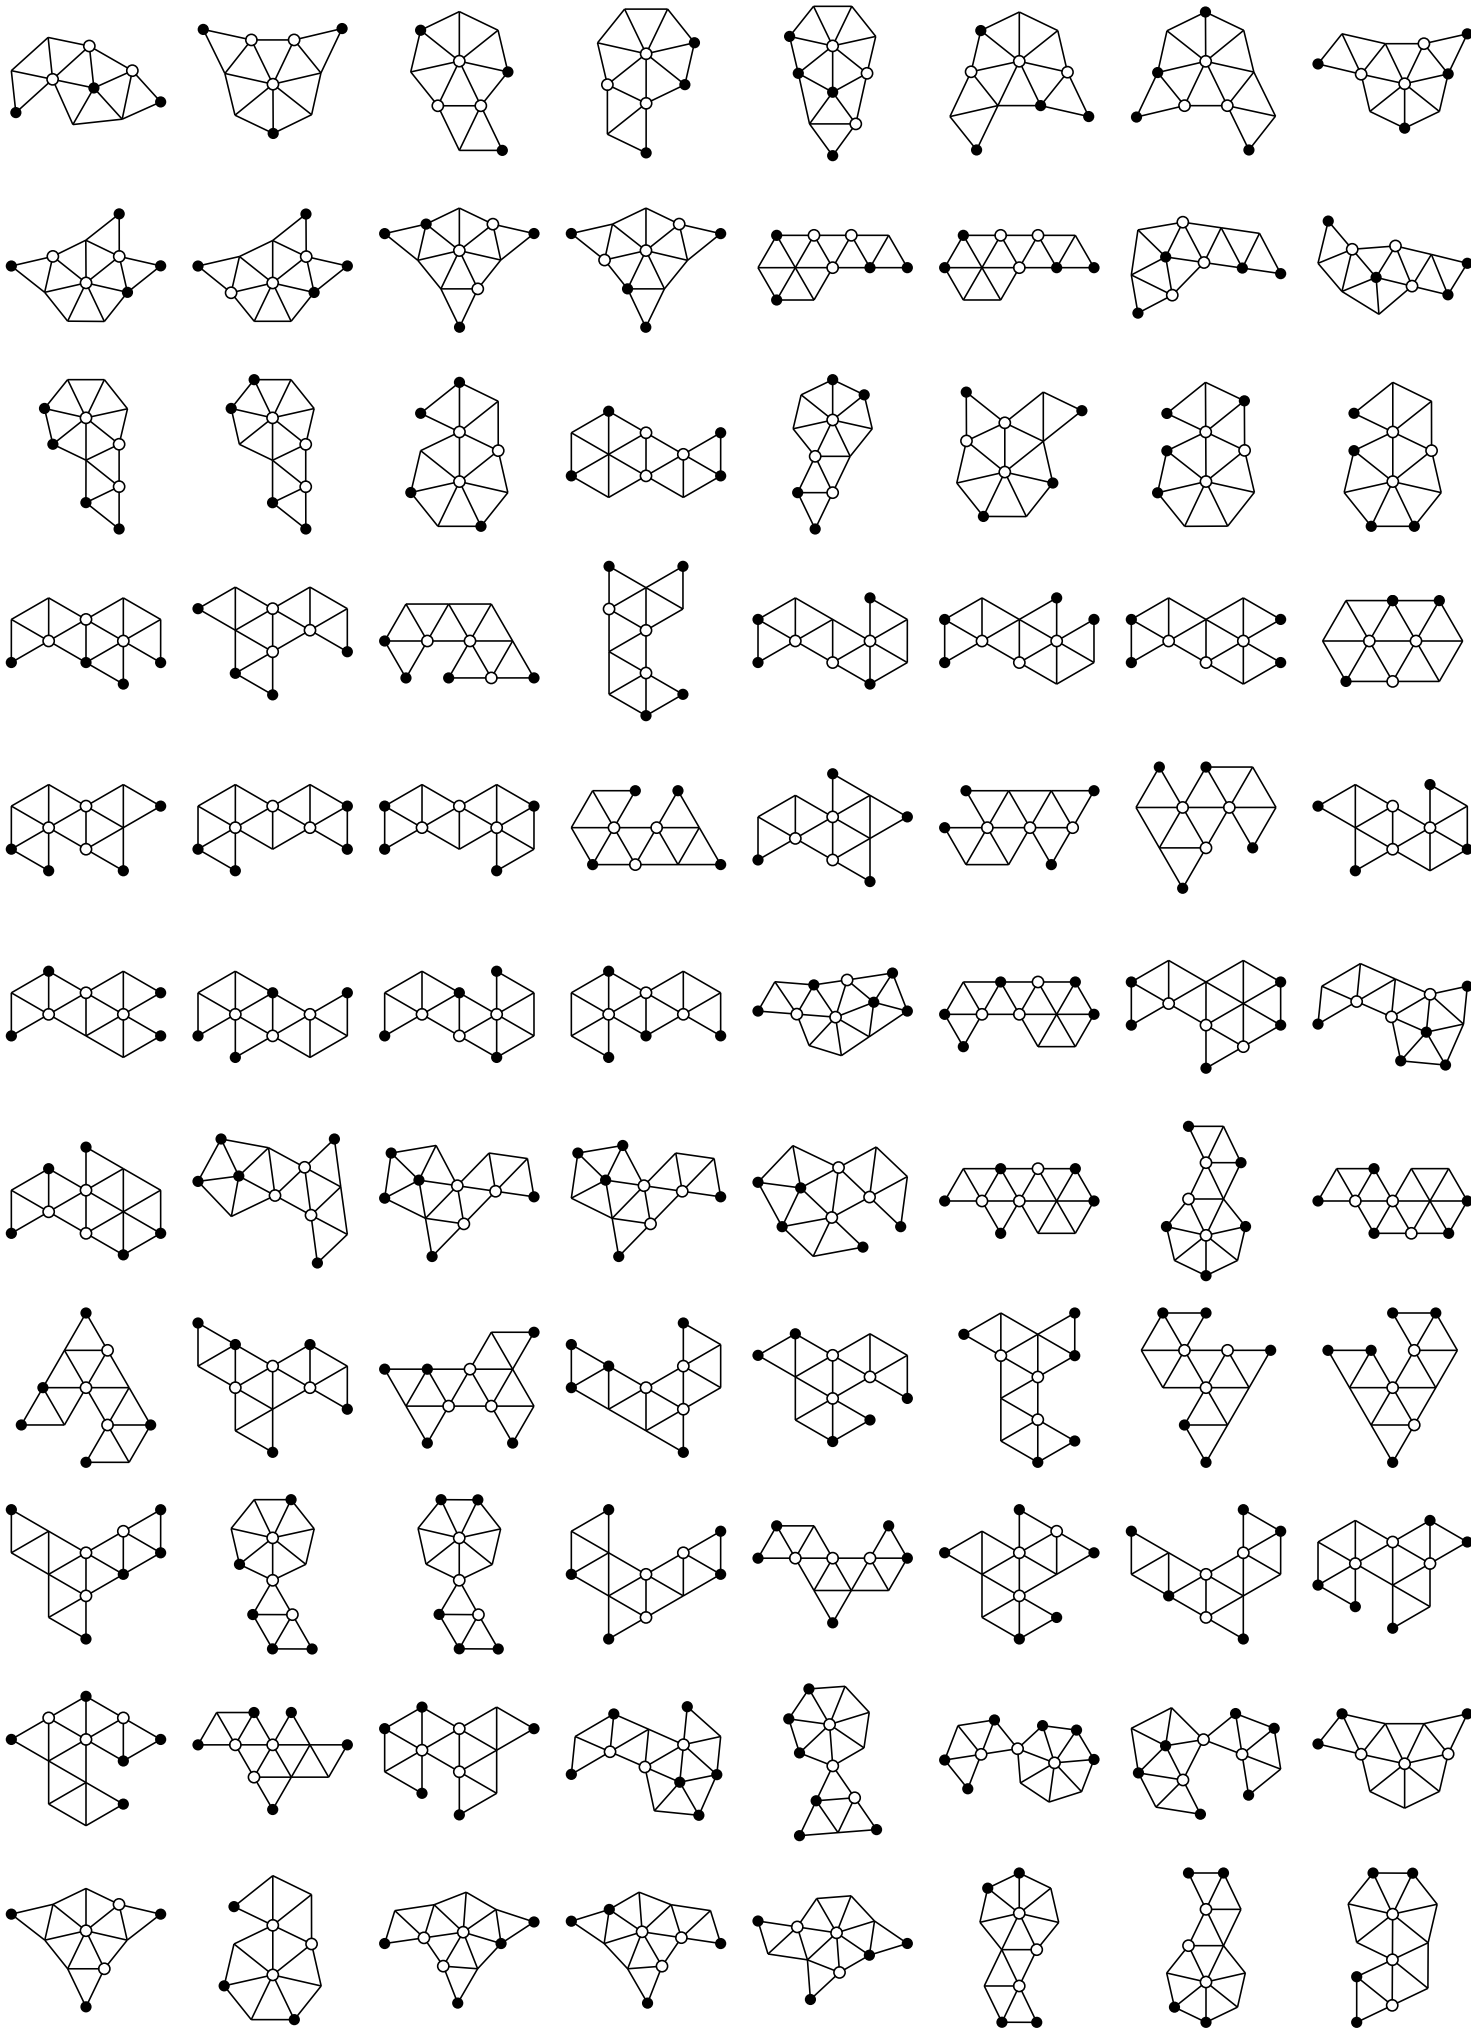



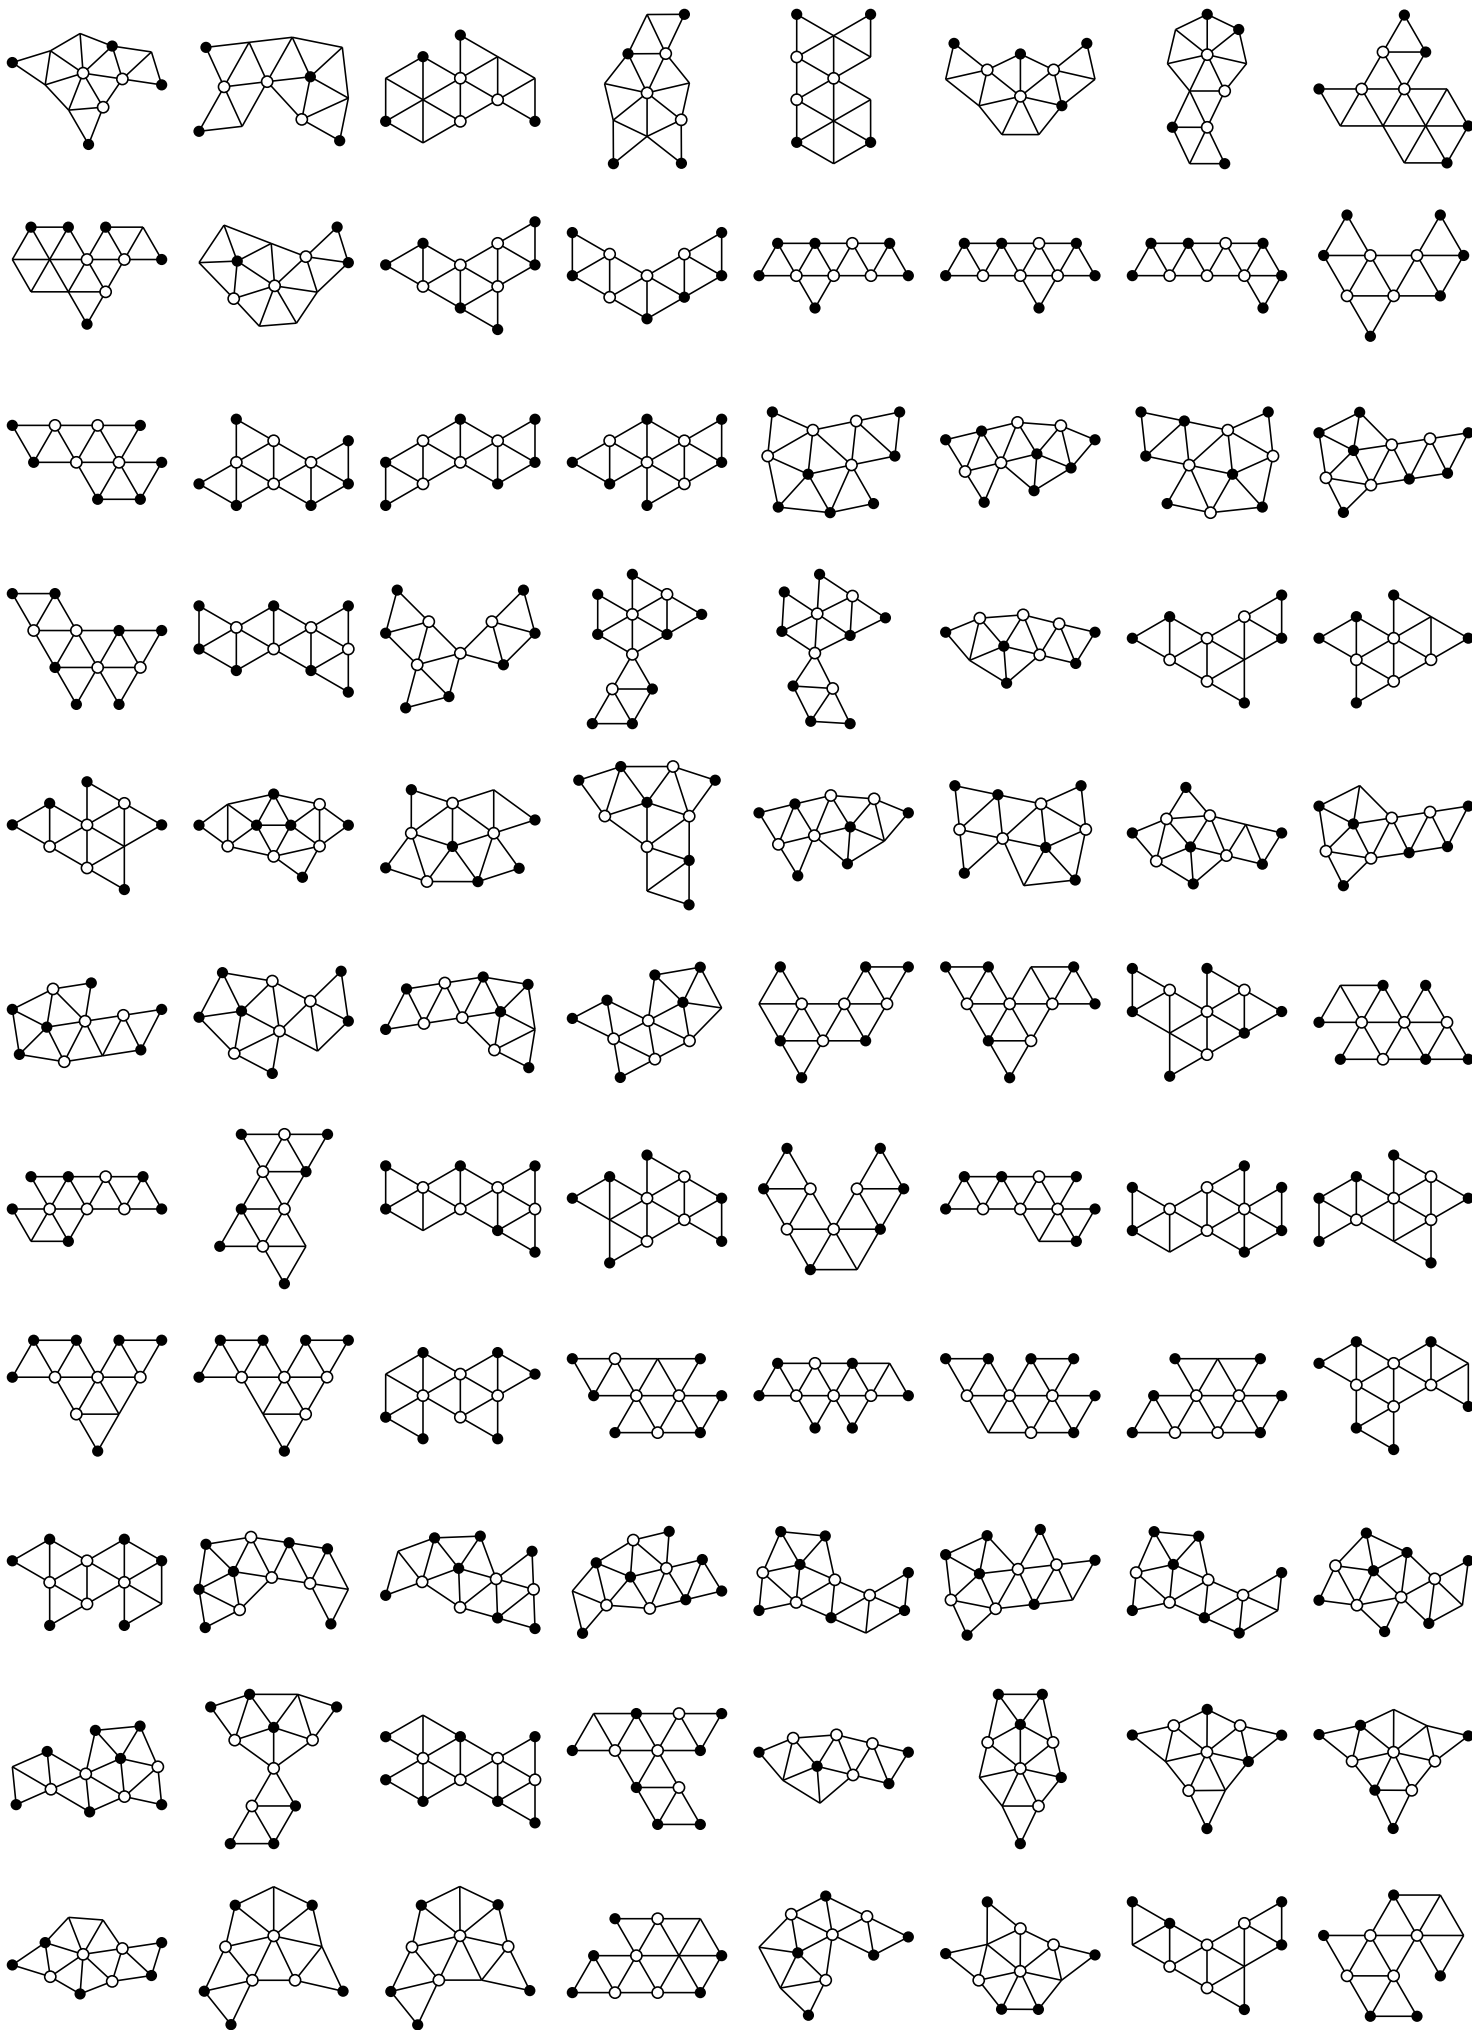

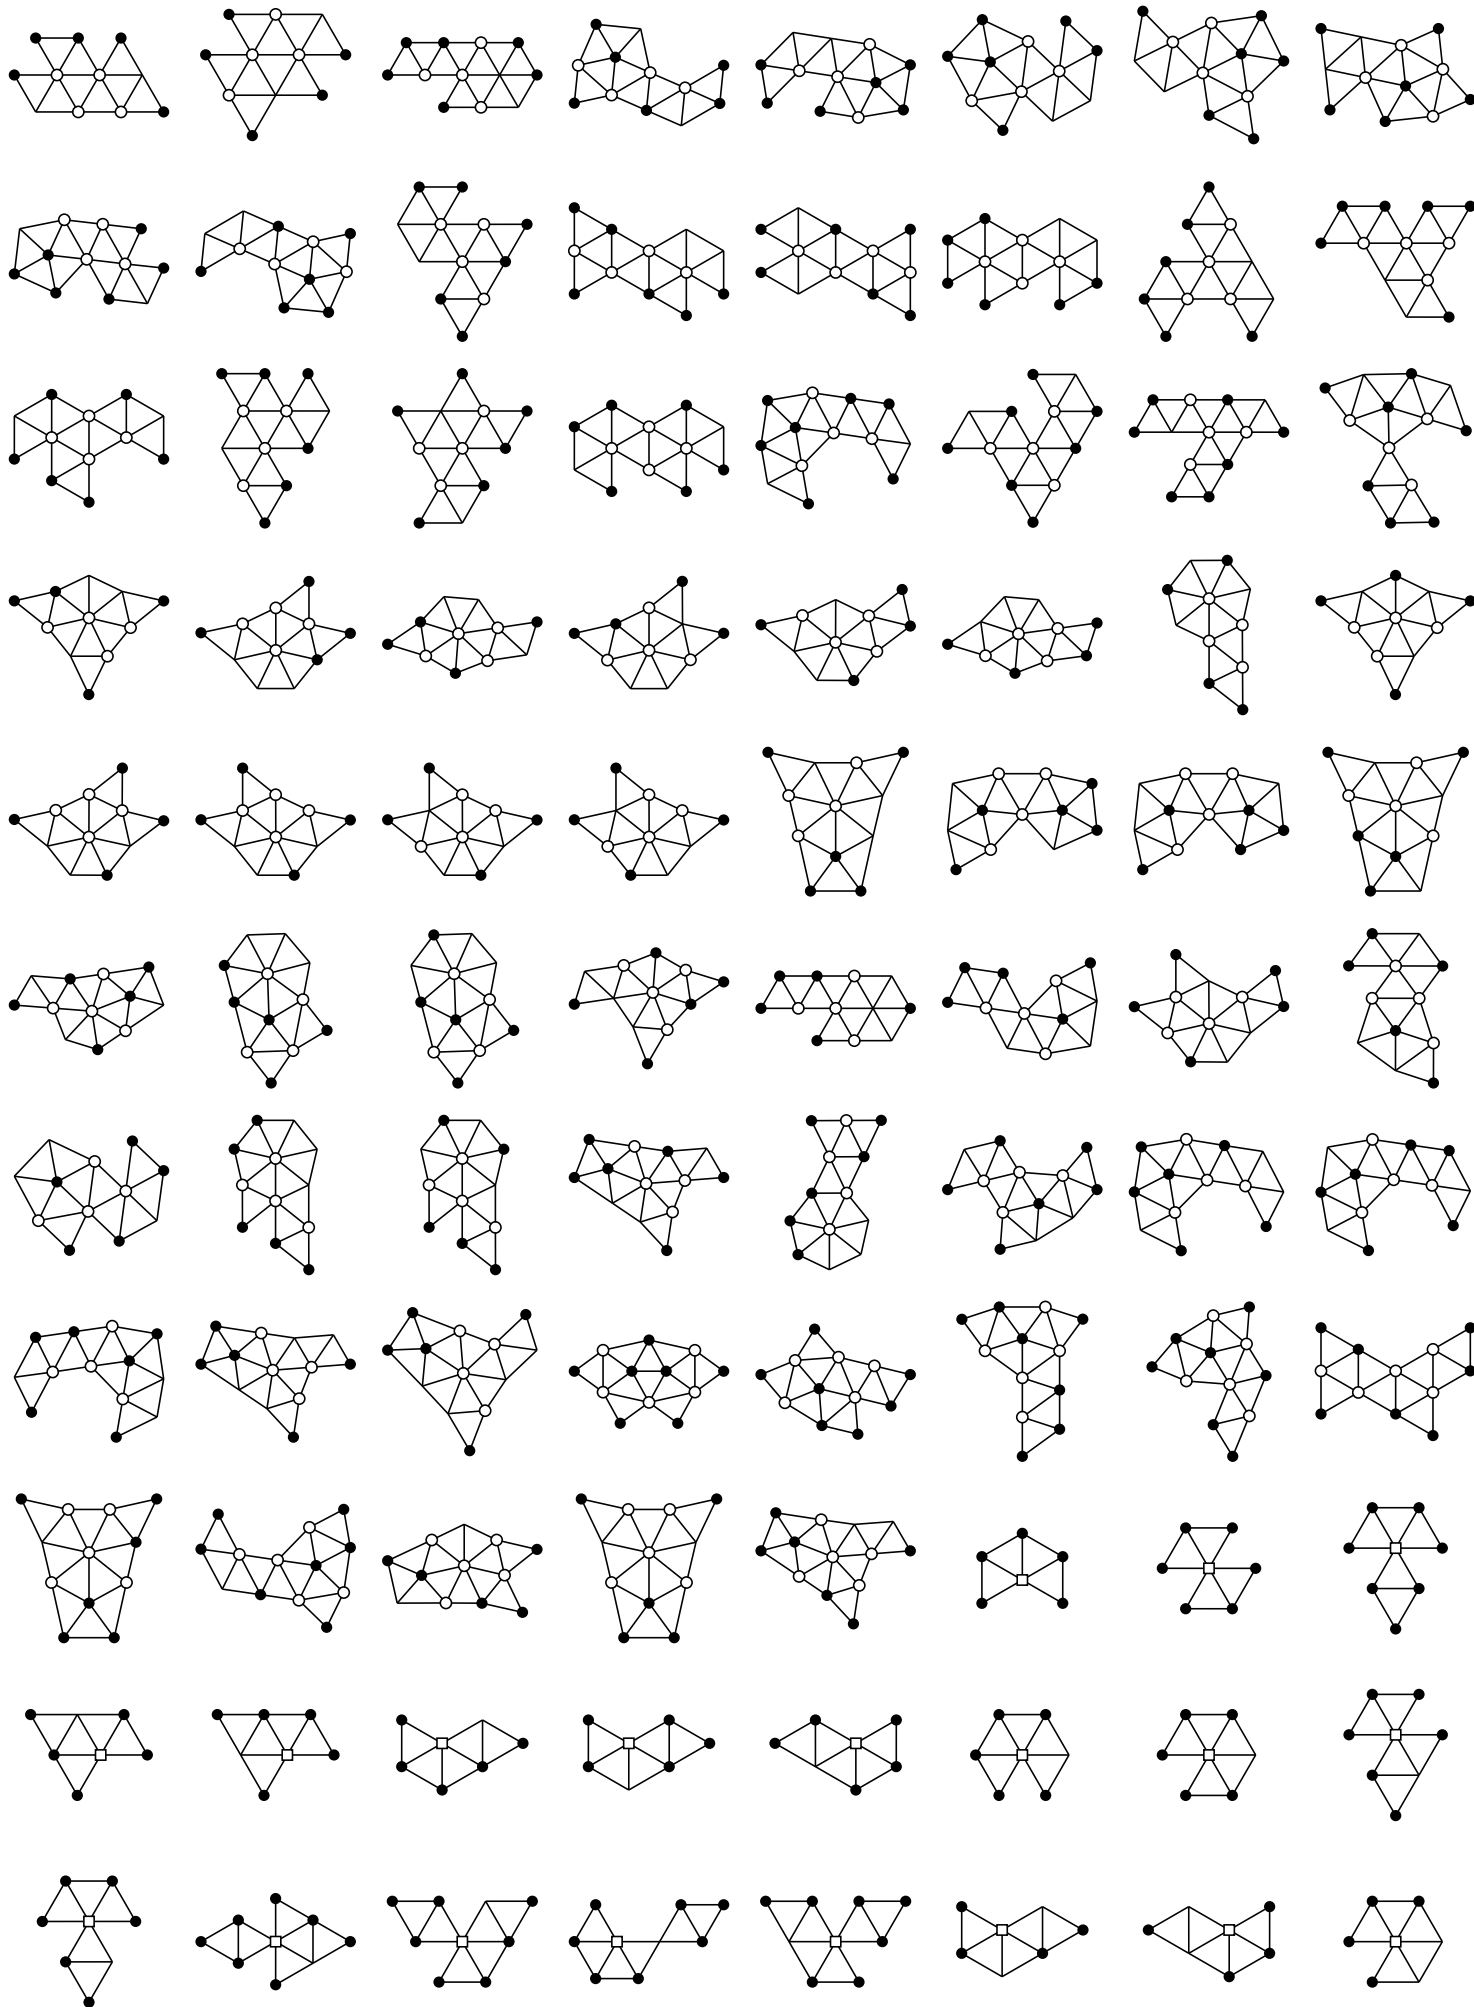

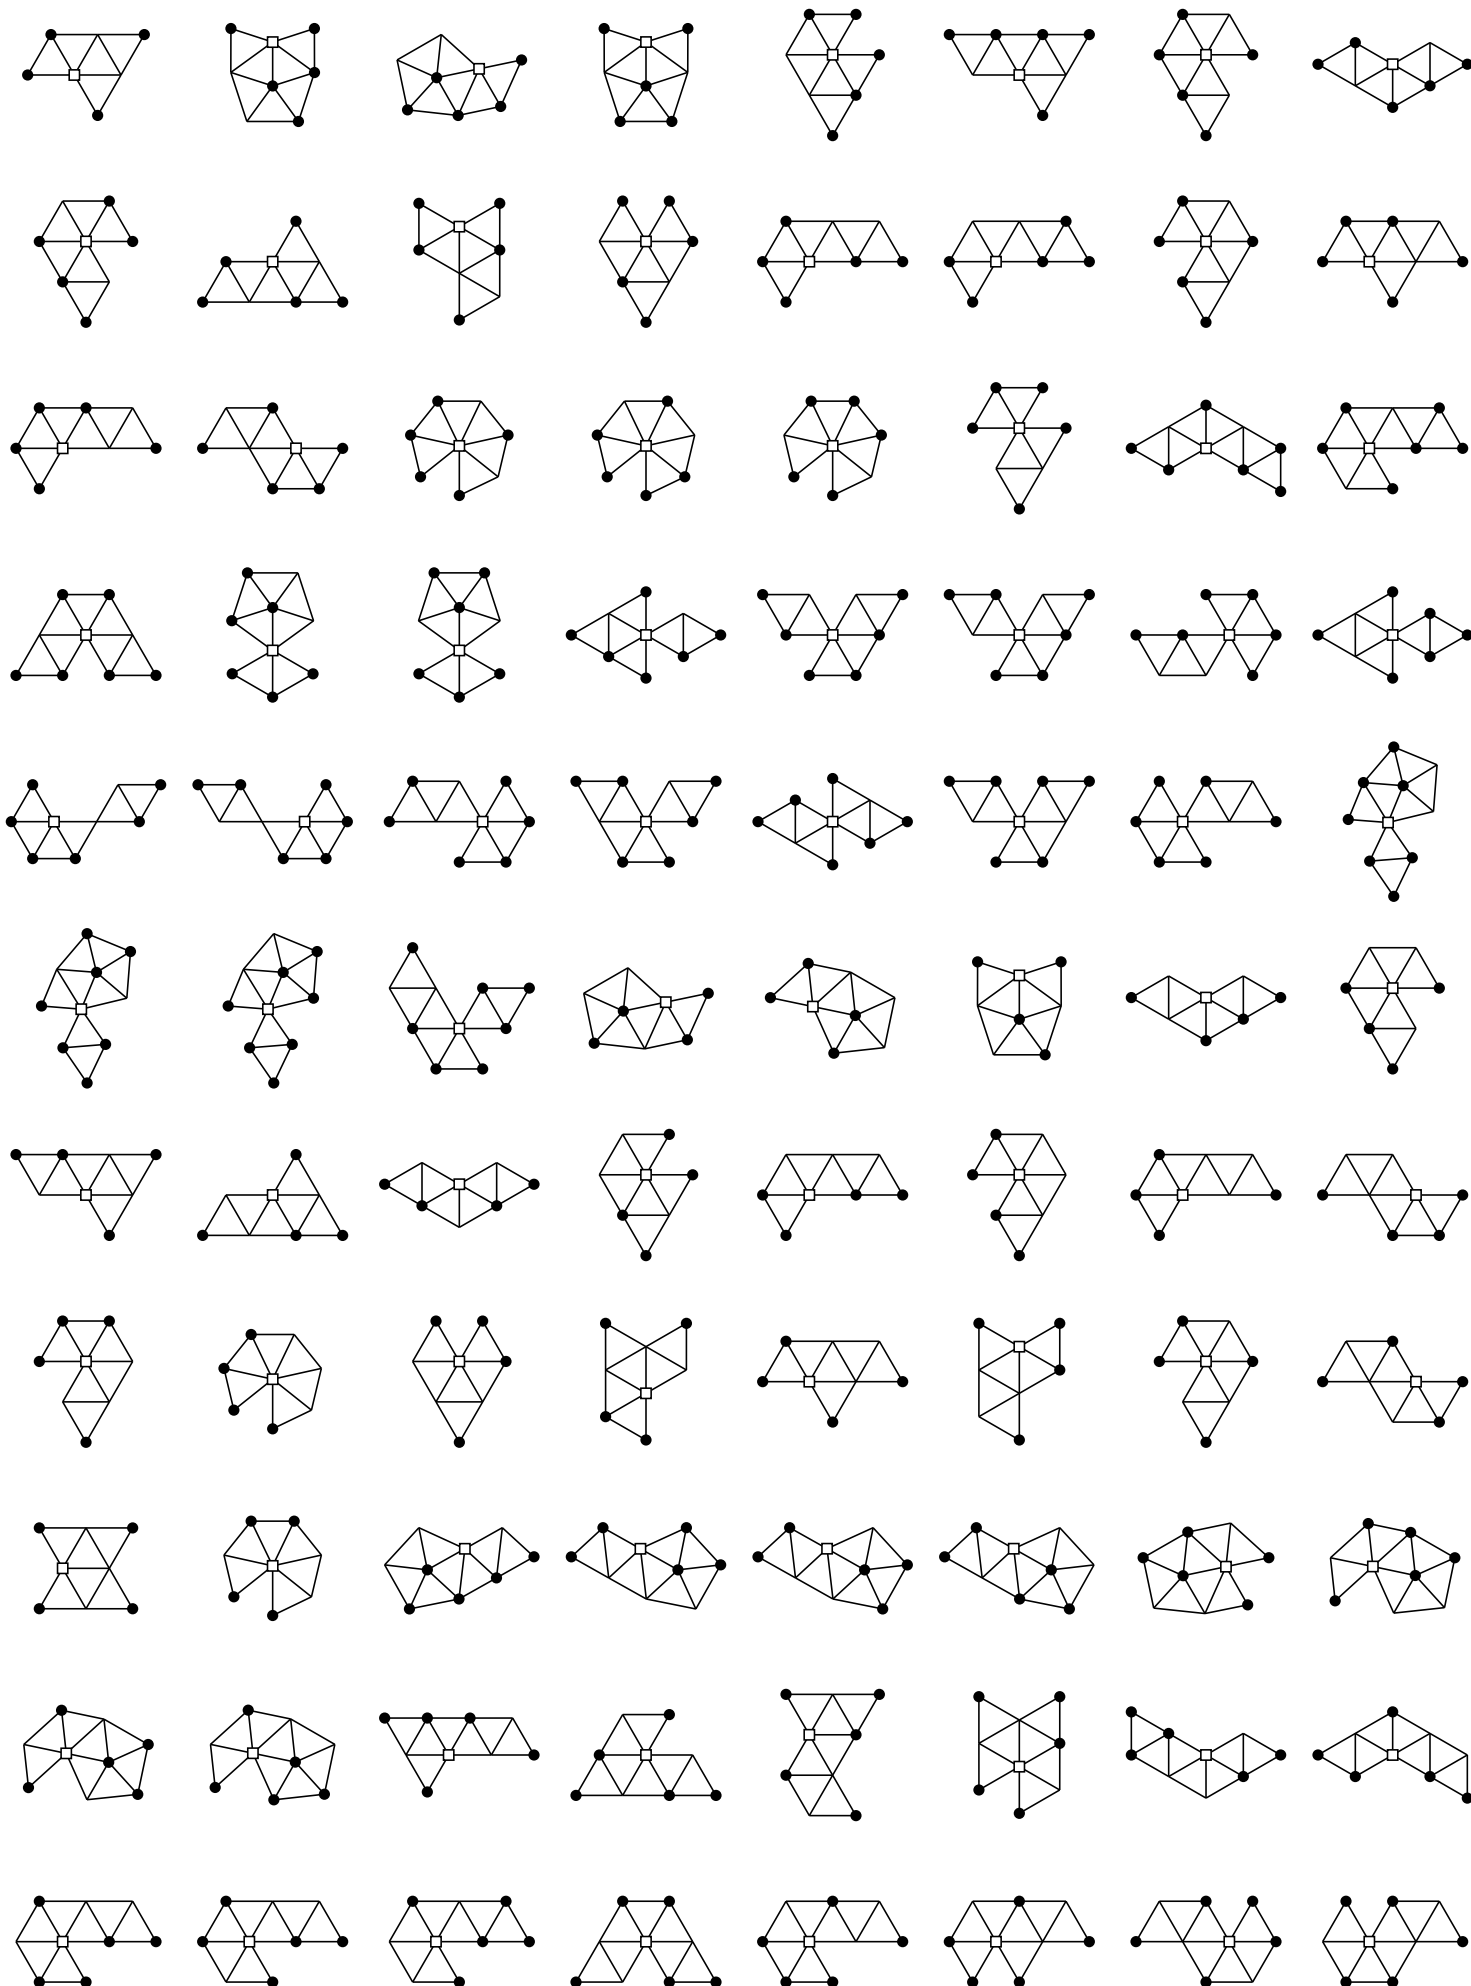

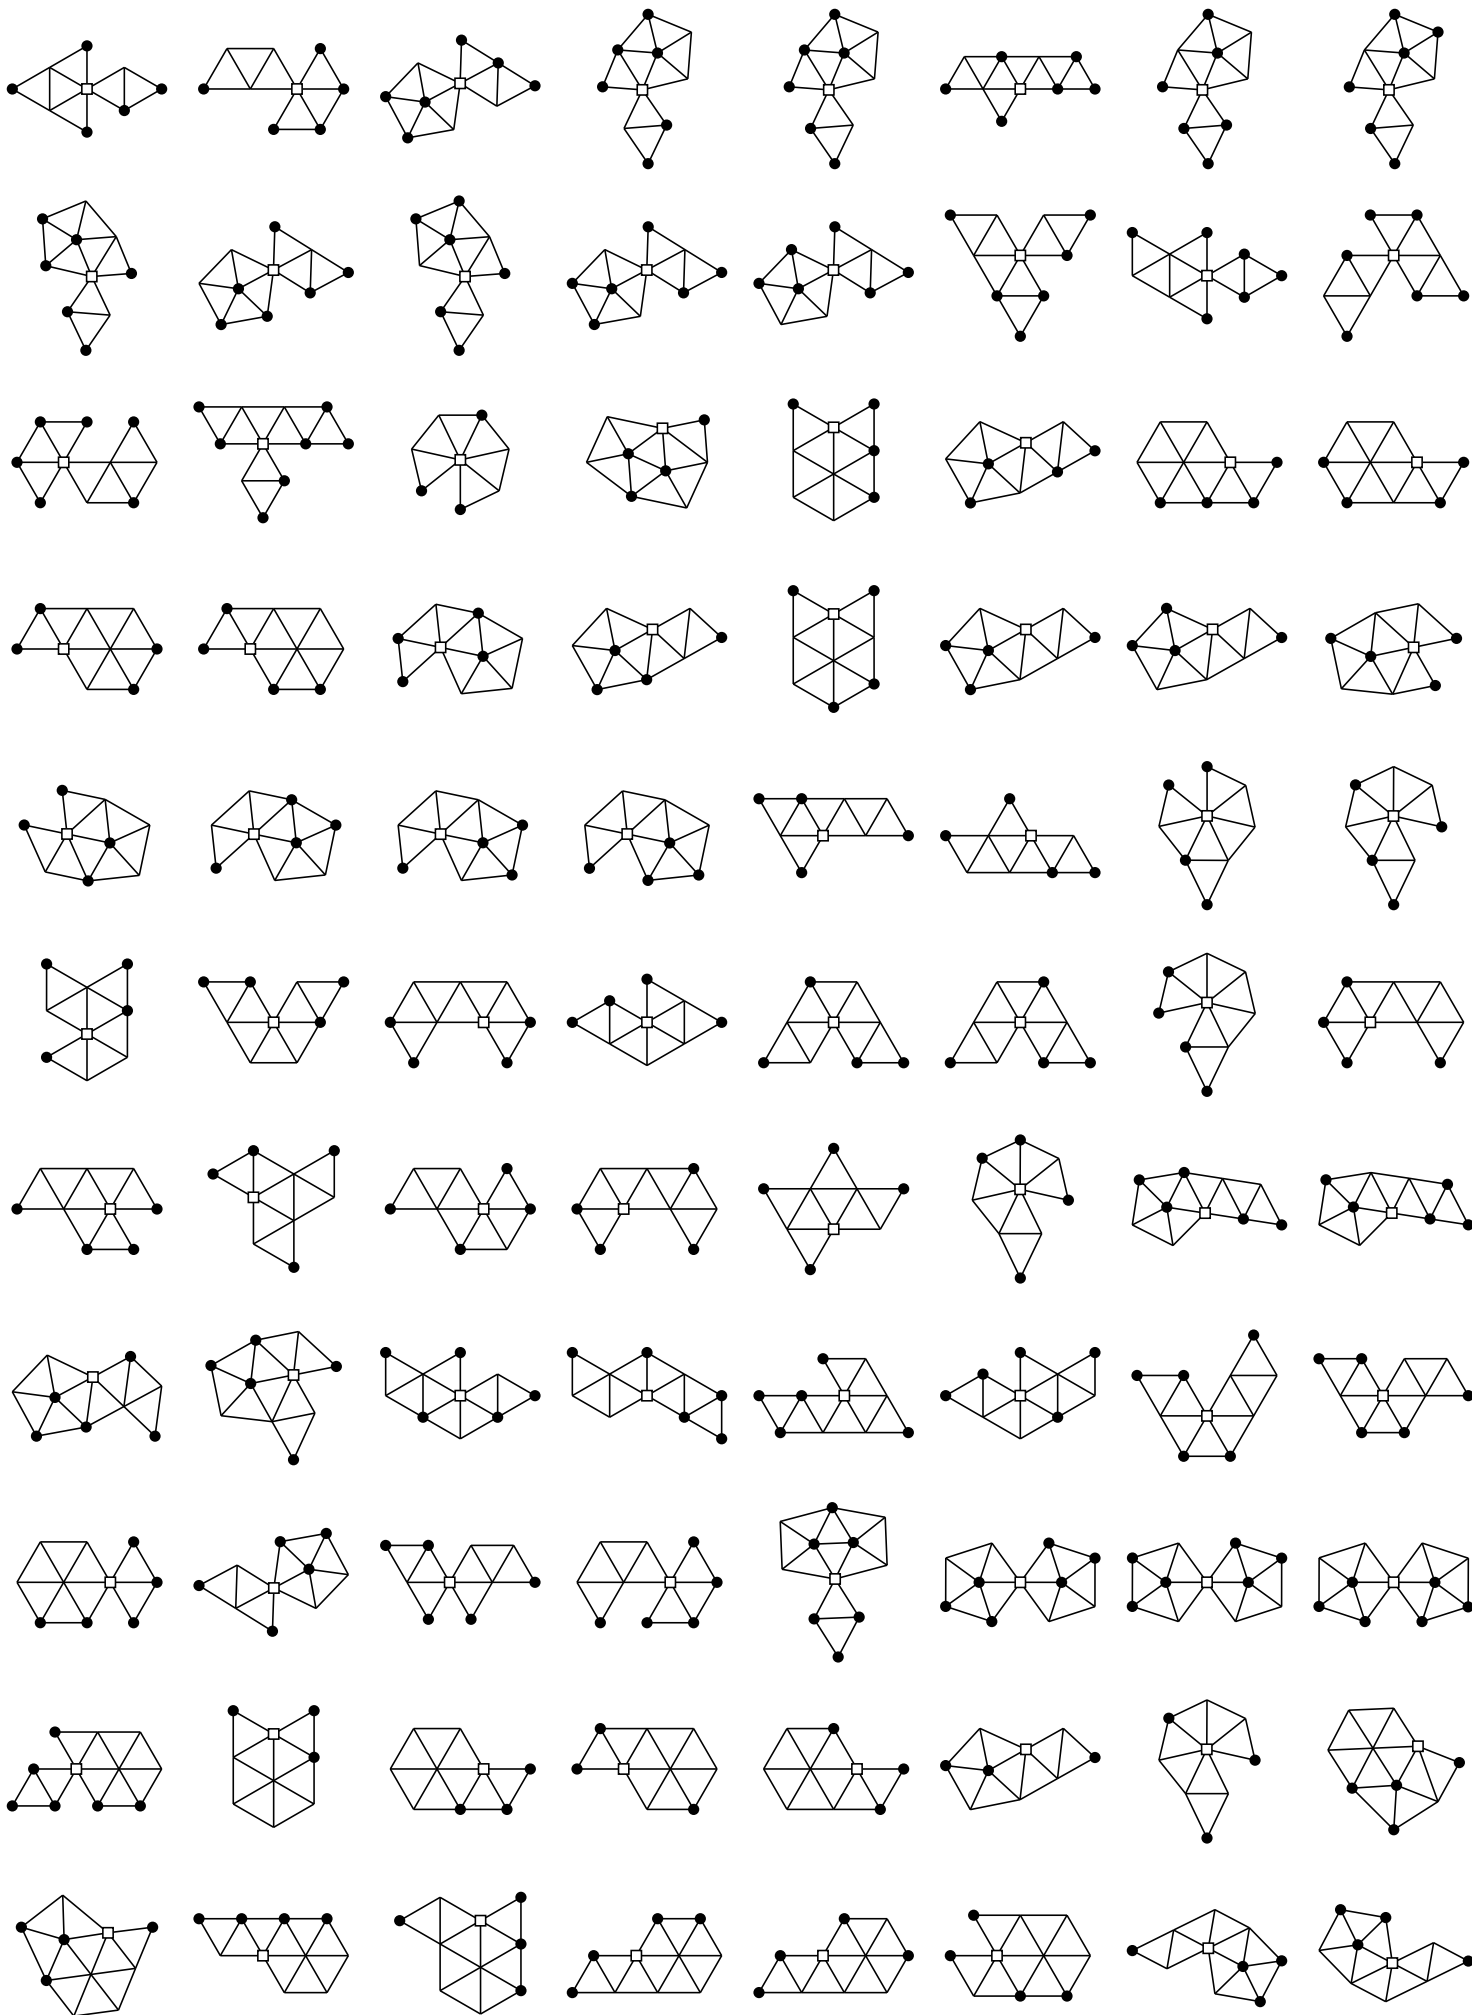

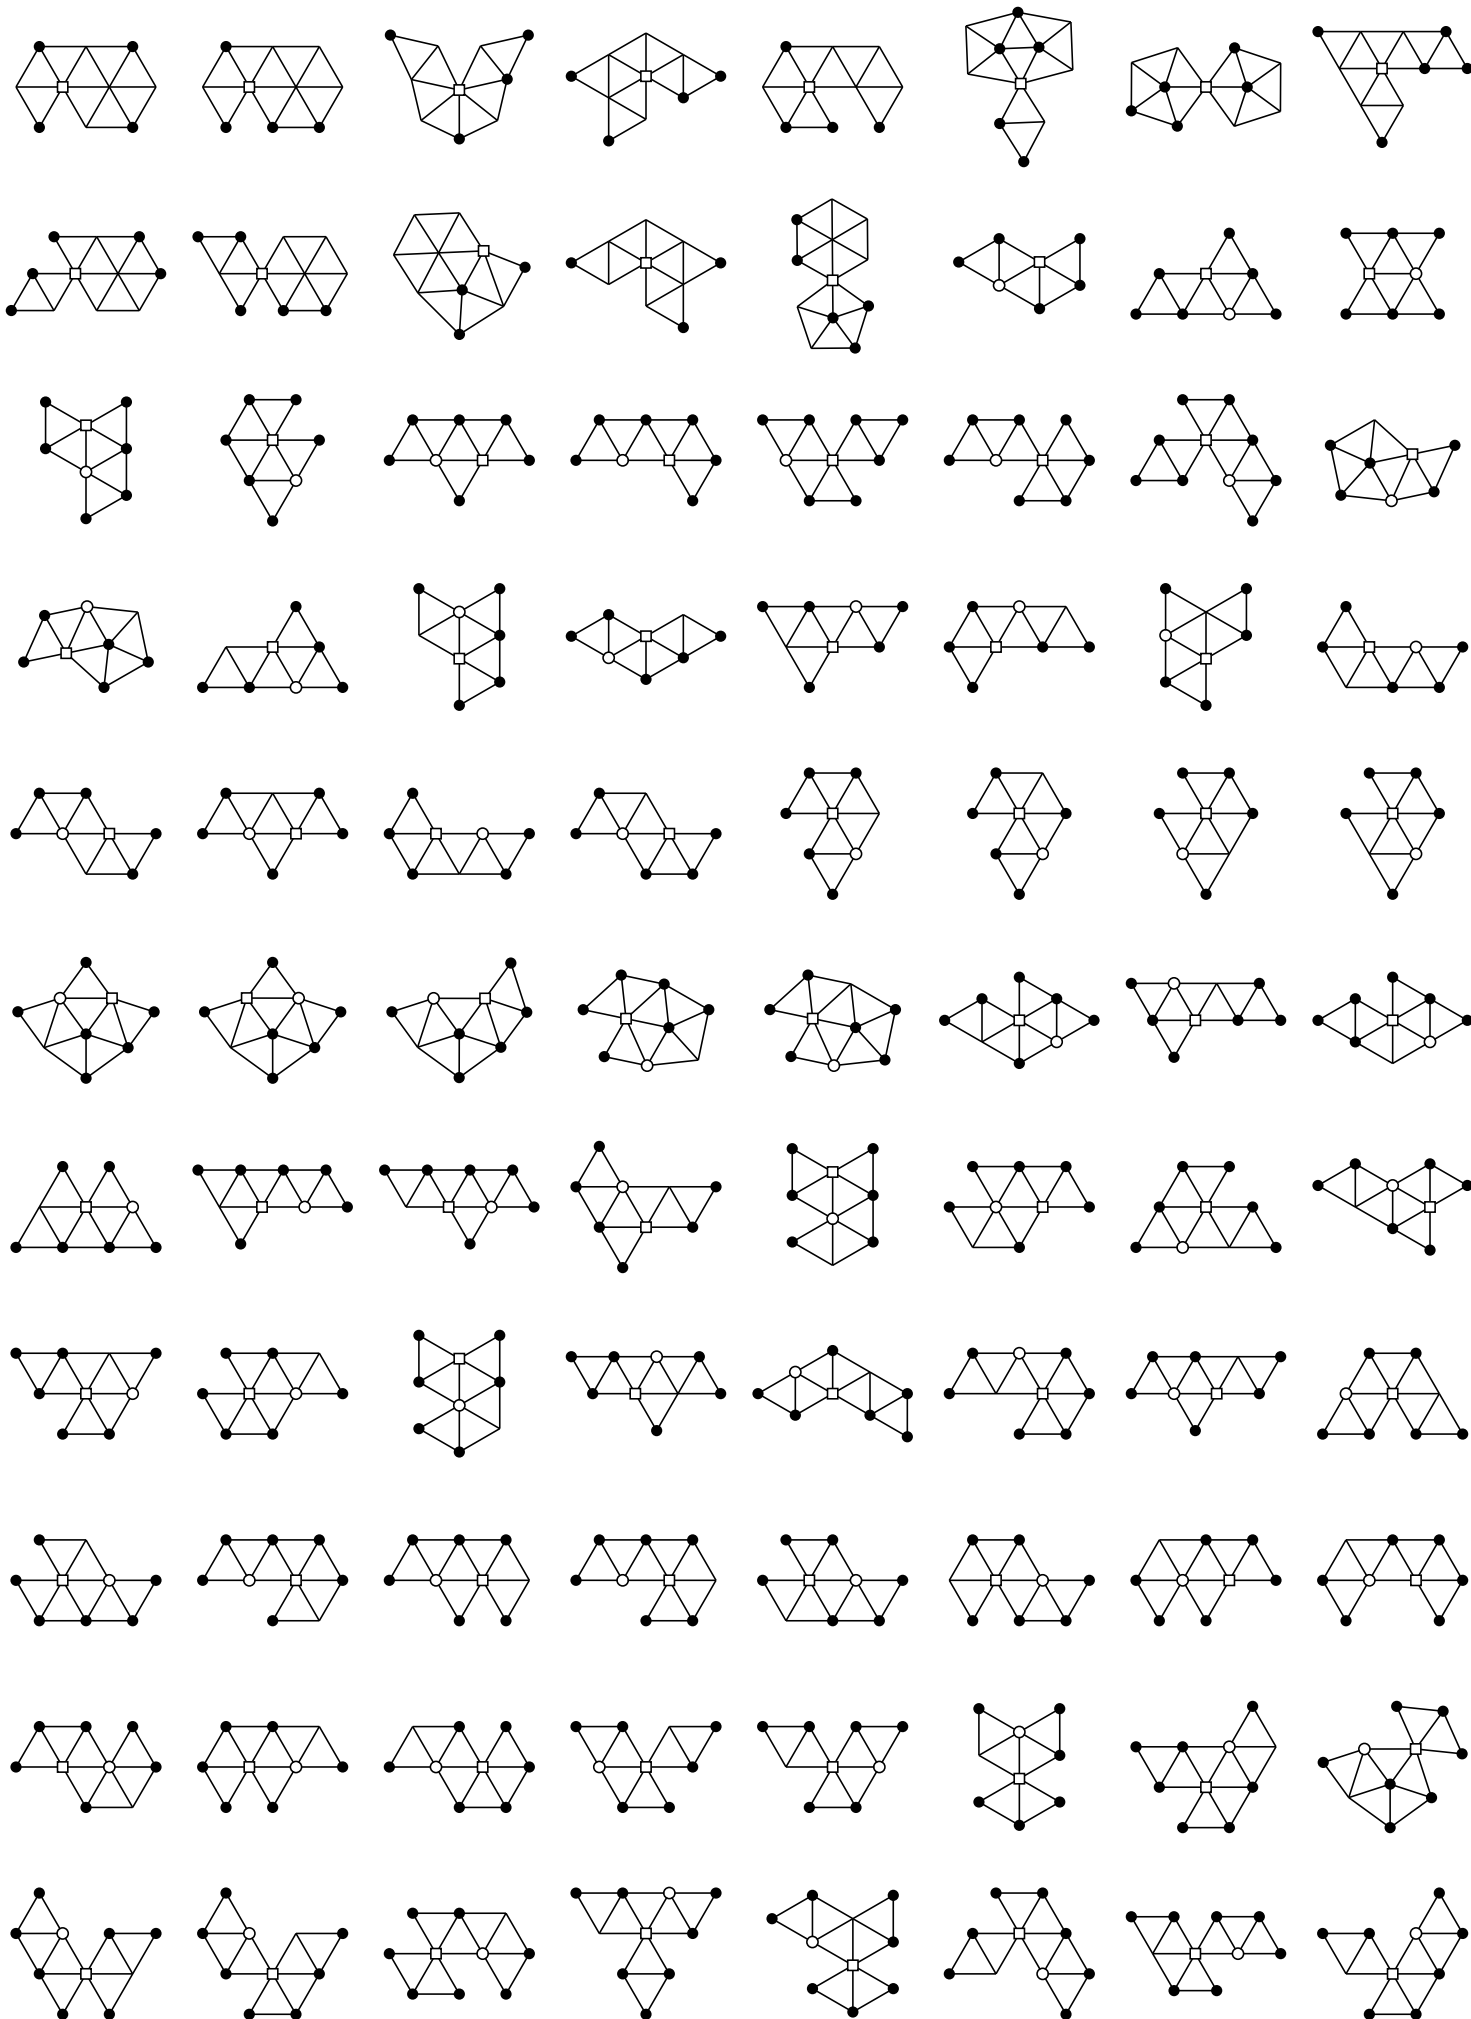

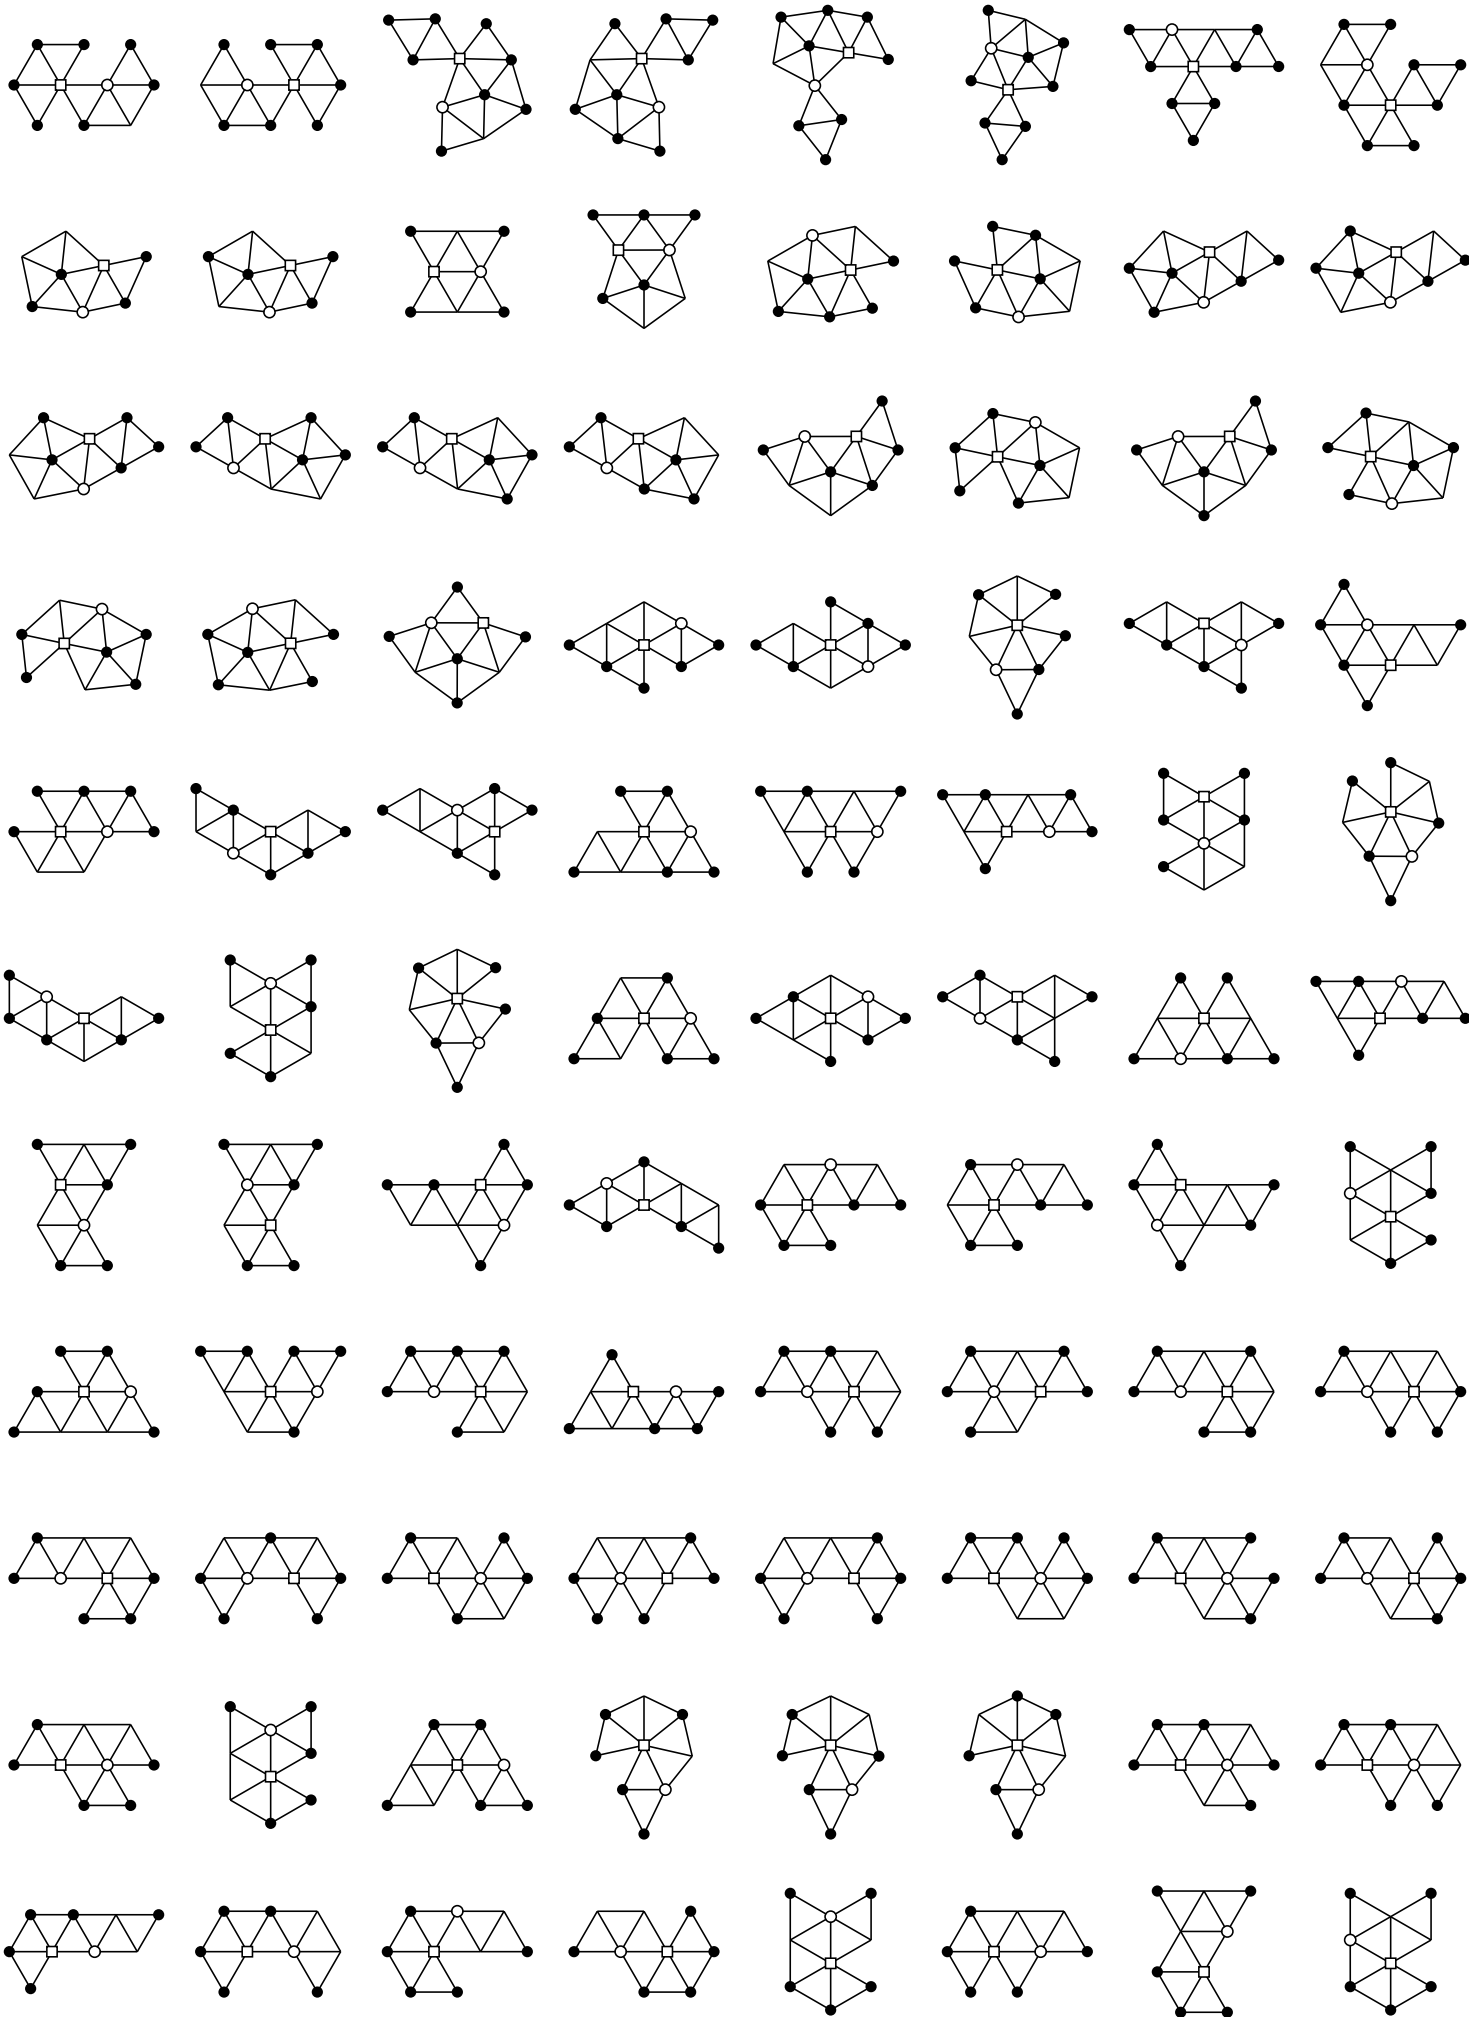

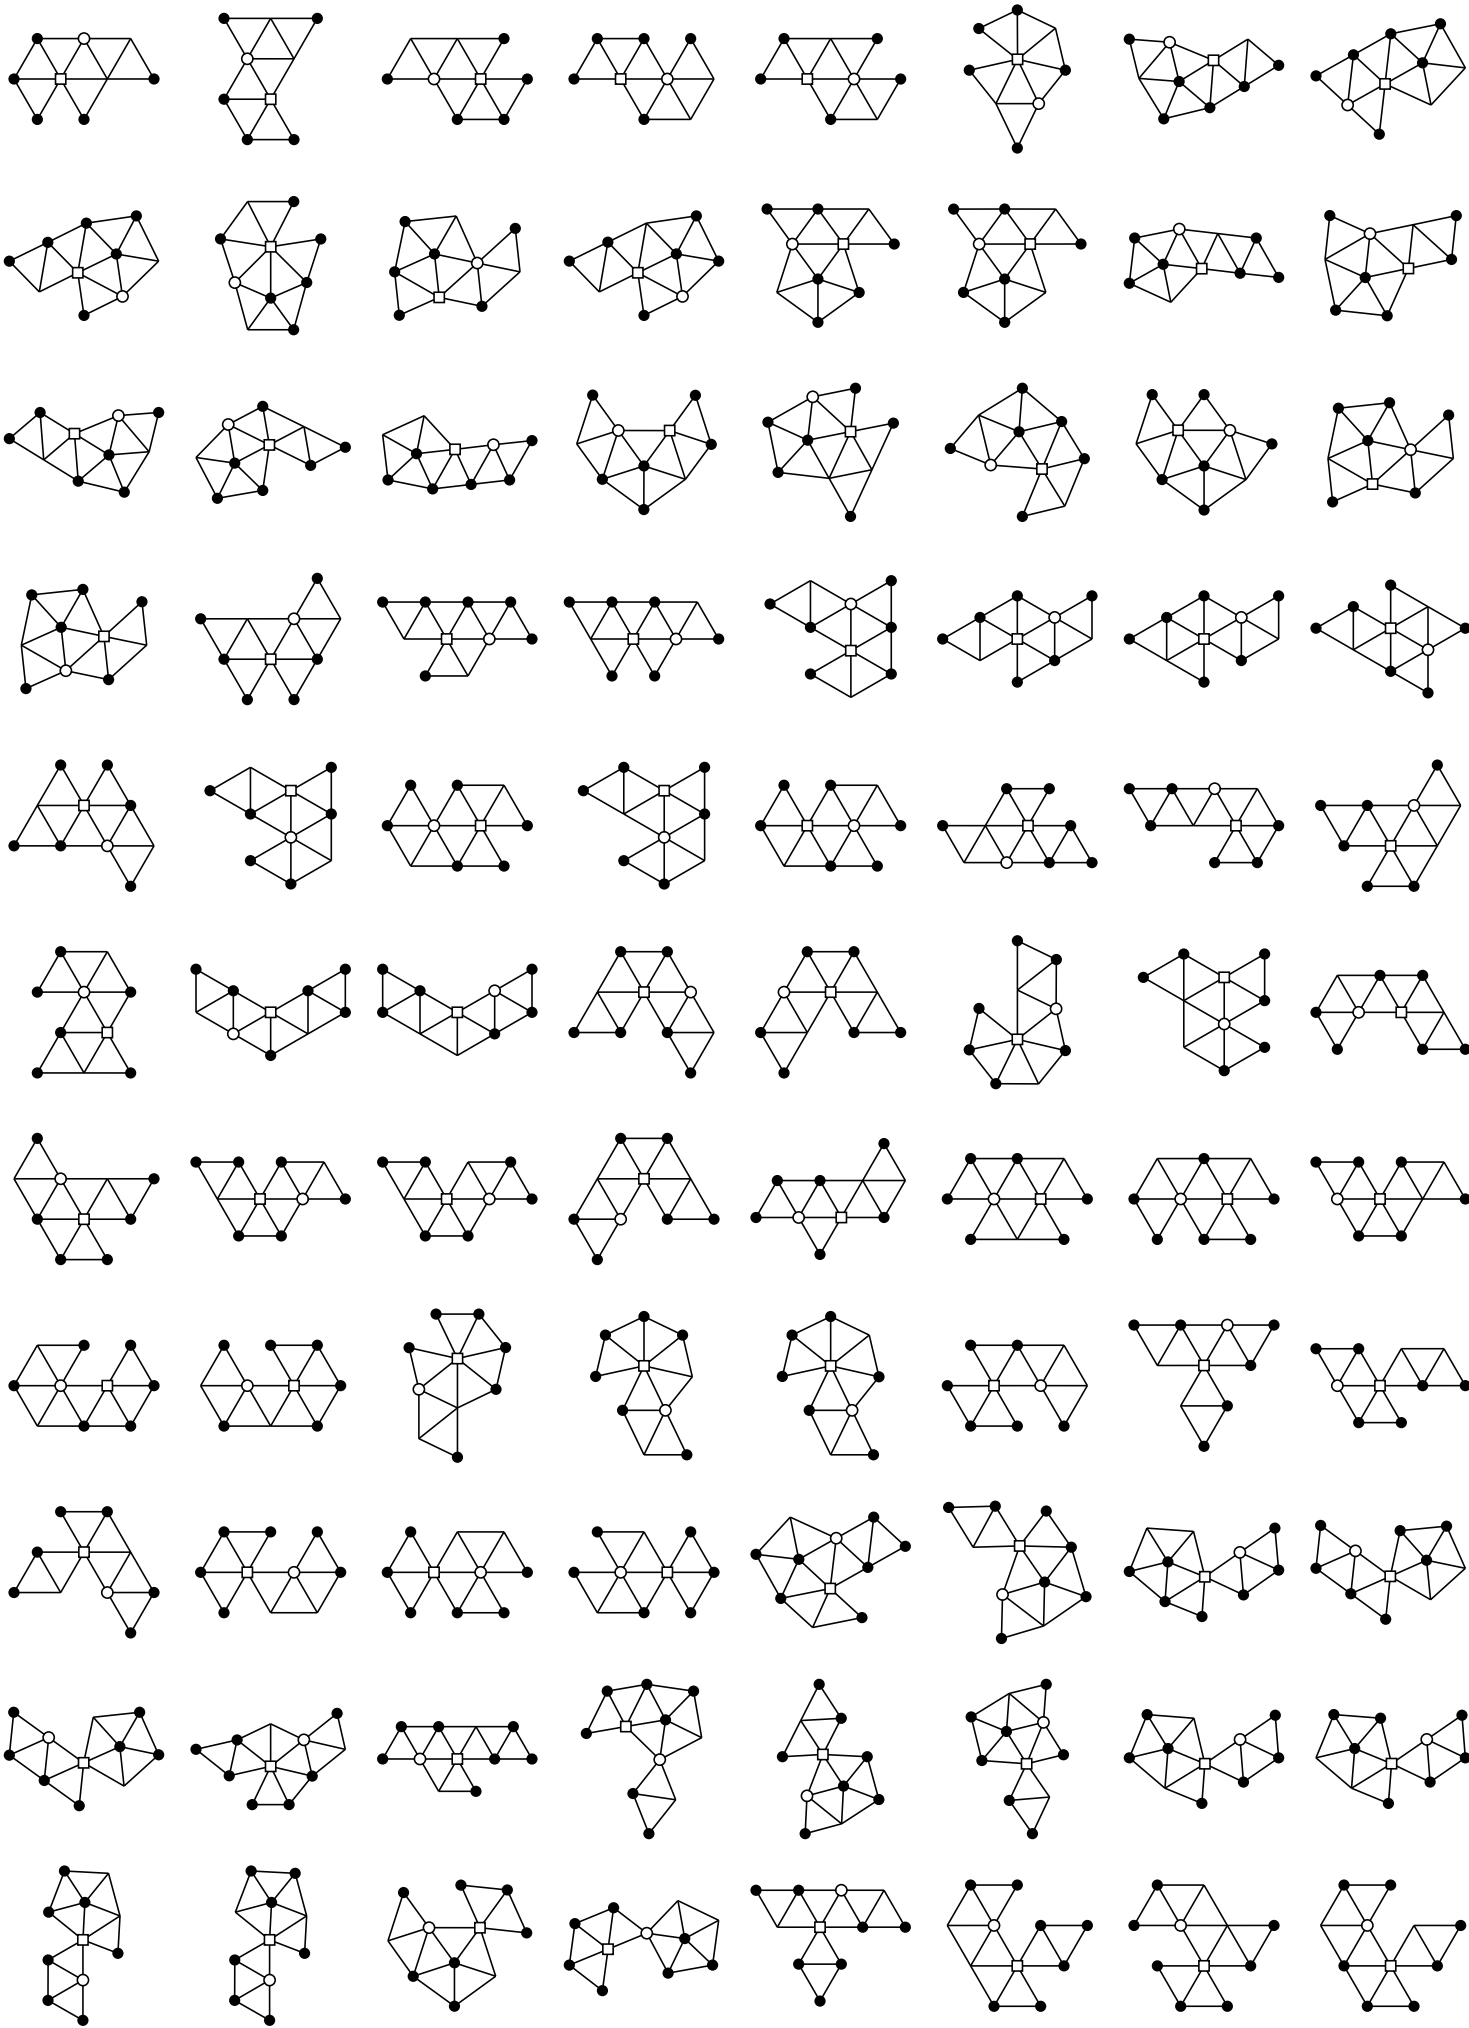

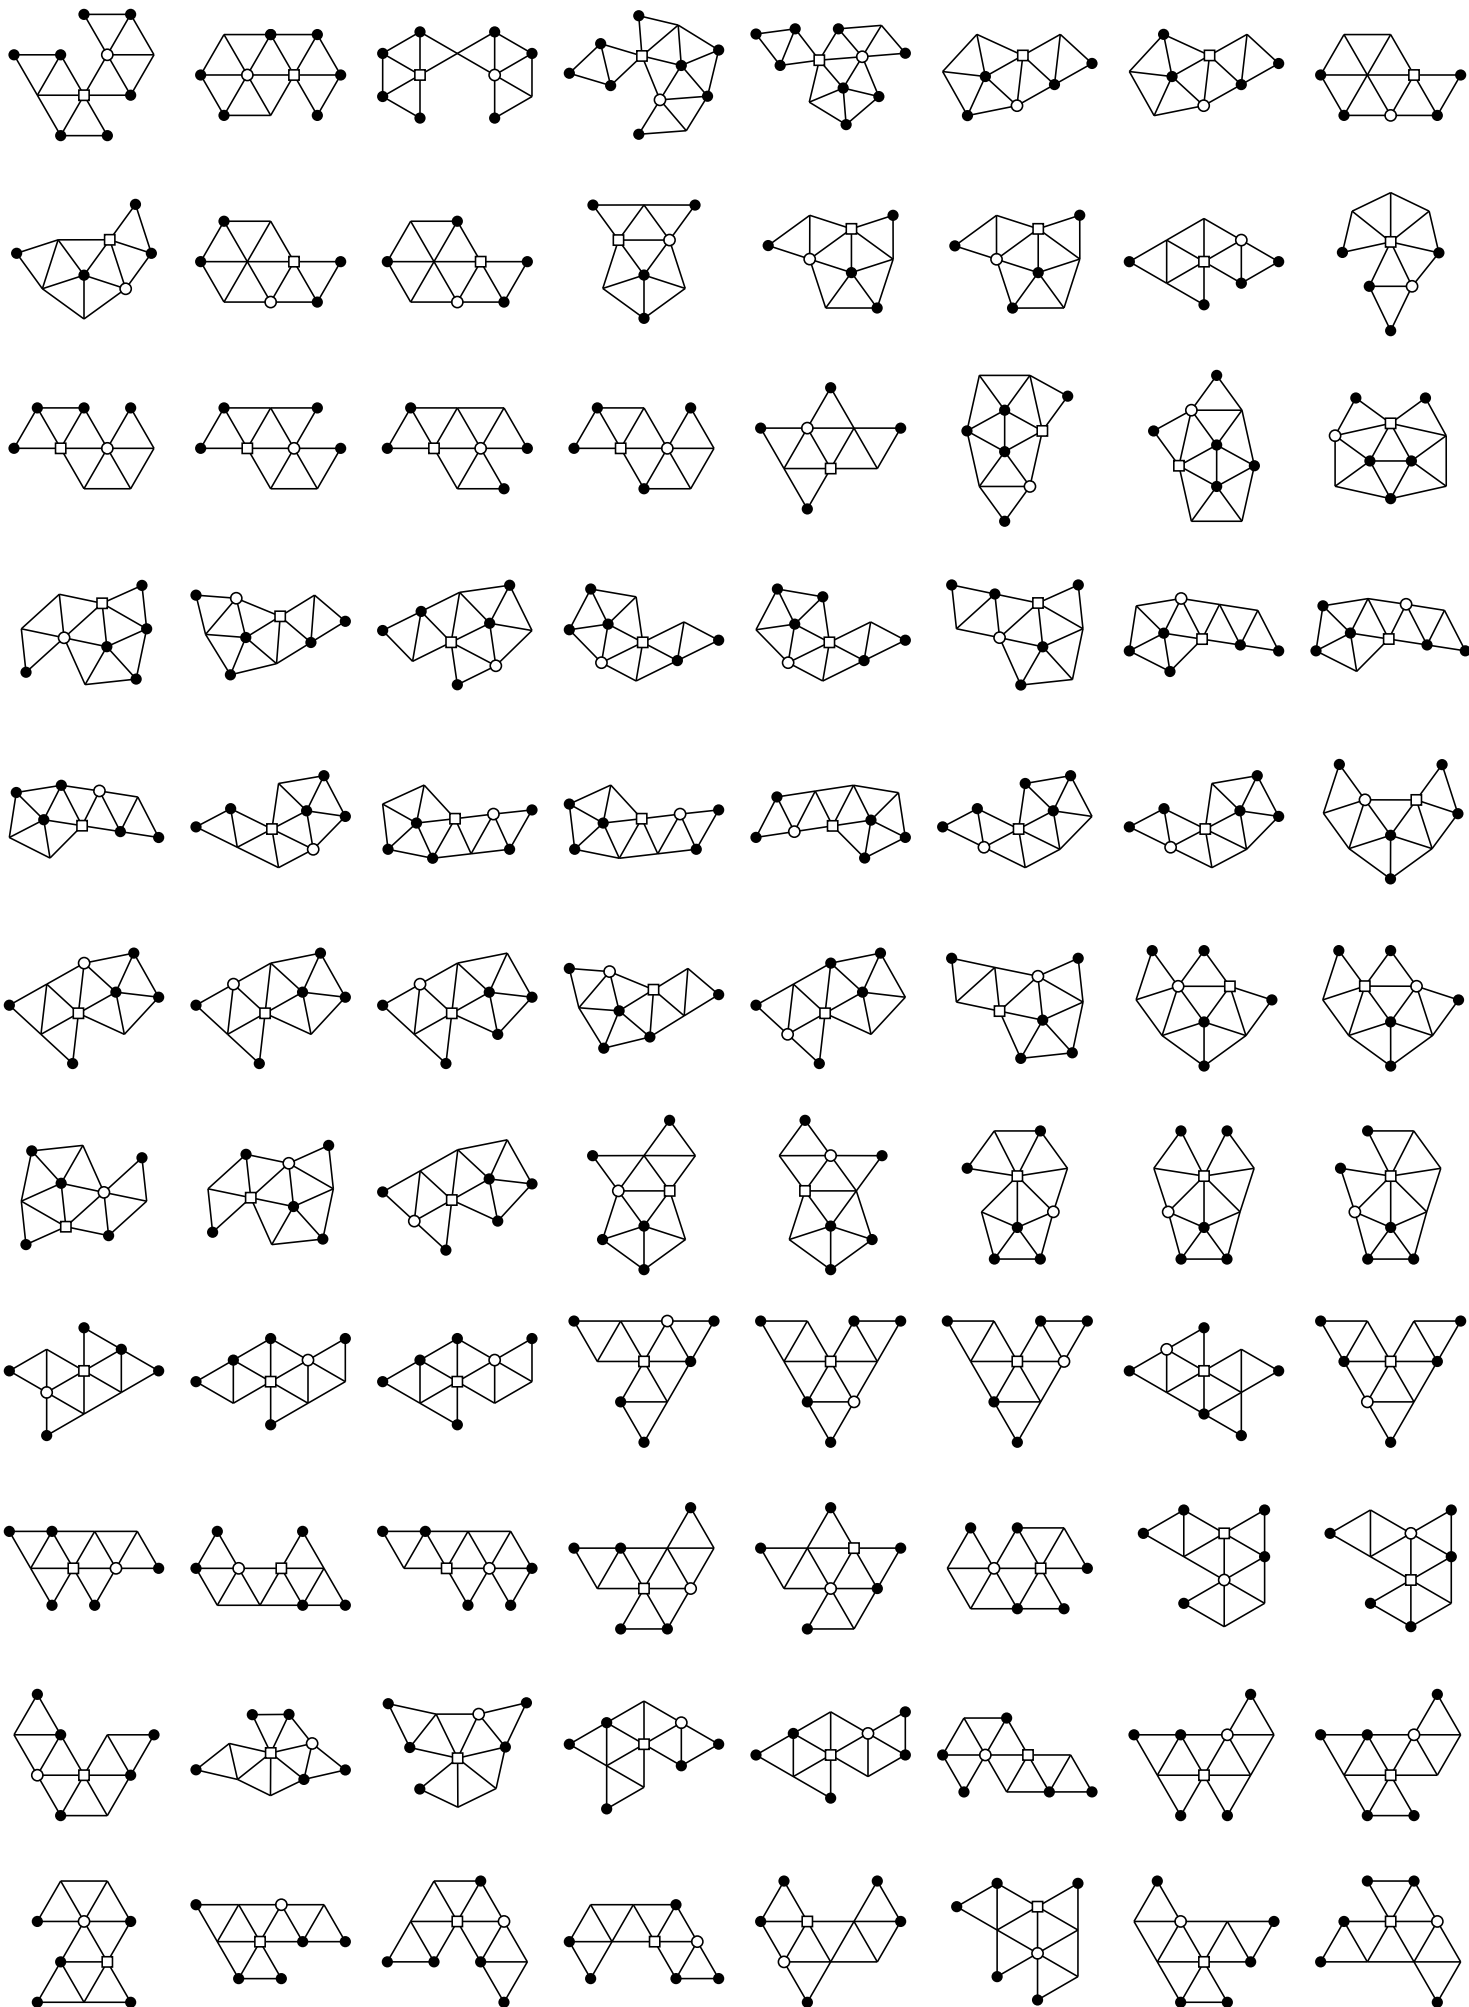



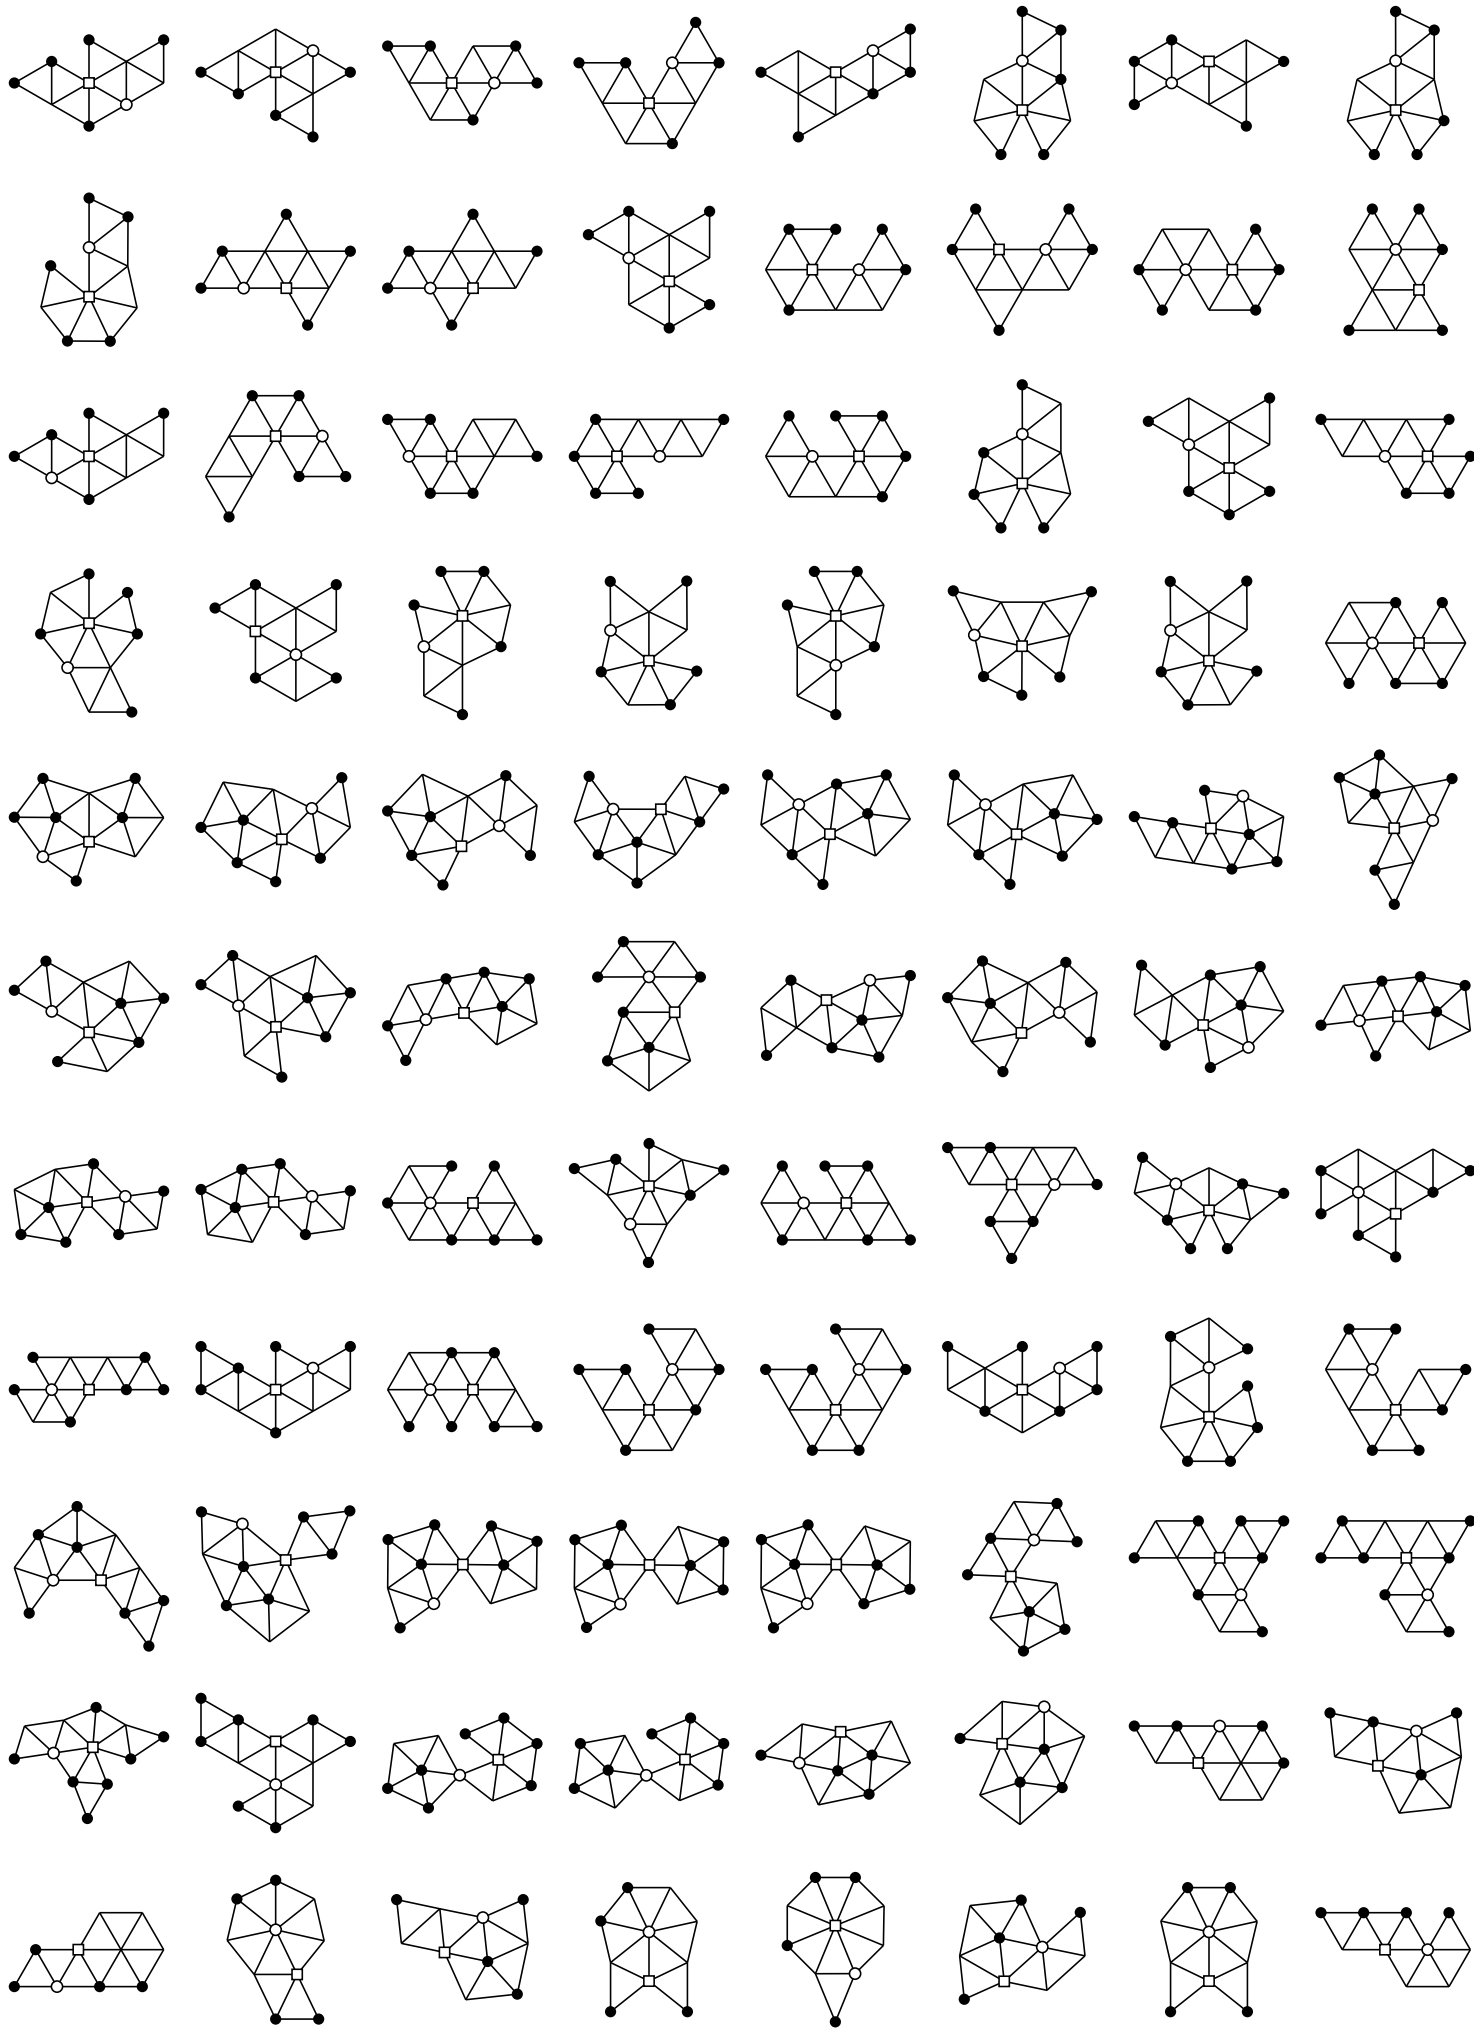

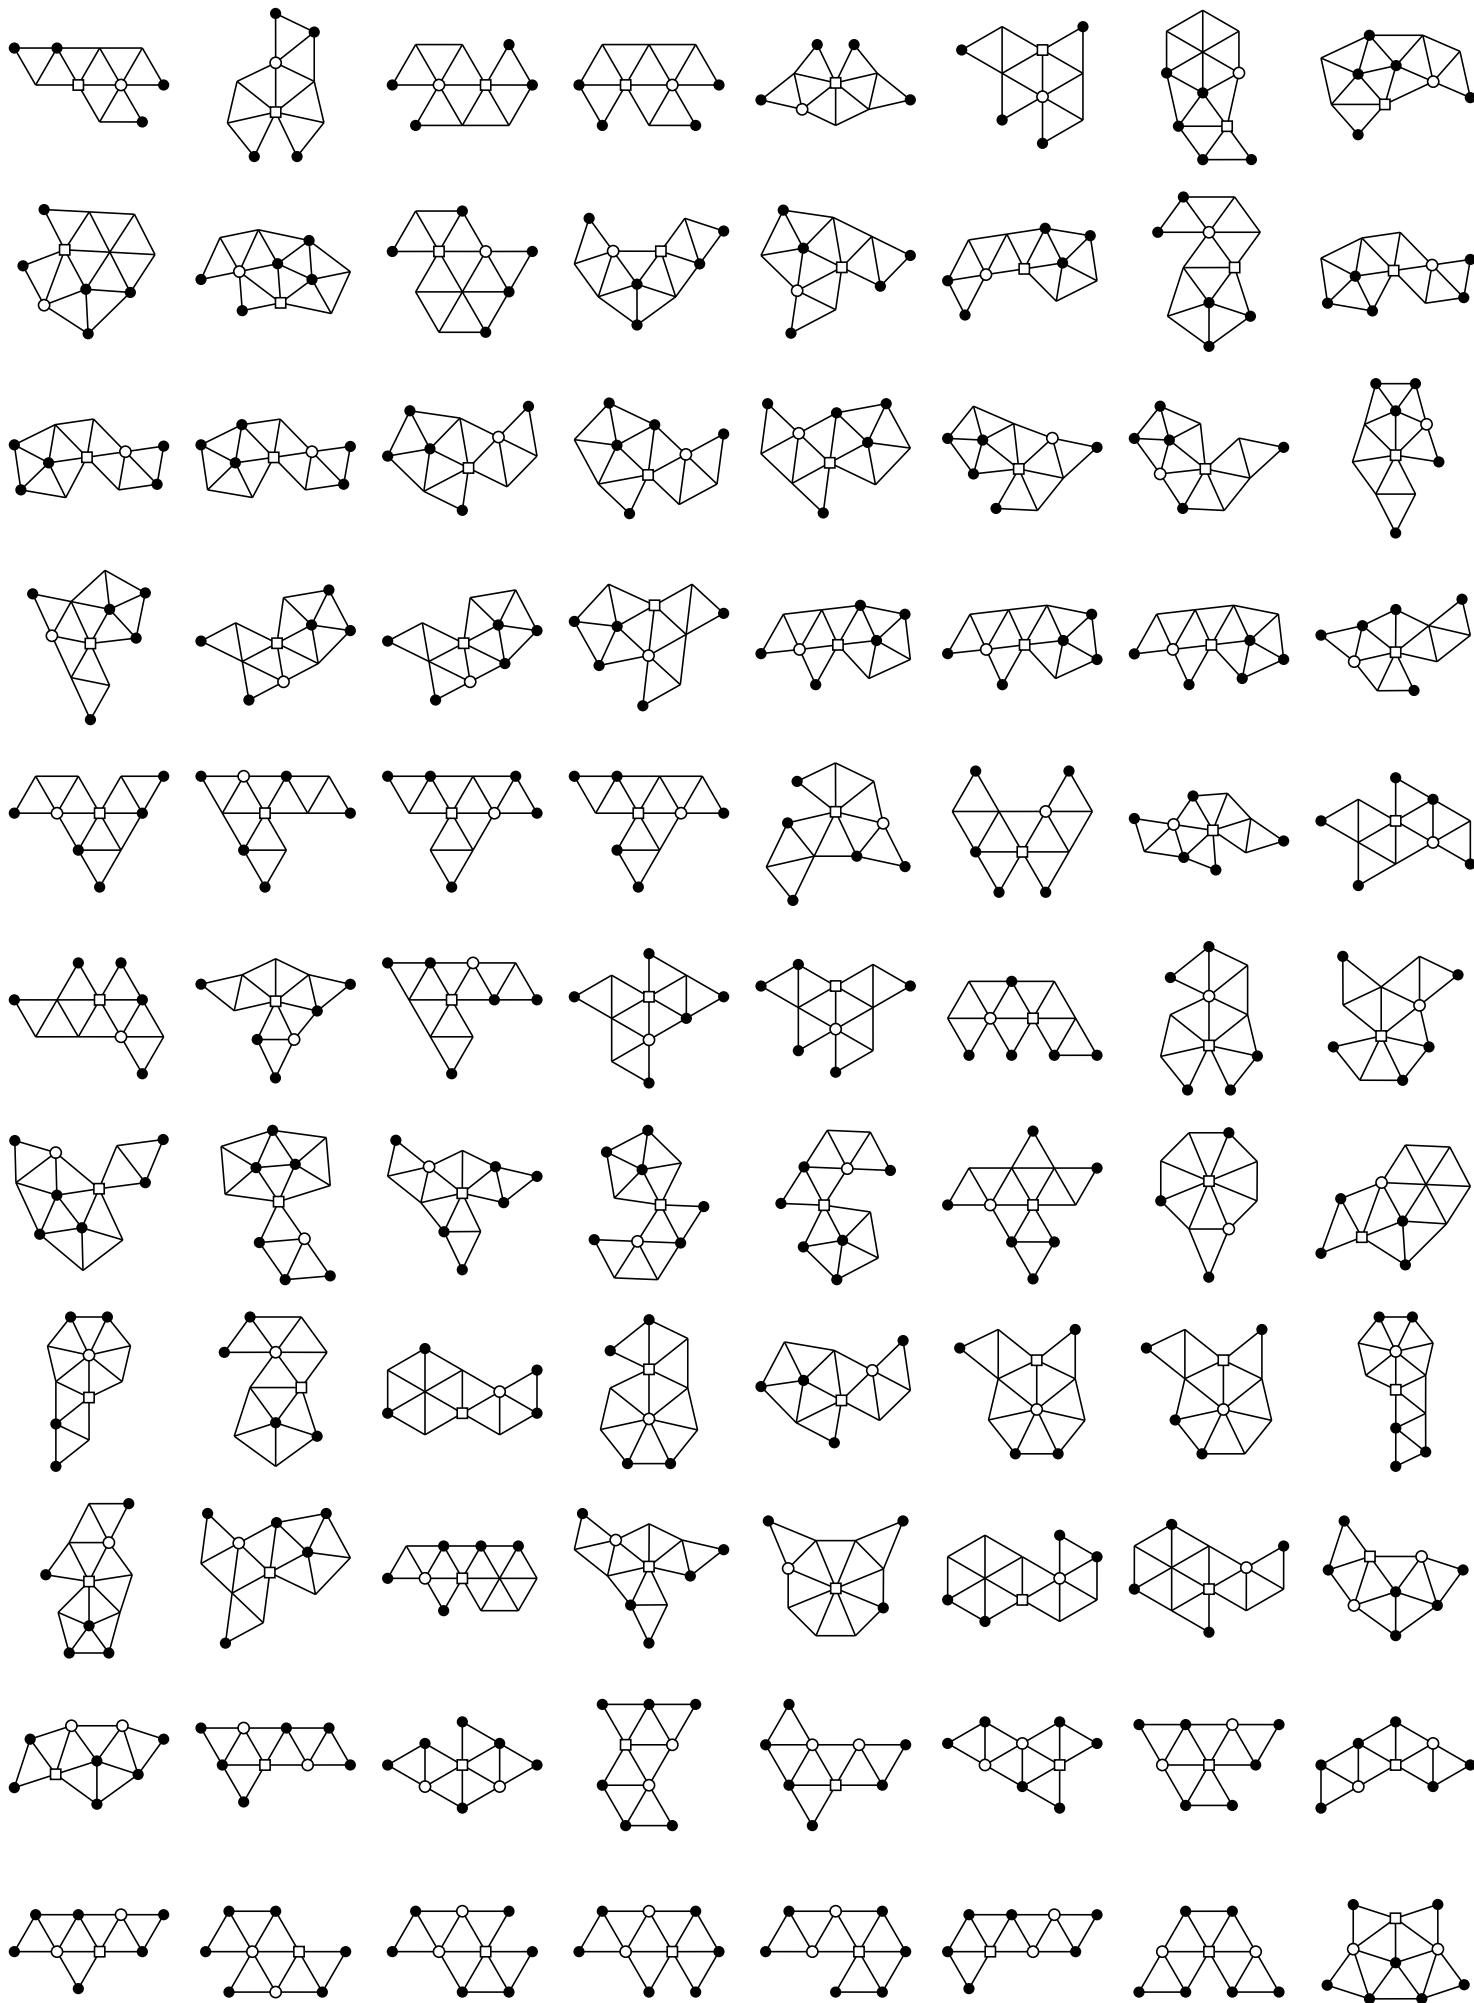

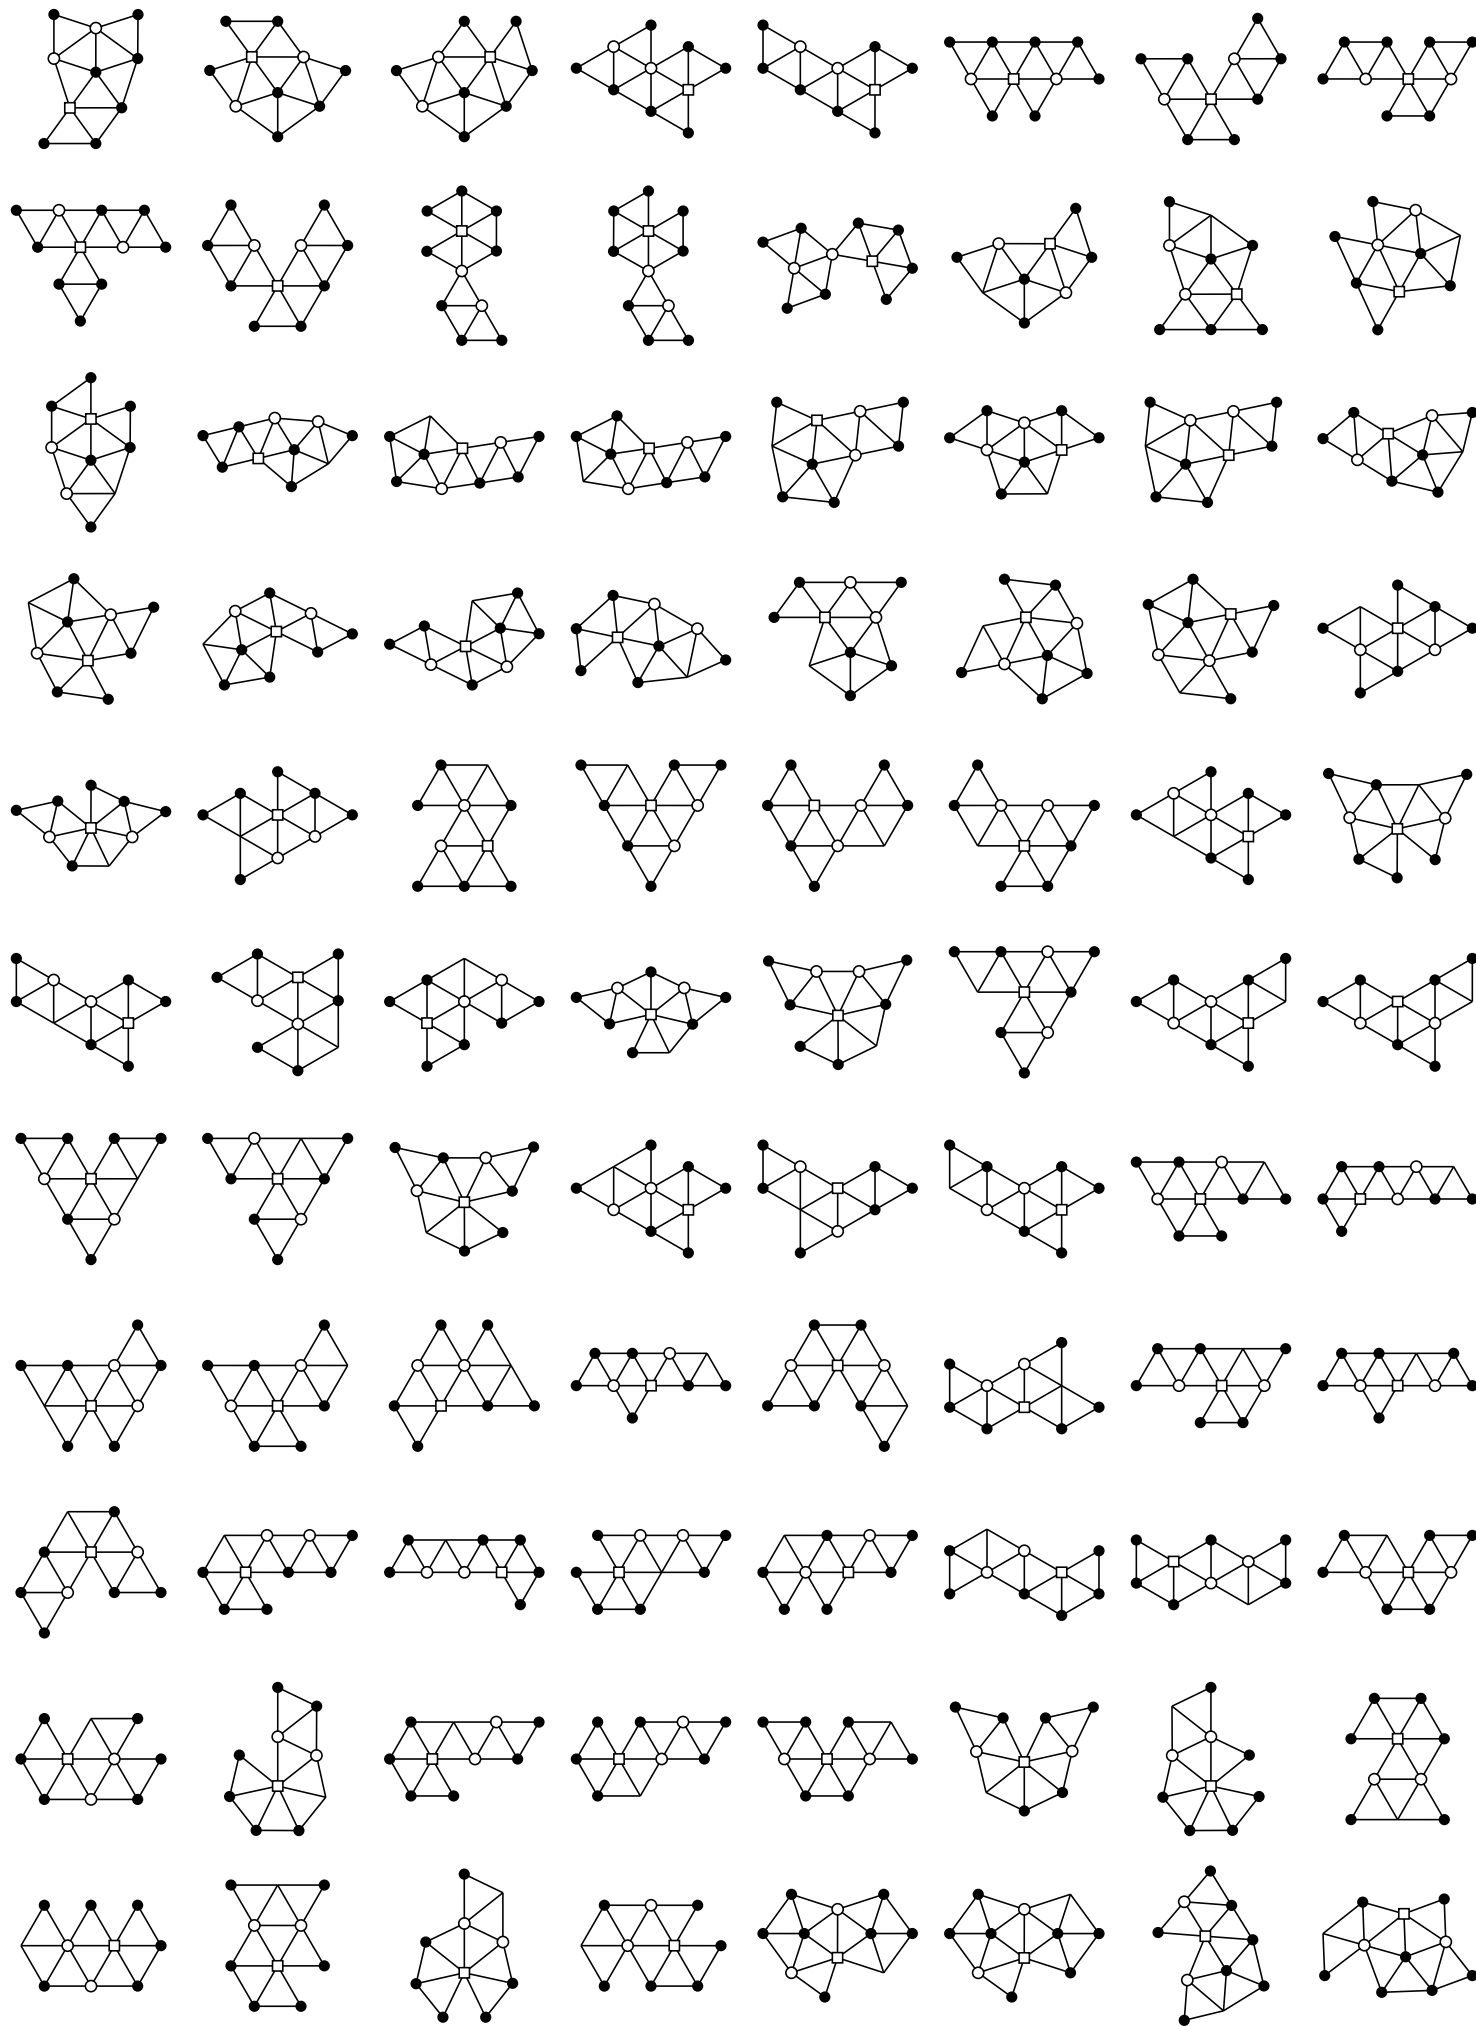

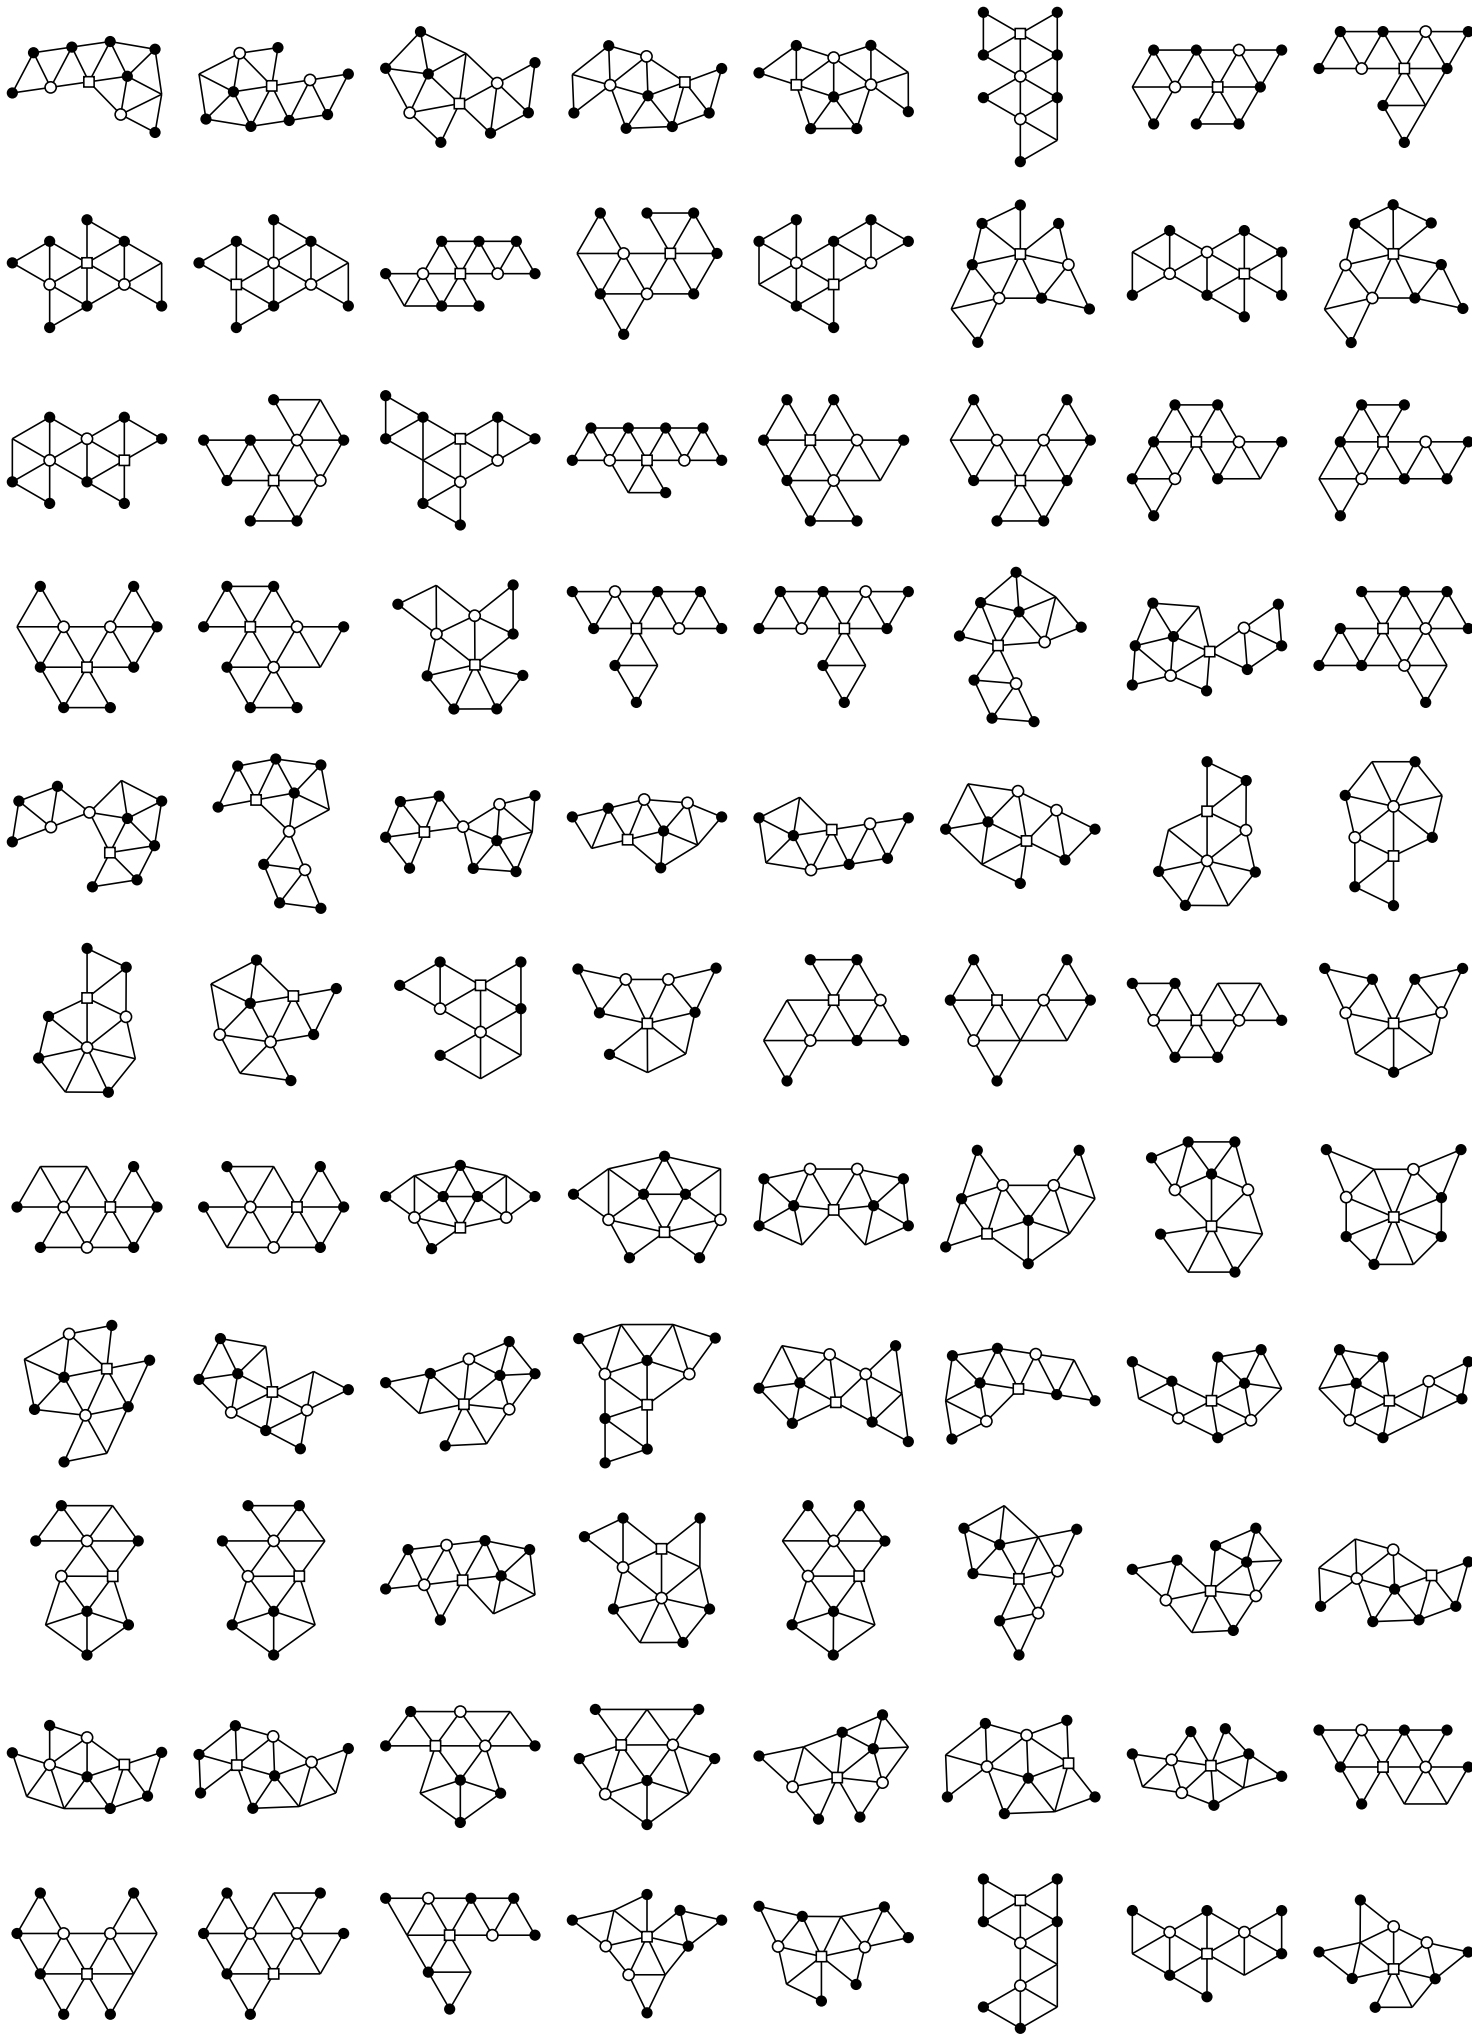

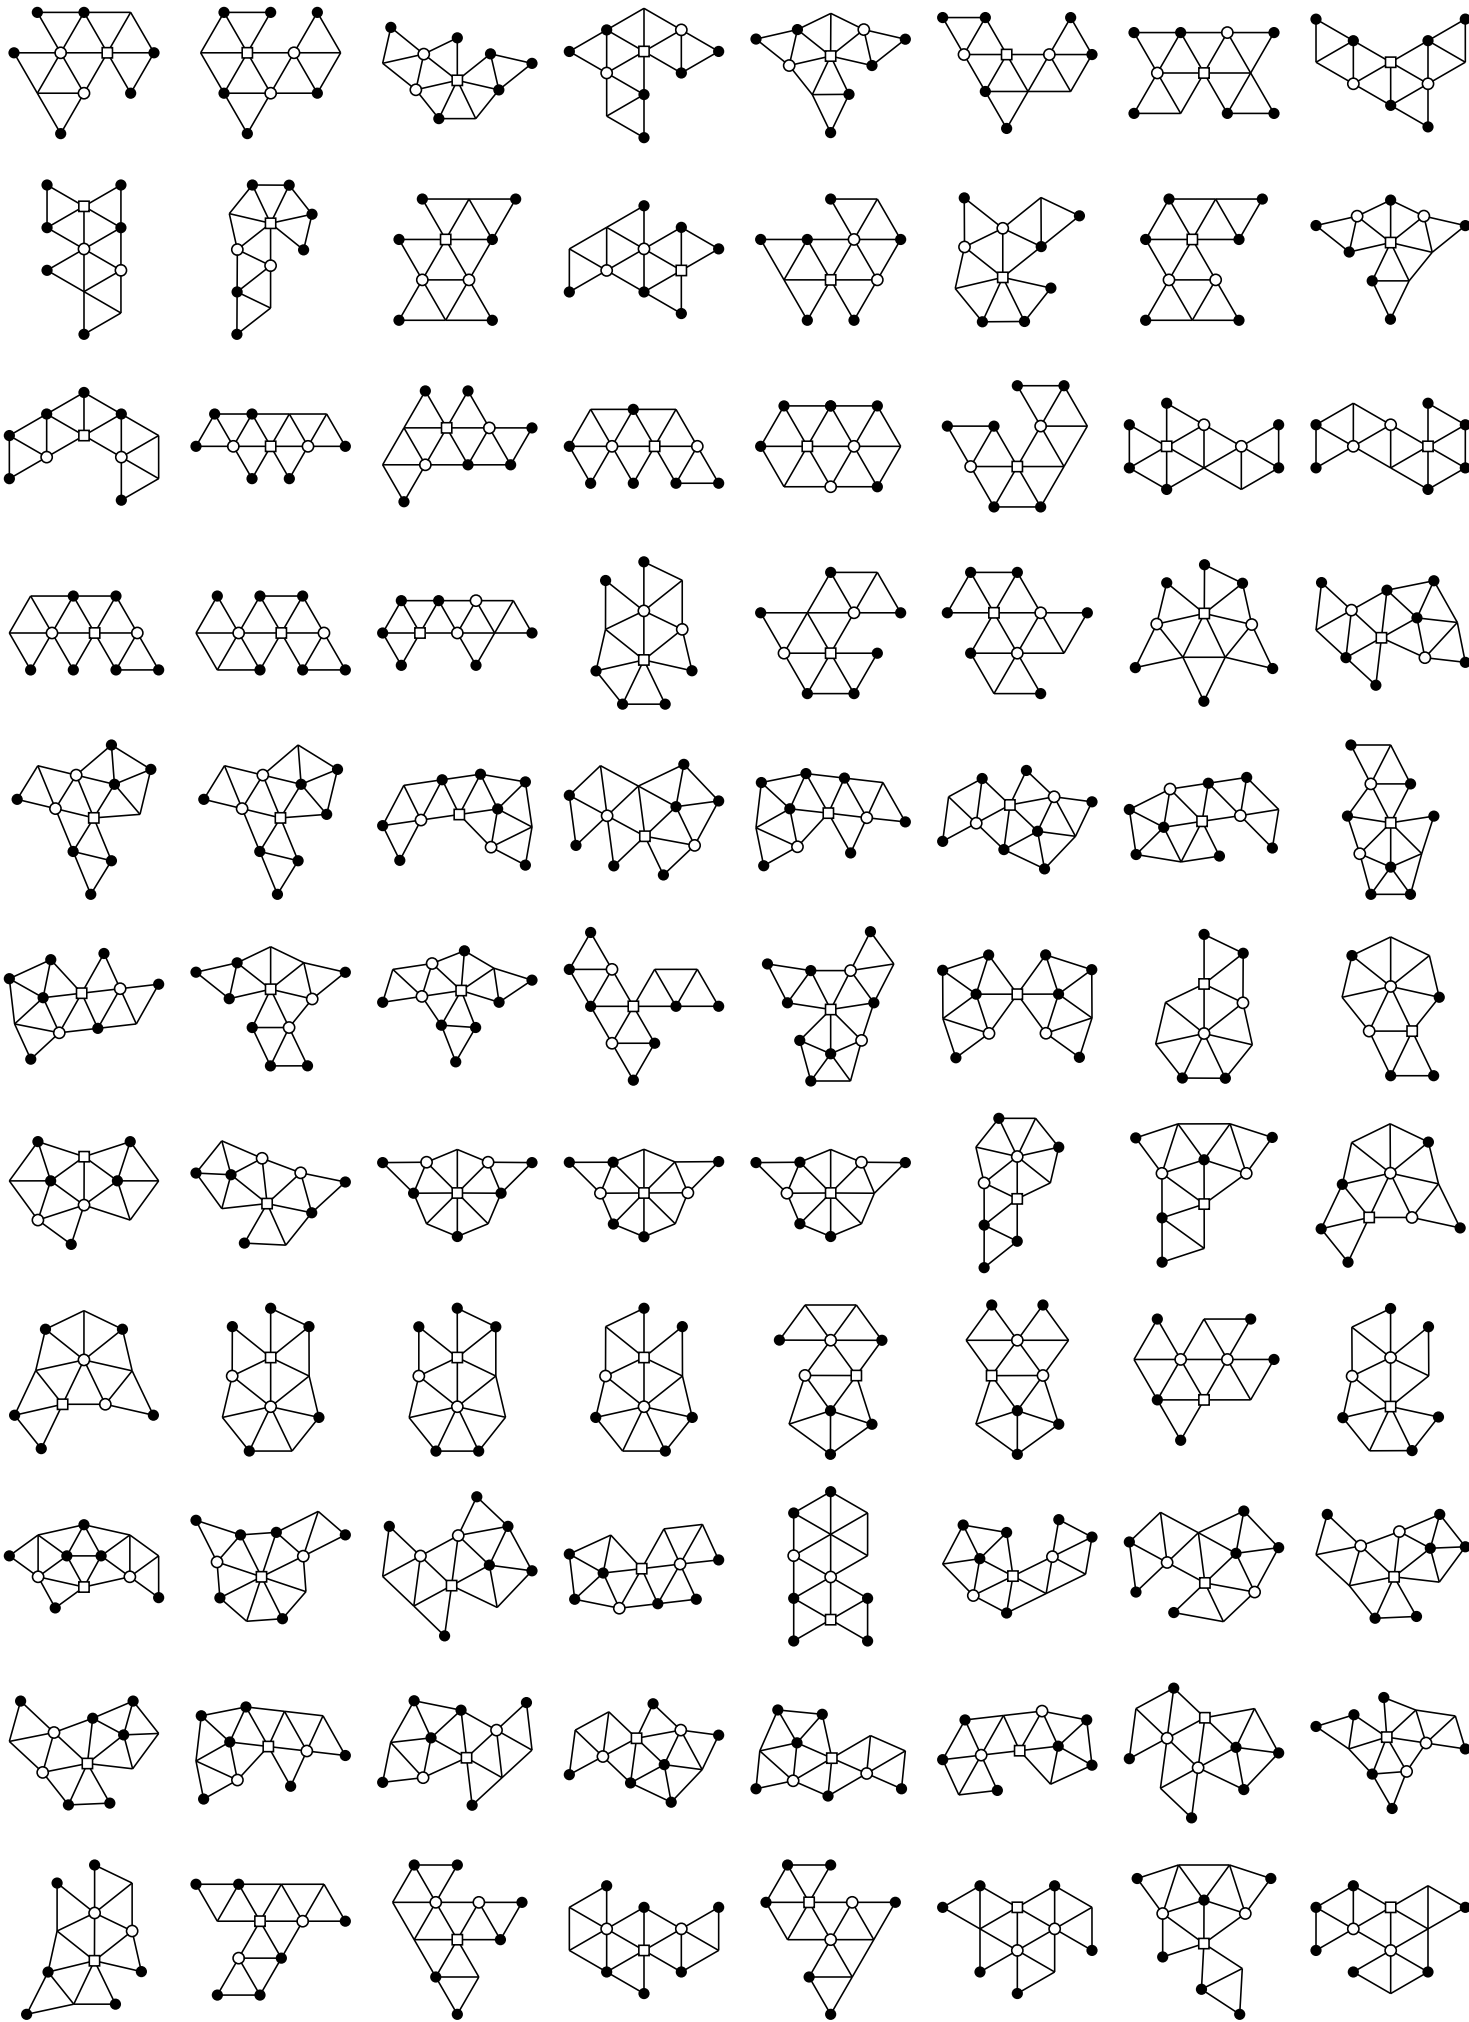

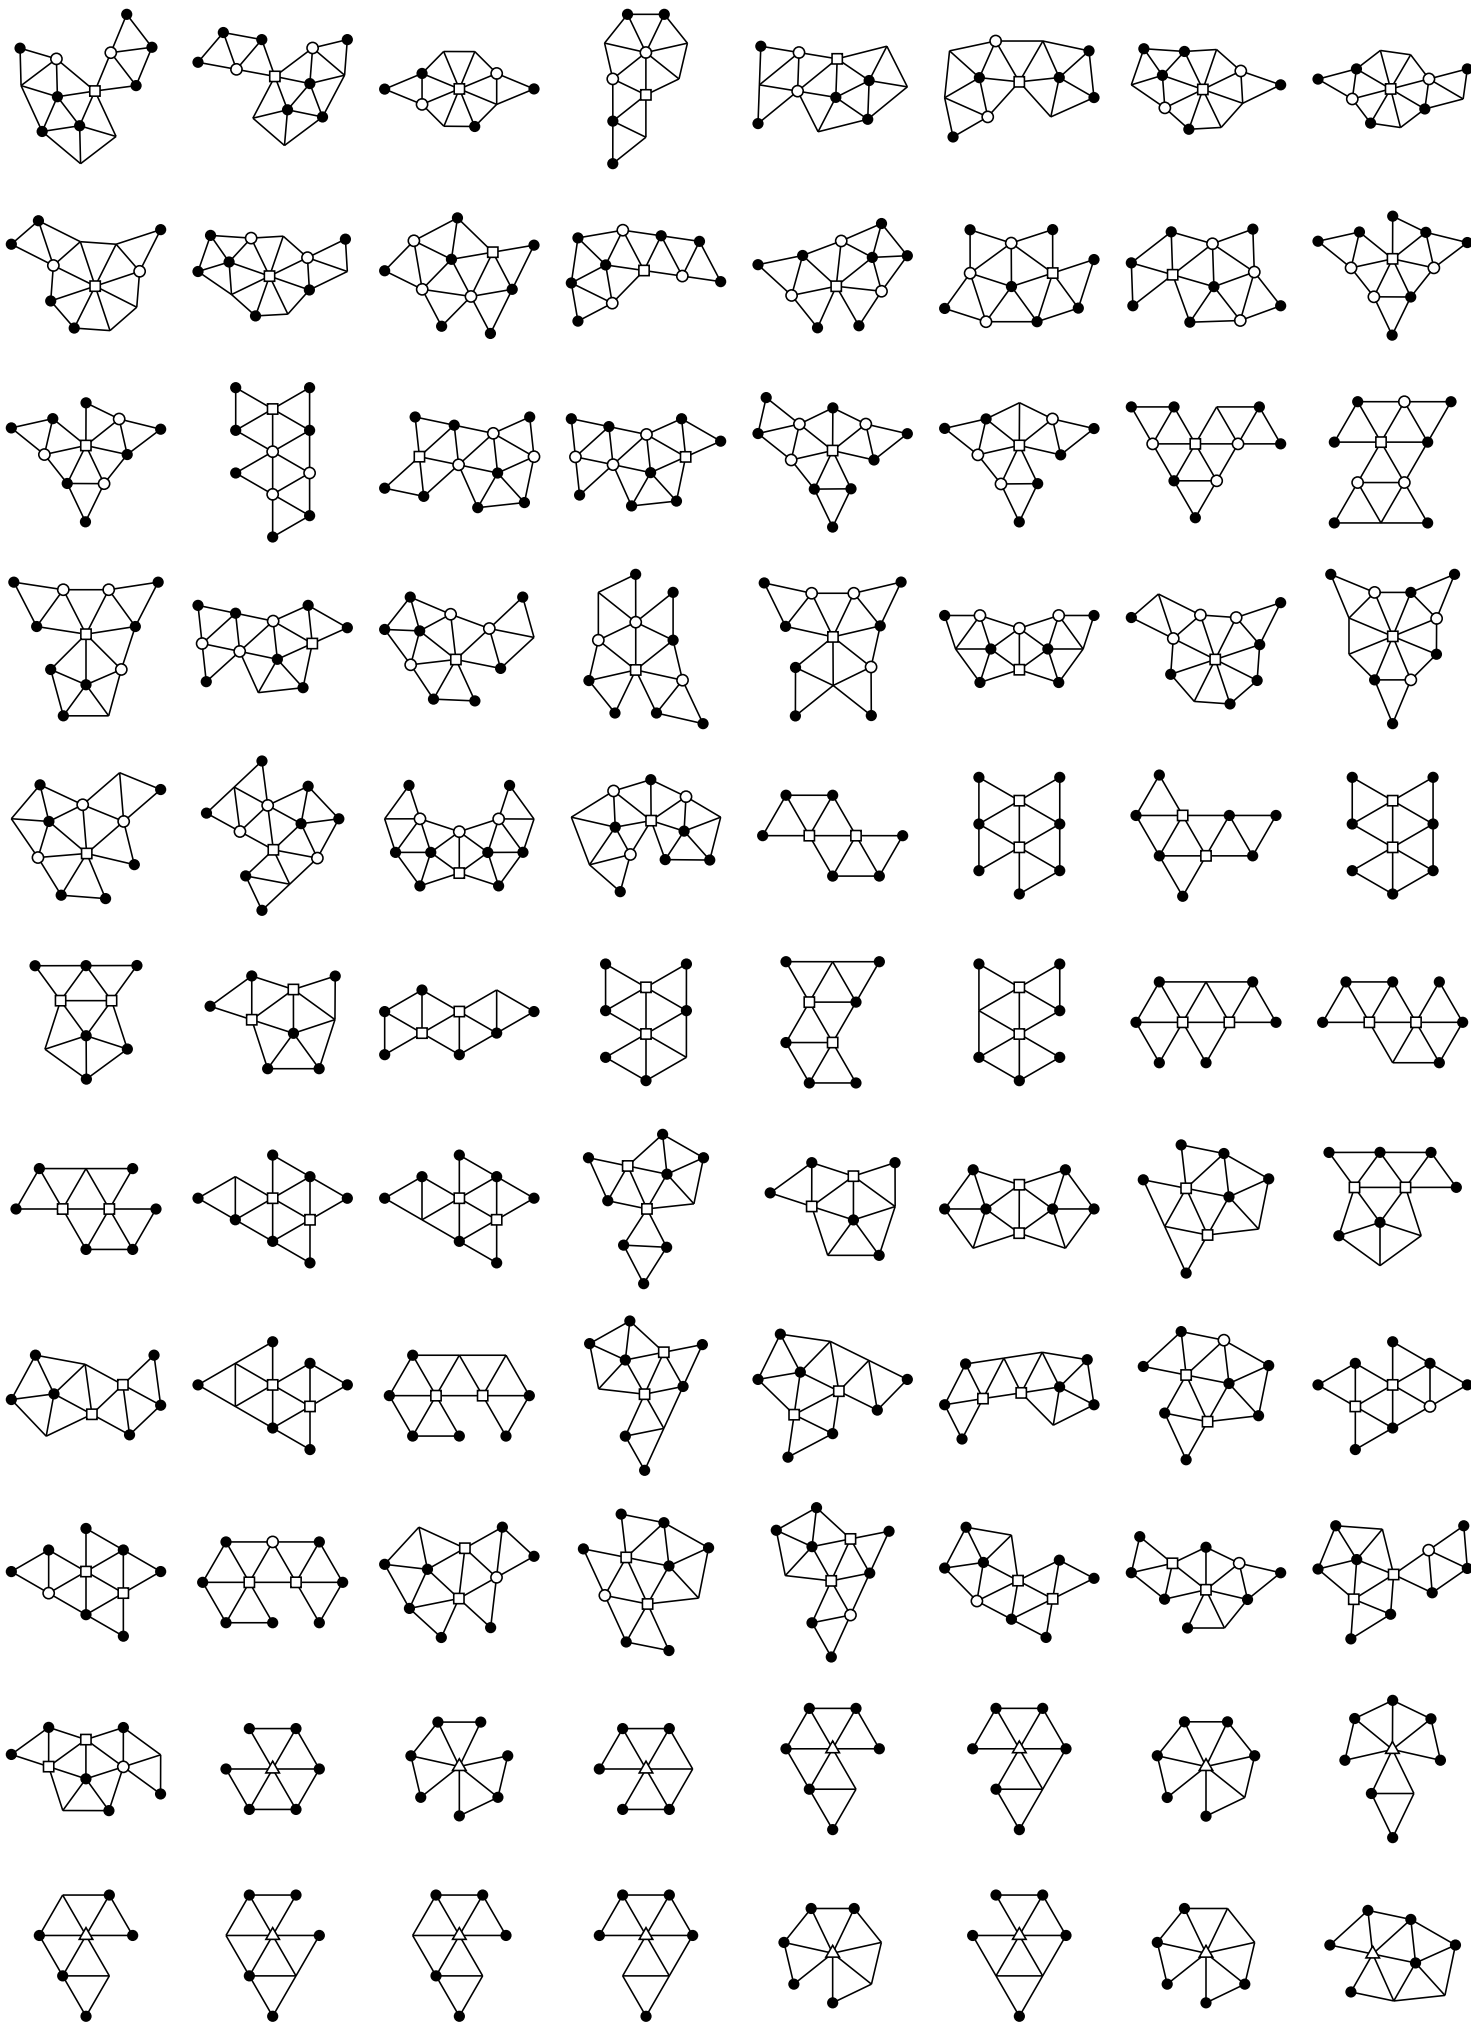

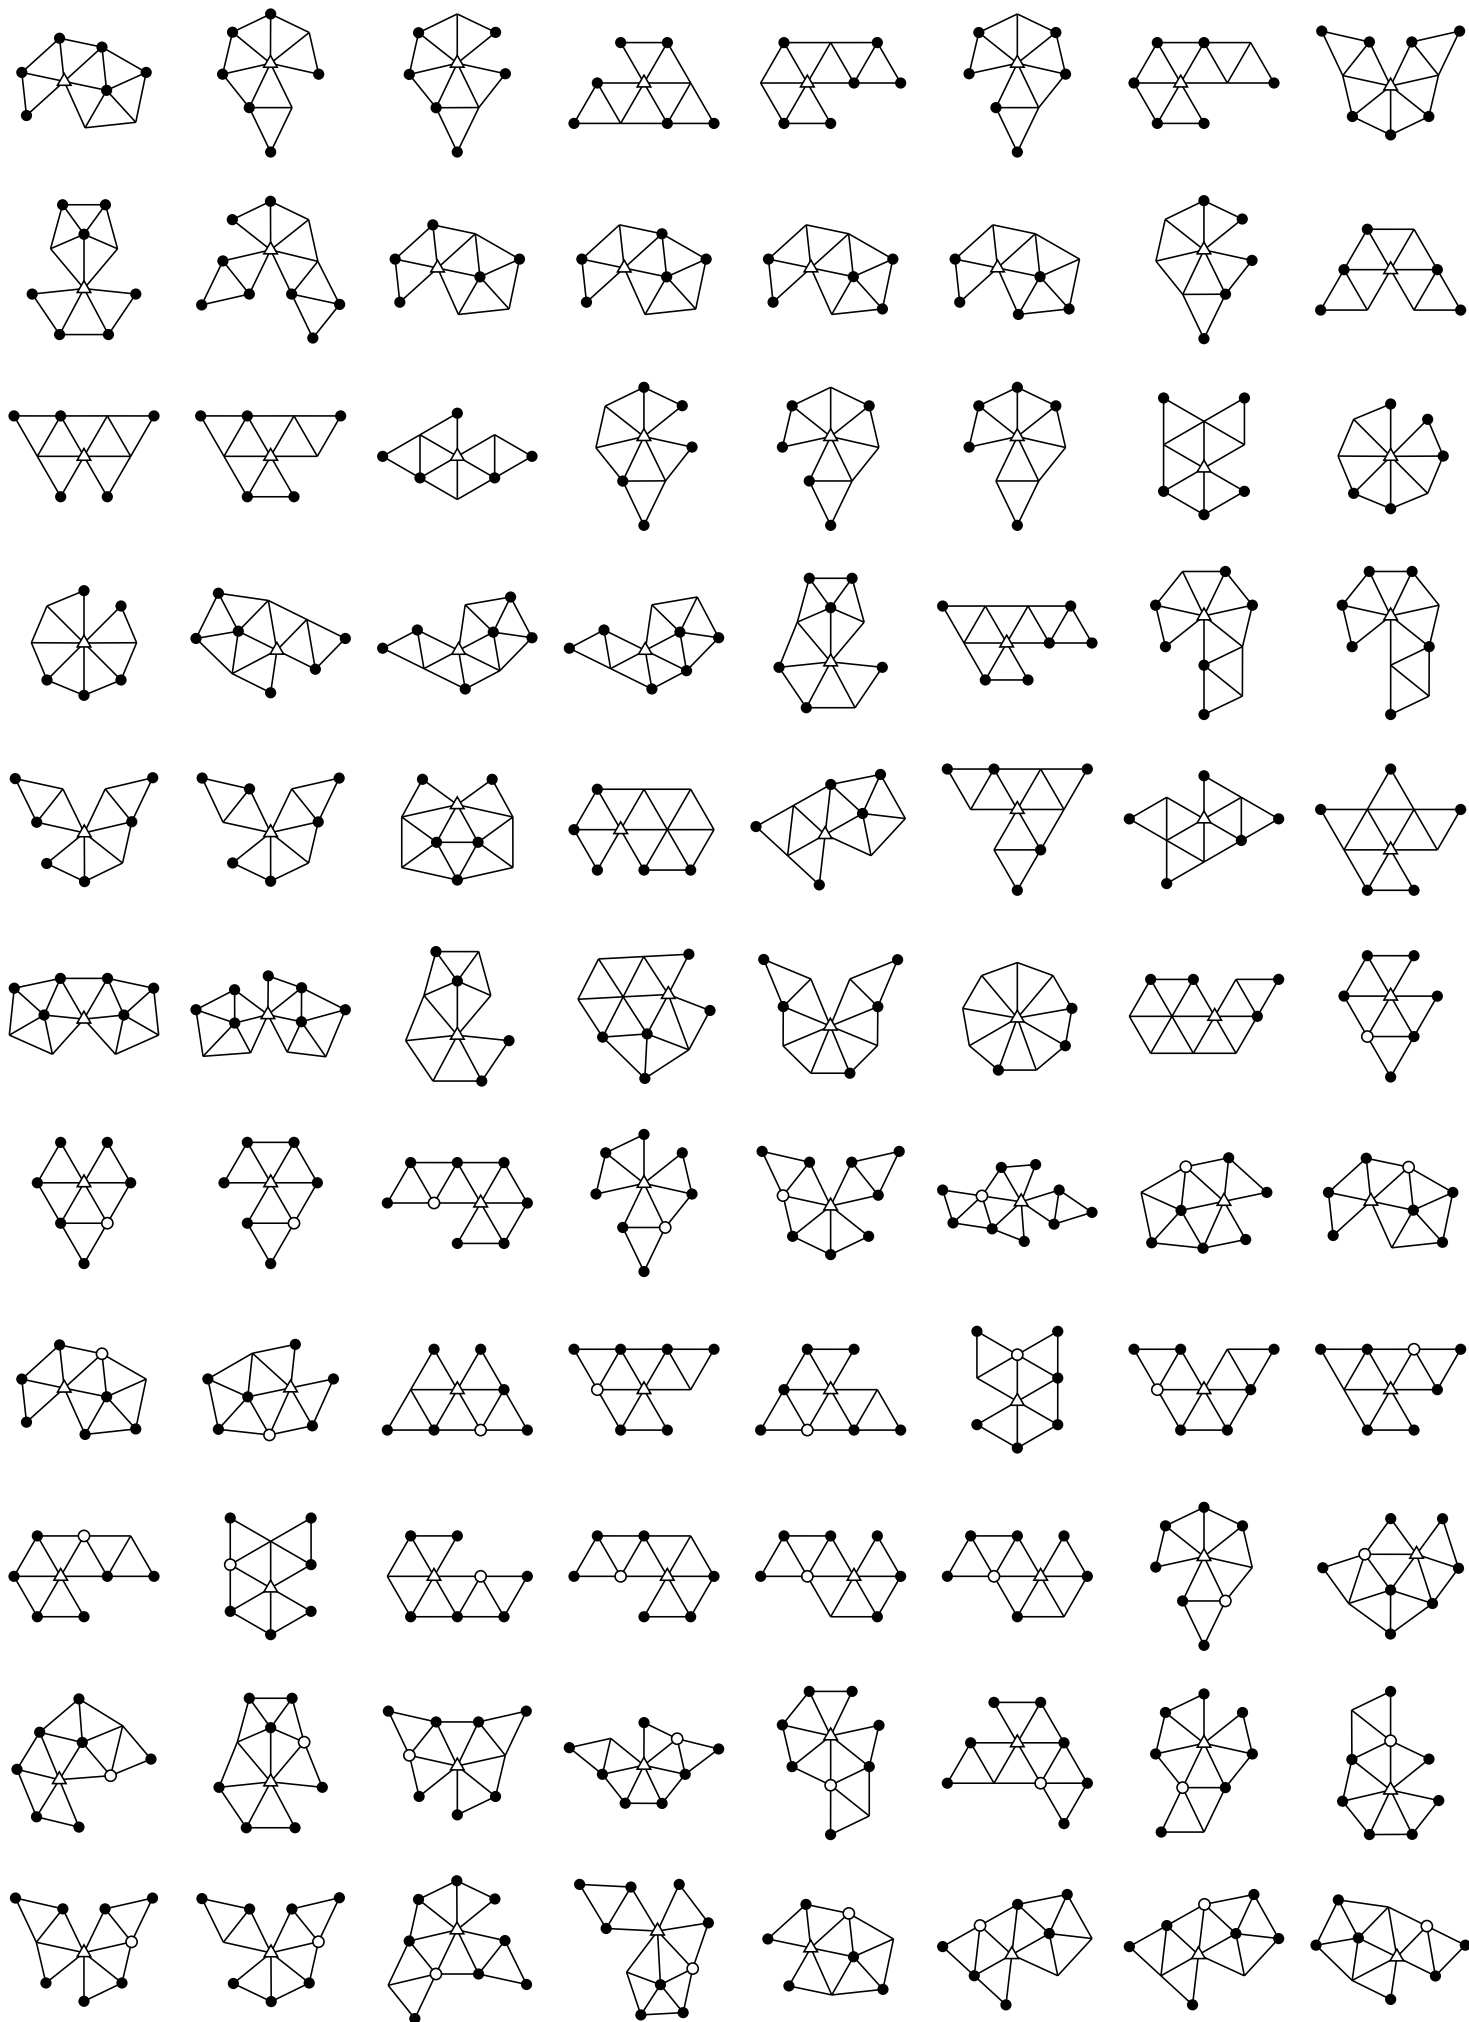

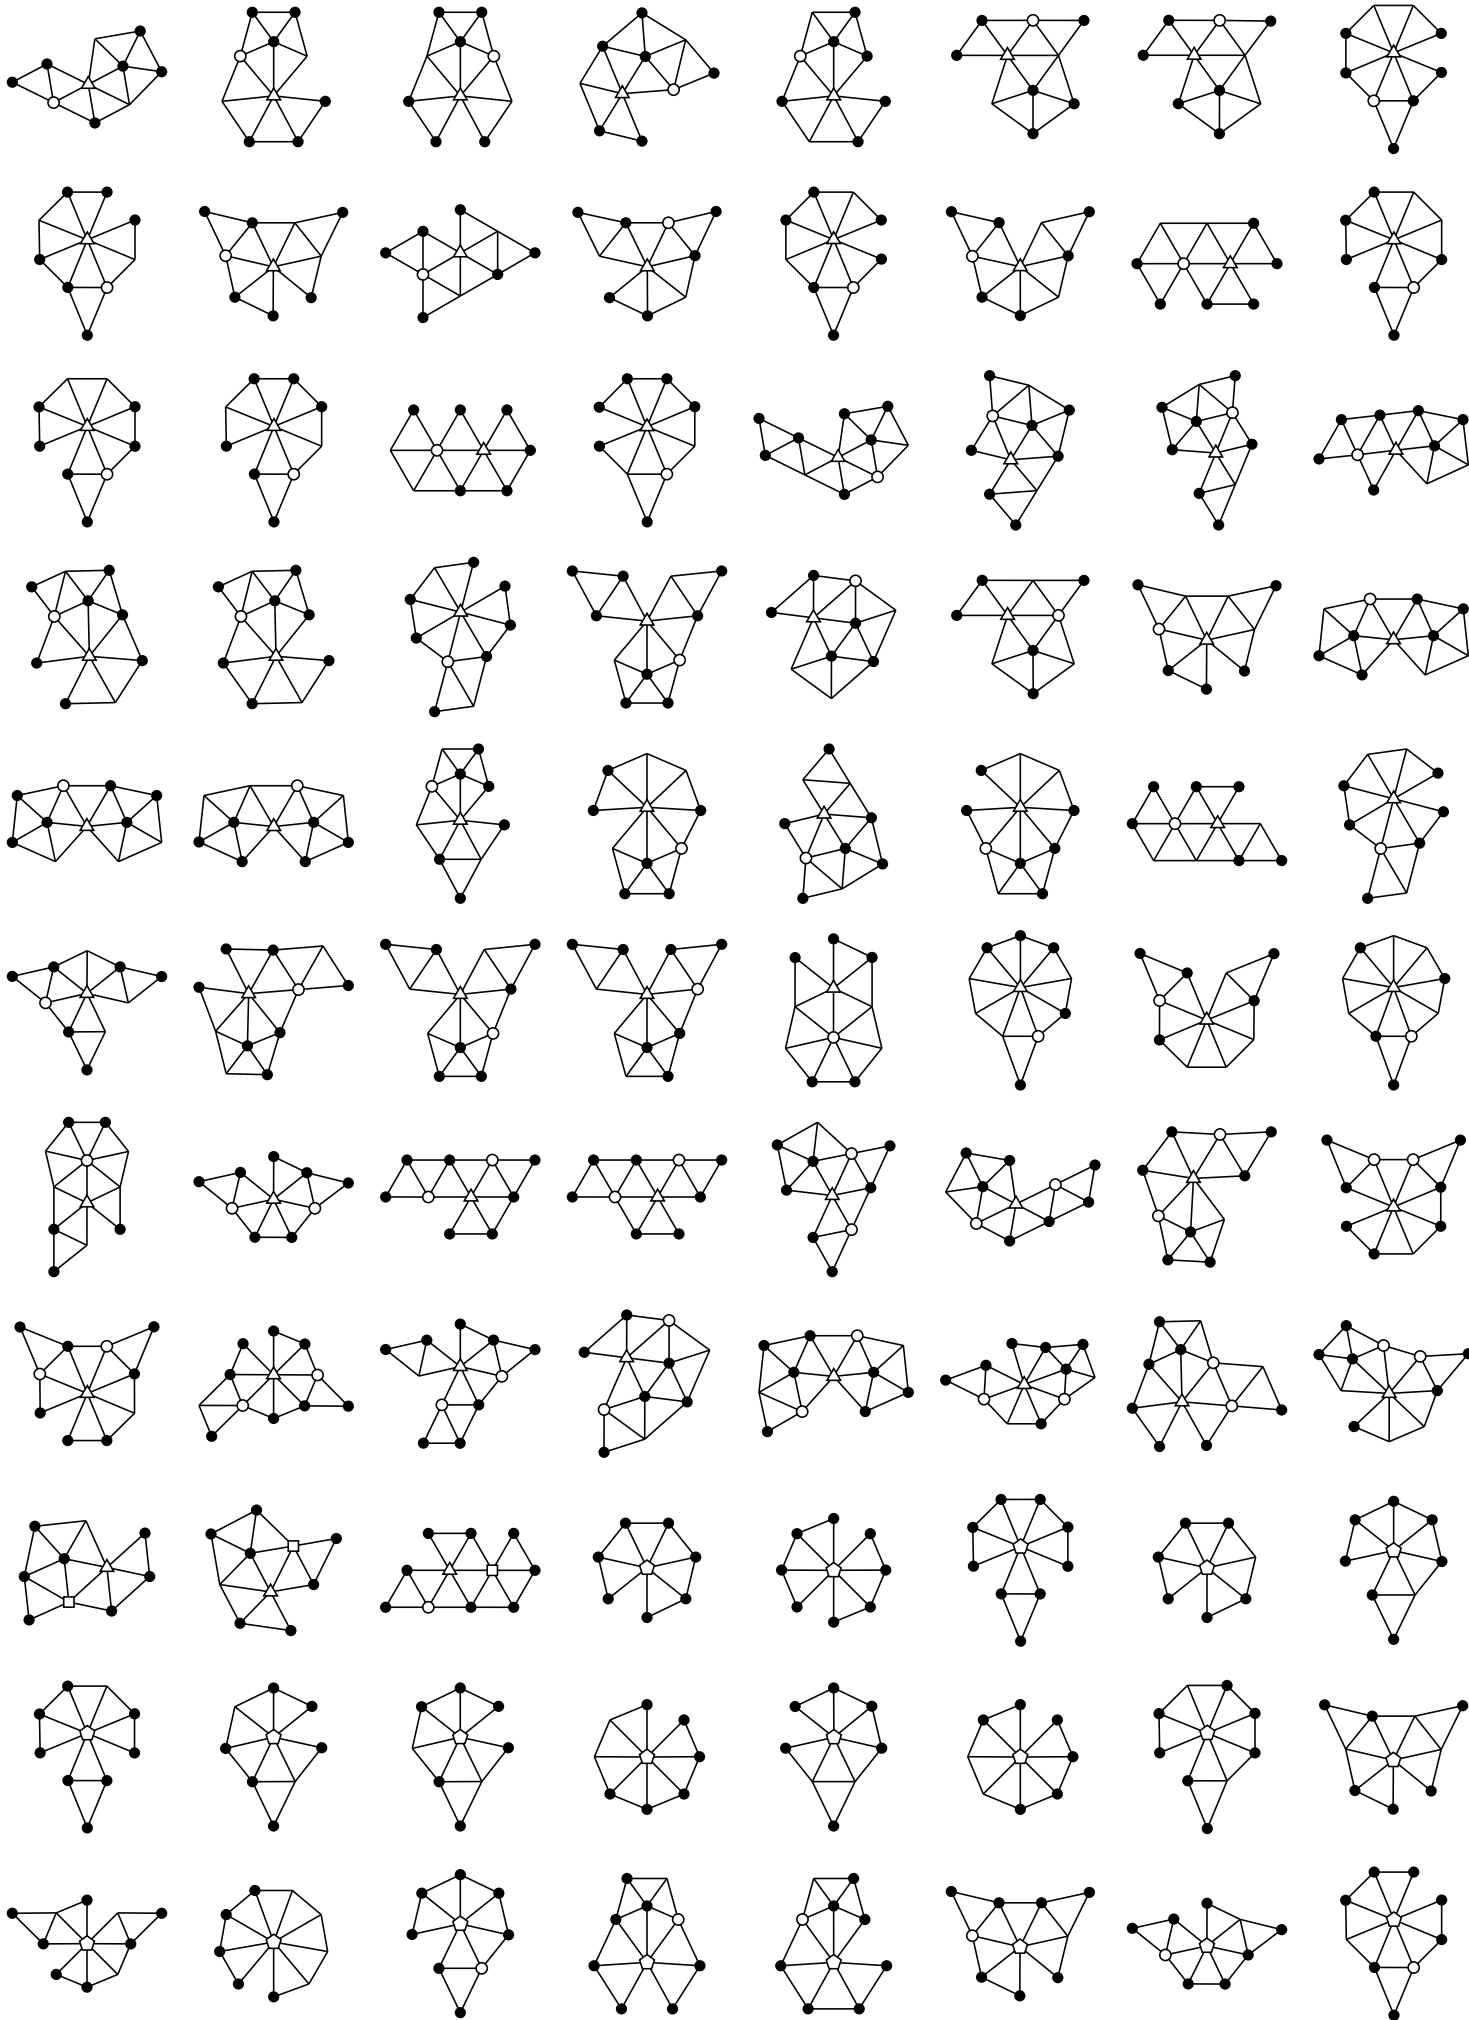



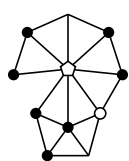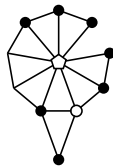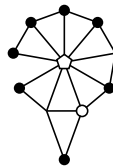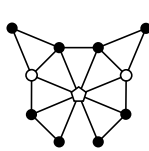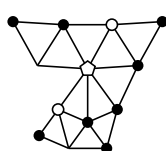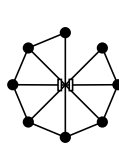

Supplement: Supplementary file 1 [file U_2822.pdf]
